# Supplementary material for: A computational framework for quantifying route diversification in road networks
Source: arXiv:2510.02582 ancillary file (2025-10-02)
Supplement: Supplementary file 1 [file Supplementary_Material.pdf]

# A computational framework for quantifying route diversification in road networks
# Supplementary Material

Giuliano Cornacchia, Luca Pappalardo, Mirco Nanni, Dino Pedreschi, Marta C. González

October 2, 2025

## Contents

**1 Supplementary Notes** **2**
Supplementary Note 1: parameter sensitivity . . . . . 2
Supplementary Note 2: DiverCity within cities . . . . . 2
Supplementary Note 3: $\mathcal{D}_C$ in grid and non-grid cities . . . . . 3
Supplementary Note 4: $\mathcal{D}_C$ and road network measures . . . . . 3
Supplementary Note 5: DiverCity and traffic congestion . . . . . 3
Supplementary Note 6: isolating the effects of mobility attractors . . . . . 5
Supplementary Note 7: DiverCity profiles of individual cities . . . . . 5

**2 Supplementary Figures** **7**

**3 Supplementary Tables** **49**

# 1 Supplementary Notes

## Supplementary Note 1: parameter sensitivity

The methodology for computing near-shortest routes, as described in the Methods section of the main article, relies on three key parameters that govern the generation and evaluation of alternative routes:

- $k$: The maximum number of alternative routes considered. Higher $k$ values allow for broader exploration of alternatives, enabling more diverse route options, while lower $k$ values focus on a smaller subset of paths.
- $p$: The penalization factor in the Path Penalization algorithm controls how strongly previously traversed edges are penalized. Low $p$ values keep alternatives near the shortest path, while high $p$ values promote greater deviation, though excessive penalization can result in impractical routes.
- $\epsilon$: The cost threshold $\epsilon$ sets the maximum allowable deviation from the optimal route, ensuring alternatives remain practical by balancing route diversity and efficiency.

In the analysis presented in the main article, we set $k = 10$, $p$=0.1, and $\epsilon = 30\%$. Here, we assess parameter sensitivity to confirm the robustness of our findings, ensuring that inter-city relationships (global distribution) and intra-city patterns (radial trends, including localized effects of attractors) remain consistent and are not artifacts of parameter choices. To evaluate parameter sensitivity, we varied one parameter at a time while keeping the others fixed to their default values:

- $k$: from 2 to 15.
- $p$: 0.05,0.1,0.2,0.30.
- $\epsilon$: from 10% to 50% in increments of 10%.

We avoided testing all parameter combinations, as certain configurations (e.g., $k$=2, $p$=0.05, $\epsilon = 10\%$) are overly restrictive, yielding very few viable near-shortest paths and failing to capture meaningful diversity. Varying one parameter at a time while keeping the others fixed ensures that the effects of each parameter on $\mathcal{D}_C$ are isolated and interpreted independently.

**Sensitivity to $k$** Varying $k$ while keeping other parameters fixed preserves the characteristic bell-shaped $\mathcal{D}_C$ distribution across cities (Figure S1), with consistent rankings, including the extremes (Mumbai and Tokyo). Similarly, trends in $\mathcal{D}_C$ with radial distance, such as the increase, plateau, and decrease near Rome's ring road, remain unchanged (Figure S2). The primary effect of $k$ is on the range of $\mathcal{D}(u, v)$, which scales from 0 to $k$, reflecting its impact on maximum diversification.

**Sensitivity to $p$** The impact of varying $p$ is illustrated in Figure S3 and Figure S4. The bell-shaped $\mathcal{D}_C D$ distribution across cities and the radial trends, including the decrease near Rome's ring road, remain consistent. Similarly to $k$, the primary change lies in the range of DiverCity: high $p$ values encourage greater route deviation, which can increase diversity, but if $p$ is too high, paths may deviate excessively, reducing DiverCity.

**Sensitivity to $\epsilon$** Figure S5 illustrates the effect varying $\epsilon$ on $\mathcal{D}_C$. Low $\epsilon$ values impose stricter constraints on near-shortest routes, leading to a significant reduction in $\mathcal{D}_C$, particularly noticeable for $\epsilon$=10% (see Figure S5). However, the overall trends in $\mathcal{D}_C$, including the bell-shaped distribution across cities and the trends with radius (Figure S6), remain consistent.

Our parameter sensitivity analysis demonstrates that while variations in $k$, $p$, and $\epsilon$ affect the absolute values of $\mathcal{D}_C$, the key trends and findings remain robust. The consistent inter-city rankings, bell-shaped distributions, and radius-dependent patterns confirm that the observed phenomena are intrinsic to the road networks and not driven by specific parameter settings for discovering alternative routes.

## Supplementary Note 2: DiverCity within cities

DiverCity is not uniformly distributed within a city. It tends to be low in the city center, averaging around 5 within the first kilometer, and increases sharply with distance from the center, stabilizing at approximately 7.5 beyond 10 km. In general, each city may exhibit unique intra-city variability due to factors such as geographical conformation, network structure, and the presence or placement of mobility attractors, which contribute to distinct patterns of DiverCity across urban areas.

The distribution of $\mathcal{D}(u, v)$ for each city (Figure S7) reveals a left-skewed distribution, with a peak around 8. However, the distribution also highlights variability among cities, indicating that some exhibit significantly different diversification patterns.

To explore this variability, we present the distribution of $\mathcal{D}(u, v)$ for each city (Figure S8). Cities display distinct levels of potential route diversification, with some achieving consistently high $\mathcal{D}(u, v)$ values across most of their

area (e.g., Tokyo, Osaka), while others exhibit lower and more constrained values (e.g., Mumbai, Rio de Janeiro). Moreover, cities with higher median $\mathcal{D}(u, v)$ values tend to exhibit lower variance, as measured by the interquartile range.

## Supplementary Note 3: $\mathcal{D}_C$ in grid and non-grid cities

To investigate the role of road network structure in shaping the availability and characteristics of alternative routes, we examine how different configurations influence route diversification. We adopt a widely used classification of urban road networks, distinguishing between grid and non-grid configurations. Grid cities feature street orientations aligned along a few dominant directions, such as orthogonal axes with four primary alignments. Non-grid configurations are further divided into two subtypes: radial networks, where roads converge toward or diverge from a central point, and organic networks, shaped by natural or historical constraints such as hills, rivers, or city walls, and developed without a unified design.

We classify each city as either grid or non-grid through a visual inspection of its road network structure (see Table 1). Among the 56 cities analyzed, the majority (34 cities) fall into the non-grid category, predominant in Europe and Asia. In contrast, grid configurations (22 cities) are more common in North America.

Figure S9a shows the distribution of $\mathcal{D}_C$ values by road network type. Grid cities exhibit higher and more stable $\mathcal{D}_C$ scores (7.68 $\pm$ 0.55) compared to non-grid cities (7.29 $\pm$ 0.79). This suggests that grid-like networks support greater potential route diversification, likely due to their uniform structure and regular intersections, which facilitate alternative paths of similar cost.

To quantify this, we calculated the time difference (in minutes) between the longest near-shortest routes (NSR) and the optimal route for each trip. Grid cities display a smaller average time difference (4.67 minutes) compared to non-grid cities (5.34 minutes) (See Figure S9b). This result highlights the efficiency of grid networks in offering alternatives that are competitive in cost, thereby enhancing their overall potential route diversification.

In summary, regular grid-like networks are associated with higher route diversification due to their ability to provide multiple alternative paths of comparable cost. In contrast, irregular networks, often found in older or geographically constrained cities, tend to offer fewer viable alternatives, reflecting their structural limitations.

## Supplementary Note 4: $\mathcal{D}_C$ and road network measures

The structural properties of road networks significantly influence their capacity to support a city's route diversification ($\mathcal{D}_C$). In this analysis, we examine the relationship between $\mathcal{D}_C$ and key network metrics, including total network length, intersection count, average street length, streets per node, and edge circuity.

**Network Length** Figure S10a shows a strong positive correlation ($r = 0.561$, $\rho = 0.652$) between total network length and $\mathcal{D}_C$. Cities with more extensive road networks provide greater opportunities for route diversification, likely due to the increased number of available paths and alternatives.

**Average Street Length** As shown in Figure S10b, there is a weak negative correlation ($r = -0.078$, $\rho = -0.169$) between $\mathcal{D}_C$ and average street length. Shorter streets likely contribute to increased connectivity and route choices, but the weak relationship suggests that other factors may play a more significant role.

**Streets Per Node** The relationship between streets per node and $\mathcal{D}_C$ is modestly positive ($r = 0.214$, $\rho = 0.278$), as shown in Figure S10c. Cities with higher connectivity at intersections tend to facilitate route diversification by increasing the number of decision points within the network.

**Intersection Count** Figure S10d illustrates a strong positive correlation ($r = 0.431$, $\rho = 0.488$) between intersection count and $\mathcal{D}_C$. A higher number of intersections creates more opportunities for alternative routing, contributing to greater potential diversification.

**Edge Circuity** Finally, we analyze the edge circuity, i.e., the ratio of edge length to the straight-line distance between endpoints, which shows a negative correlation with $\mathcal{D}_C$ ($r = -0.297$, $\rho = -0.415$), as shown in Figure S10e. Cities with more winding or indirect roads tend to have lower route diversification.

In summary, extensive networks with high intersection density and shorter, more direct streets tend to exhibit higher $\mathcal{D}_C$. Conversely, features like long average street lengths and high edge circuity are associated with reduced potential diversification.

## Supplementary Note 5: DiverCity and traffic congestion

In the main text, we introduce the congestion index ($CI$), defined as $CI(u, v) = \frac{t_{\text{peak}} - t_{\text{off-peak}}}{dist(u,v)}$, where $t_{\text{peak}}$ and $t_{\text{off-peak}}$ are the estimated travel times for a given trip $(u, v)$ under peak and off-peak traffic conditions, respectively, and

$\text{dist}(u, v)$ is the straight-line distance between origin and destination. The congestion index, expressed in seconds per kilometre, provides a normalized measure of trip-level congestion, capturing the extent to which peak-hour travel times exceed free-flow conditions. Higher $CI$ values indicate more severe congestion. This supplementary note offers additional details on its computation and presents further analyses supporting its interpretability and connection to DiverCity.

**a. Travel Time Retrieval** Travel times are retrieved from TomTom's routing API by setting the departure time to 8:00 AM and 2:00 AM local time, corresponding to peak and off-peak traffic conditions, respectively. To ensure consistency and avoid the influence of unpredictable events (e.g., accidents or temporary road closures), we specify a departure date in the future, which triggers the API to return travel times based on historical traffic patterns rather than live conditions. The API provides the expected travel time for the optimal route at each specified time. This procedure is applied across all cities. Full API documentation is available at: `https://developer.tomtom.com/routing-api`.

**b. Distribution of the Congestion Index** We compute the Congestion Index over a representative subset of up to 2,142 origin-destination (OD) pairs per city. These are extracted using the radial sampling used in the main analysis, with nodes located at distances of 2, 4, 6, 8, 10, 12, and 15 km from the city center, spaced every 20°. This design ensures coverage from central to peripheral areas while keeping the number of required API calls tractable. The 15 km cutoff reflects the distance at which DiverCity values plateau in most cities. Figure S11 shows the global and city-level distributions of CI values. While most trips experience moderate or low congestion (global median: 52.05 s/km; mean: 59.56 s/km), the distribution is right-skewed, with a long tail extending beyond 150 s/km. This tail corresponds to trips that incur substantial delays relative to free-flow conditions. City-level distributions reveal heterogeneity in both central tendency and spread, reflecting the varying degrees of congestion stress across urban systems. These differences motivate our use of city-specific percentile thresholds to identify the most congested trips.

**c. Correlation between DiverCity and $CI$** To examine the relationship between DiverCity and $CI$, we compute their Pearson correlation across percentile bins of the $CI$ distribution. As shown in Figure S12, the correlation is slightly positive in the lowest percentiles, remains weak or negligible across most of the distribution, and becomes increasingly negative in the upper tail. This indicates that route diversification, i.e., DiverCity, plays a more significant role under severe traffic conditions.

The weak positive correlation in the low-congestion $CI$ range reflects that DiverCity has little explanatory value when traffic is free-flowing. In this regime, high-DiverCity trips may show marginally higher $CI$ if they involve central or popular OD pairs, while low-DiverCity trips can also occur on seldom-used roads that rarely experience delays. This mix explains the slight positive correlation observed in the low-congestion levels.

In contrast, for trips above the 95th percentile of the city-specific $CI$ distribution, the correlation reaches $r = -0.227$ and $\rho = -0.218$, indicating that trips with limited and spatially overlapping routing alternatives, i.e., low DiverCity, are more prone to severe congestion. Under such conditions, the absence of viable alternative routes concentrates traffic on a small set of corridors, amplifying delays when these links become saturated. Conversely, trips with higher DiverCity benefit from the flexibility to redistribute traffic across multiple, loosely overlapping routes, mitigating the impact of high-traffic conditions.

To verify that this pattern is not a statistical artifact, we construct a null model in which DiverCity values are randomly reassigned across trips. As shown in Figure S13, the null model yields correlations near zero across all percentile ranges, further confirming that the observed relationship is not due to random variation. Based on these findings, we define *congested trips* as those falling within the top 5% of the CI distribution in each city.

**d. DiverCity in Congested vs Non-Congested Trips** We further examine the relationship between DiverCity and congestion by comparing DiverCity values for trips classified as congested (top 5% of each city's $CI$ distribution) and those that are not. At the global level, the difference is statistically significant: congested trips exhibit lower DiverCity, with an average of 5.93, compared to 6.97 for non-congested ones ($p < 0.05$, Welch's t-test). At the city level, we compute the relative difference $\Delta\mathcal{D}$, which expresses the percentage increase in DiverCity between non-congested and congested trips within the same city. Figure S14 shows the distribution of $\Delta\mathcal{D}$ across cities. On average, DiverCity is 17.88% higher in non-congested trips. The trend is robust: 43 out of 56 cities (76.79%) exhibit statistically significant differences ($p < 0.05$, Welch's t-test), and only two cities (Istanbul and Barcelona) show a negative value.

These results demonstrate that DiverCity is not only globally lower in congested trips but also consistently lower across diverse urban contexts. This further supports its role as a structural indicator of routing flexibility and resilience to traffic congestion.

An illustrative example is shown in Figure S15, which compares two OD pairs in London with identical straight-line distances (5 km). The trip with lower DiverCity falls in the top 5% of the city's $CI$ distribution and exhibits markedly higher congestion.

**e. DiverCity Differences Across Attractor Usage** To test whether DiverCity's difference in congested and non-congested trips holds independently of attractor usage, we stratify trips into deciles based on the share of their fastest path that overlaps with attractor roads. Within each decile, we compare DiverCity values between congested and non-congested trips. As shown in Figure S16, DiverCity remains consistently higher for non-congested trips across all levels of attractor reliance. All group-wise differences are statistically significant ($p < 0.05$, Welch's t-test). These results indicate that DiverCity captures structural aspects of routing flexibility that are not explained by attractor usage alone. In practice, even among trips that make similar use of major roads, those that are congested exhibit lower DiverCity than non-congested ones.

## Supplementary Note 6: isolating the effects of mobility attractors

To analyze the impact of mobility attractors on route diversification in a controlled environment, we employ a regular lattice grid $L$ spanning $60 \times 60$ km, consistent with the scale used in real-city analyses. Each road segment in $L$ is 500 meters long with a default speed limit of 50 km/h. Mobility attractors are introduced into $L$ as "squares" centered at $L$'s midpoint, with a side length of $2d$ and a speed limit of 100 km/h.

**a. Relationship Between Attractor Position and DiverCity Reduction** Introducing a mobility attractor $A_d$ at varying distances $d$ from the lattice center reduces $\mathcal{D}_L(u, v)$ in its vicinity. Figure S17 shows the spatial distribution of $\mathcal{D}_L(u, v)$ for attractors placed at varying distances ($d$) from the center. The results reveal a consistent pattern: DiverCity reductions occur in regions near the attractor. In addition to visual inspection, we also quantify this observation by analyzing the relationship between $d$ and the distance at which $\mathcal{D}_L(u, v)$ reaches its minimum value (S18). The two quantities exhibit a strong correlation ($r = 0.995$, $\rho = 0.998$), and the trend is well-fitted ($R^2$ of 0.995) by a linear function $y = 1.08x + 0.61$. The slope (1.08) close to one indicates that the reduction zone is closely aligned with the attractor's position, with only a slight additional spread. This confirms that the introduction of an attractor suppresses DiverCity locally, with the suppression zone centered around the attractor.

**b. Extent of DiverCity Suppression** We also investigated the factors driving the extent of DiverCity suppression, measured as the minimum $\mathcal{D}_L(u, v)$, by analyzing how the minimum changes with the attractor's speed and its distance $d$ from $L$'s center. We varied the attractor speed from 60 to 130 km/h (default: 100 km/h) and restricted the analysis to $r >$2 km, avoiding the natural DiverCity low near the center from being misidentified as the global minimum. As shown in Figure S19, the minimum $\mathcal{D}_L(u, v)$, is independent of the attractor's distance $d$ from $L$'s center, except near the lattice boundary (r $\approx$ 30 km), where the suppression zone partially extends beyond the grid, preventing DiverCity from fully decreasing. The key driver of the suppression is the attractor's speed limit: higher speeds consistently lower the minimum $\mathcal{D}_L(u, v)$, confirming that faster attractors amplify the suppressive effect.

**c. Interplay with a Second Attractor** We further explore the impact of introducing a second attractor $B_{d+\delta}$ at an offset $\delta$ from $A_d$. Figure S20 presents the DiverCity profiles for varying offsets ($\delta$) and attractor speeds. The benefit of a second attractor, measured by the area under the curve (AUC) difference between $\mathcal{D}_L(u, v)$ with two and one attractors, diminishes linearly as $\delta$ increases (Figure S20). Higher-speed attractors maintain slightly greater benefits. The second attractor provides limited benefits near the center but becomes more effective at greater distances. Notably, for $r > 18$ km, its introduction is consistently beneficial, except for low speeds (<70 km/h). Figure S21 exemplifies these effects for an attractor at 10 km and varying offsets for the second attractor. DiverCity increases when the second attractor is located near the first one. However, as the offset grows, the suppression zones from both attractors create two distinct reductions, with the second reduction lagging behind the second attractor's position for large offsets.

**d. Larger attractor configurations** To extend the analysis on mobility attractors, we evaluate the impact of introducing a third attractor into the grid. Figure S21 illustrates the AUC of $\mathcal{D}_L(u, v)$ for two base configurations: one with the first attractor positioned at 10 km from the center (Figure S22a) and the other at 15 km (Figure S22b), with two additional attractors placed at varying offsets. When the offsets between attractors are minimal (i.e., all three attractors are closely clustered), the AUC is maximized, suggesting enhanced potential route diversification. This confirms that clustering attractors can mitigate the localized suppression effect caused by a single attractor. As the offsets of the second and third attractors increase, the AUC decreases. This is due to the formation of distinct, non-overlapping suppression zones created by widely spaced attractors, which reduce the overall potential for route diversification across the grid. Notably, the configuration with the first attractor at 15 km (Figure S22b) consistently achieves higher AUC values than the configuration with the first attractor at 10 km (Figure S22a). This supports the observation that positioning the initial attractor farther from the grid's center yields greater benefits in terms of route diversification.

## Supplementary Note 7: DiverCity profiles of individual cities

In this supplementary note, we provide a comprehensive overview of each city's DiverCity characteristics, supported by a dedicated plot for every city (Figures S24–S79). Each plot includes the distribution of $\mathcal{D}(u, v)$, highlighting

intra-city variability, $\mathcal{D}(u,v)$ as a function of radial distance from the city center, the increase in DiverCity ($\mathcal{D}_C$) as a function of attractor speed reduction, the increase in travel time as a function of attractor speed reduction, and the spatial distribution of $\mathcal{D}(u,v)$ across the city, providing a geographical perspective on route diversification within urban areas. We provide an interactive online platform (https://divercitymaps.github.io) to visualize the spatial distribution of DiverCity across all considered cities.

The spatial distribution maps consistently confirm that low $\mathcal{D}(u,v)$ values (lighter regions) cluster near mobility attractors. These attractors act as dominant elements that suppress DiverCity by attracting and concentrating traffic. While Rome (Figure S67) and its ring road attractor, which suppresses DiverCity near its perimeter, are highlighted as a key example in the main article, this pattern is not unique to Rome. Similar patterns are observed in other cities, such as Amsterdam (Figure S24), Beijing (S28), Berlin (Figure S29), Dallas (Figure S37), Houston (S43), London (Figure S51), Milan (Figure S57), Moscow (S58), Paris (Figure S64), Santiago (Figure S69), Seoul (Figure S71), and Washington DC (Figure S79).

Some cities lack fully enclosed ring road attractors due to geographical constraints, such as their coastal locations. Instead, these cities often feature semi-ring or linear attractor configurations. Examples include Boston (Figure S31), Buenos Aires (S33), Chicago (Figure S36), Dubai (Figure S40), Jakarta (S45), Karachi (Figure S46), and Melbourne (S55). Although these configurations are not fully closed, their impact on DiverCity is comparable to that of traditional ring roads, with noticeable clustering of low $\mathcal{D}(u,v)$ values near these attractors. This emphasizes that the observed effect is determined by the road's function as a mobility attractor rather than its specific shape.

Finally, Table S1 provides a recap of all the computed metrics for each city.

## 2 Supplementary Figures

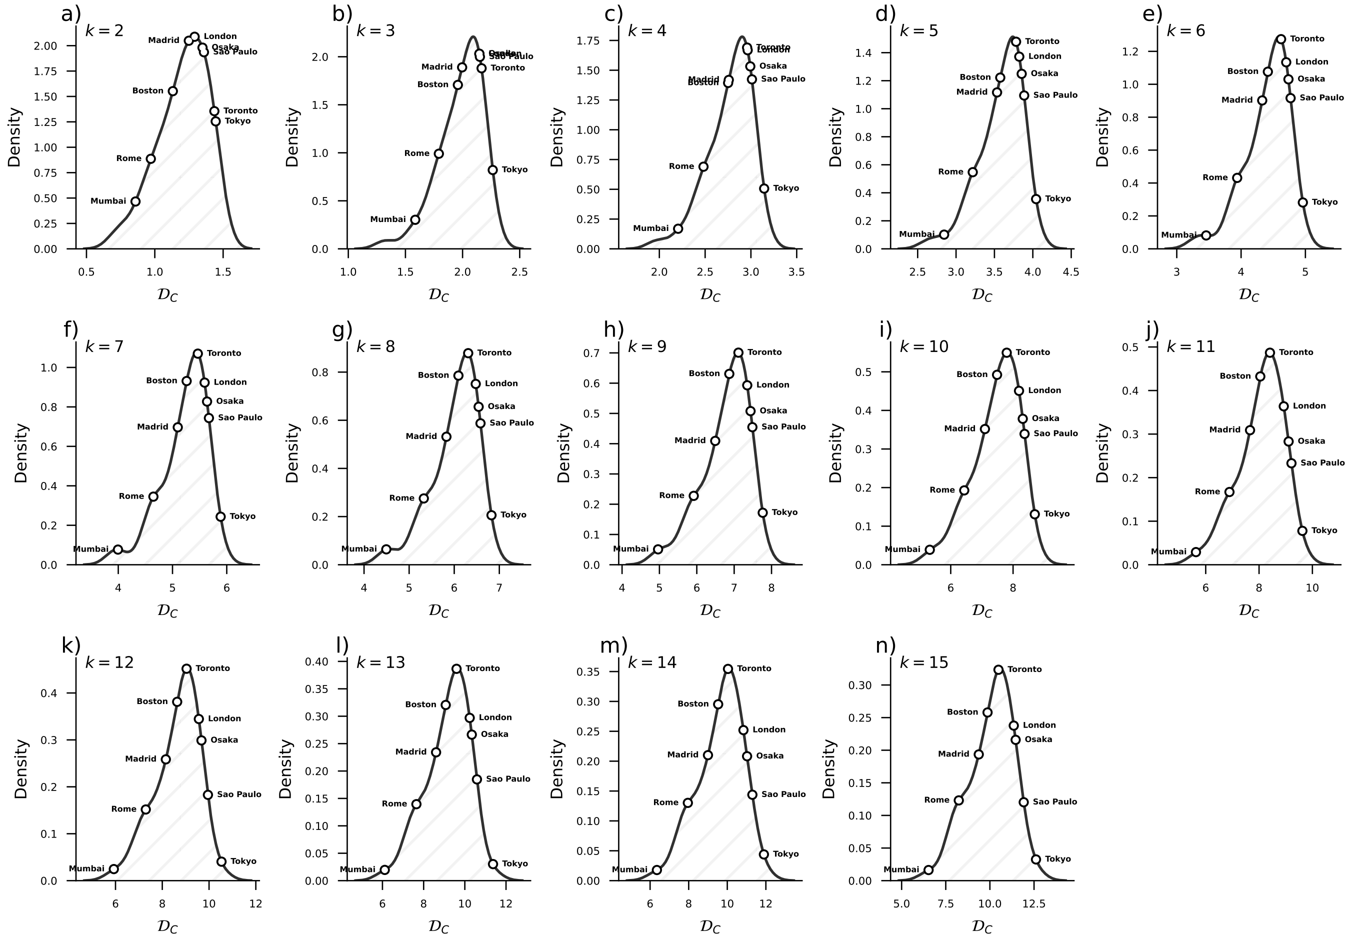


Figure S1: **Distribution of the median DiverCity ($\mathcal{D}_C$) for varying $k$.** The plot shows the distribution of $\mathcal{D}_C$ across all 56 cities for different values of $k$. Default parameters: $p = 0.1$, $\epsilon = 30\%$.

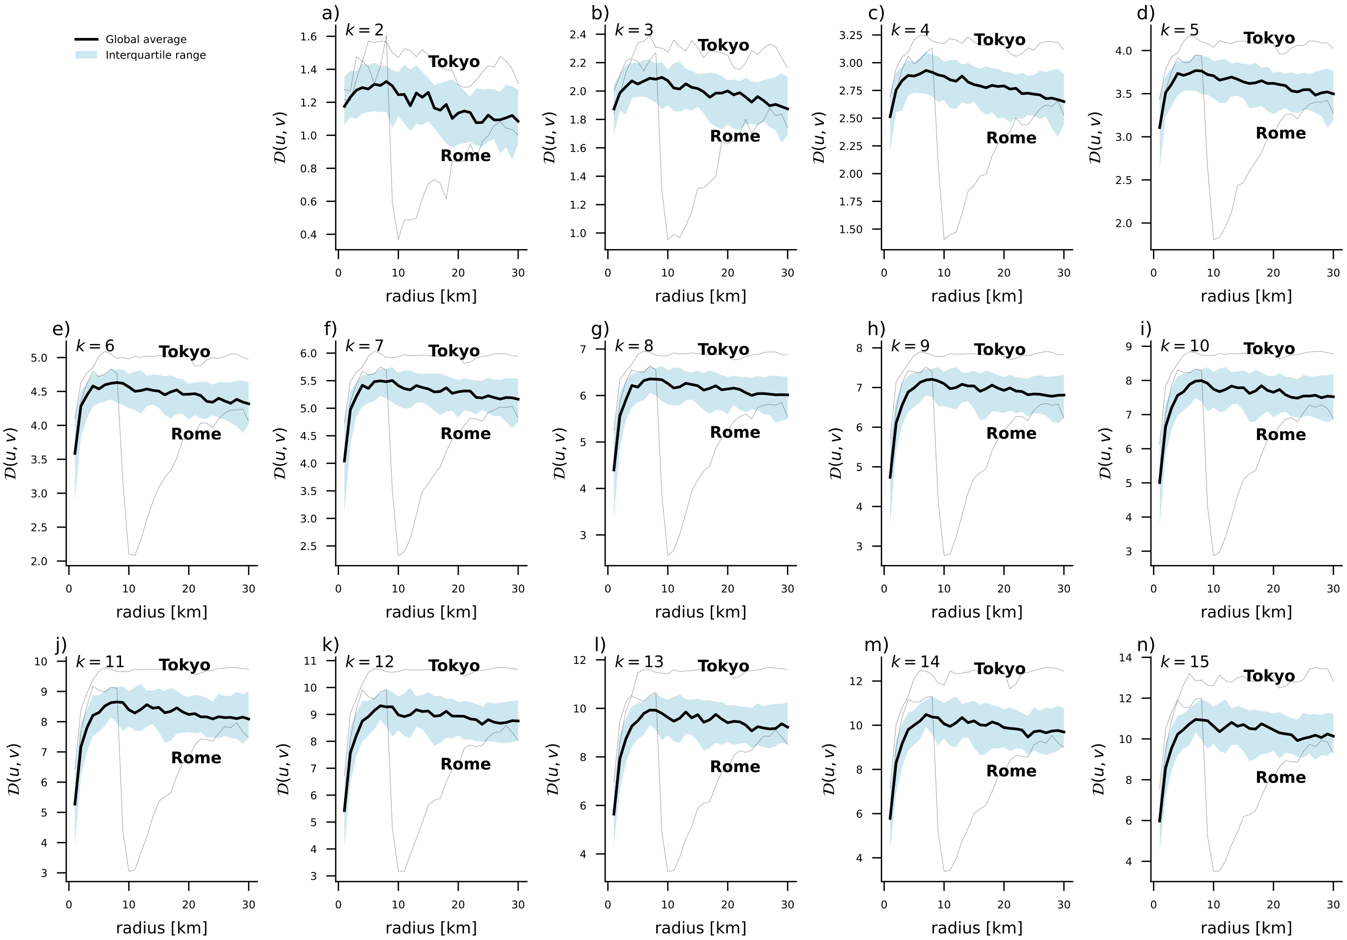


Figure S2: **DiverCity ($\mathcal{D}_C$) for trips at different radial distances for varying $k$.** The figure illustrates $\mathcal{D}_C$ as a function of radial distance for different $k$ values across all 56 cities. Default parameters: $p = 0.1$, $\epsilon = 30\%$.

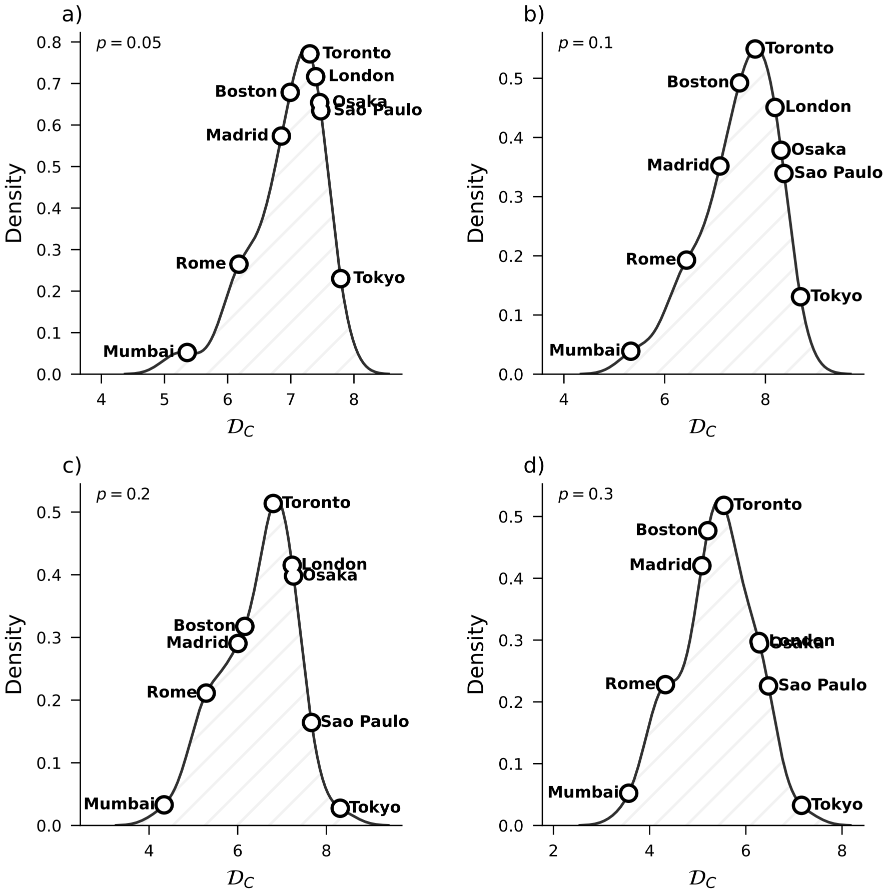


Figure S3: **Distribution of the median DiverCity ($\mathcal{D}_C$) for varying $p$.** The plot shows the distribution of $\mathcal{D}_C$ across all 56 cities for different values of $p$. Default parameters: $k = 10$, $\epsilon = 30\%$.

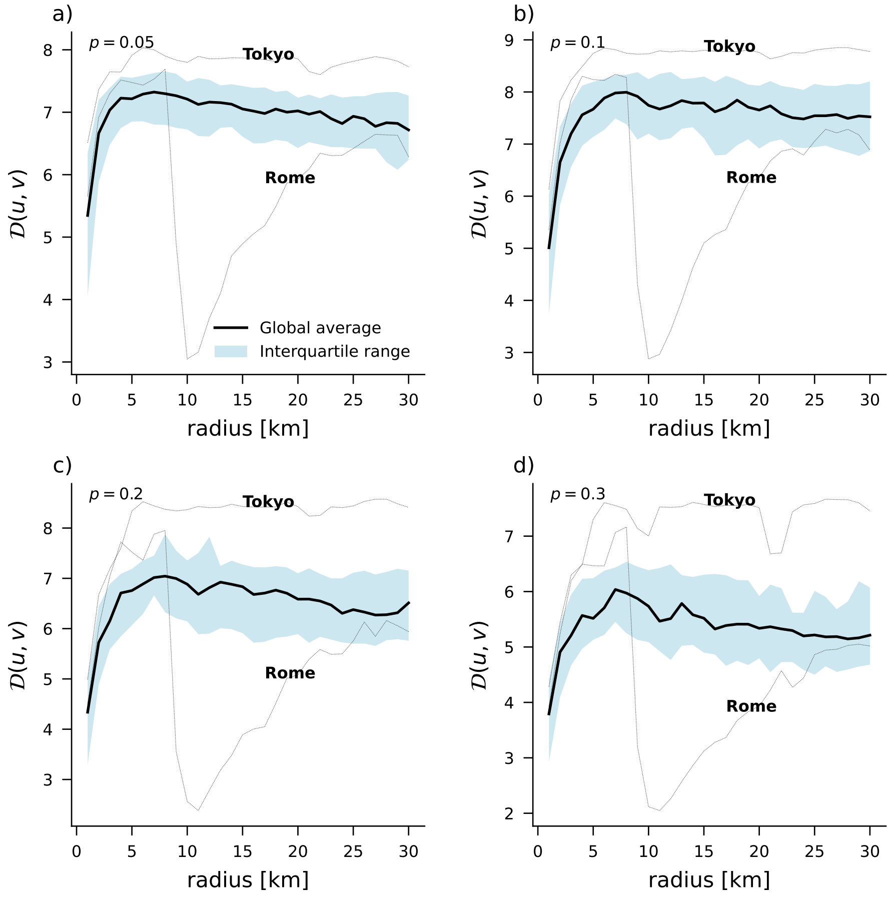


Figure S4: **DiverCity ($\mathcal{D}_C$) for trips at different radial distances for varying $p$.** The figure illustrates $\mathcal{D}_C$ as a function of radial distance for different $p$ values across all 56 cities. Default parameters: $k = 10$, $\epsilon = 30\%$.

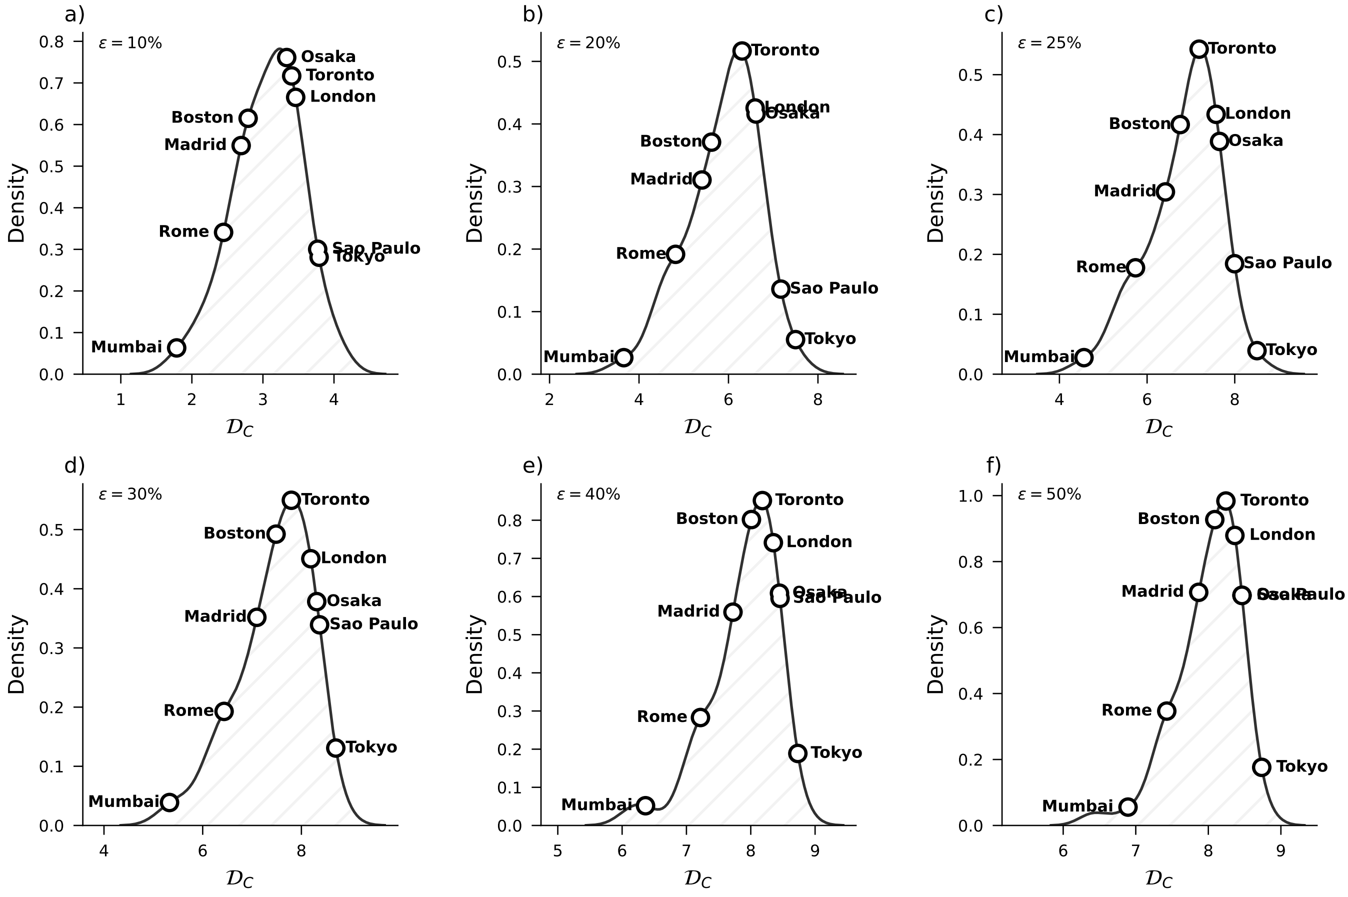


Figure S5: **Distribution of the median DiverCity ($\mathcal{D}_C$) for varying $\epsilon$.** The plot shows the distribution of $\mathcal{D}_C$ across all 56 cities for different values of $\epsilon$. Default parameters: $k = 10$, $p = 0.1$.

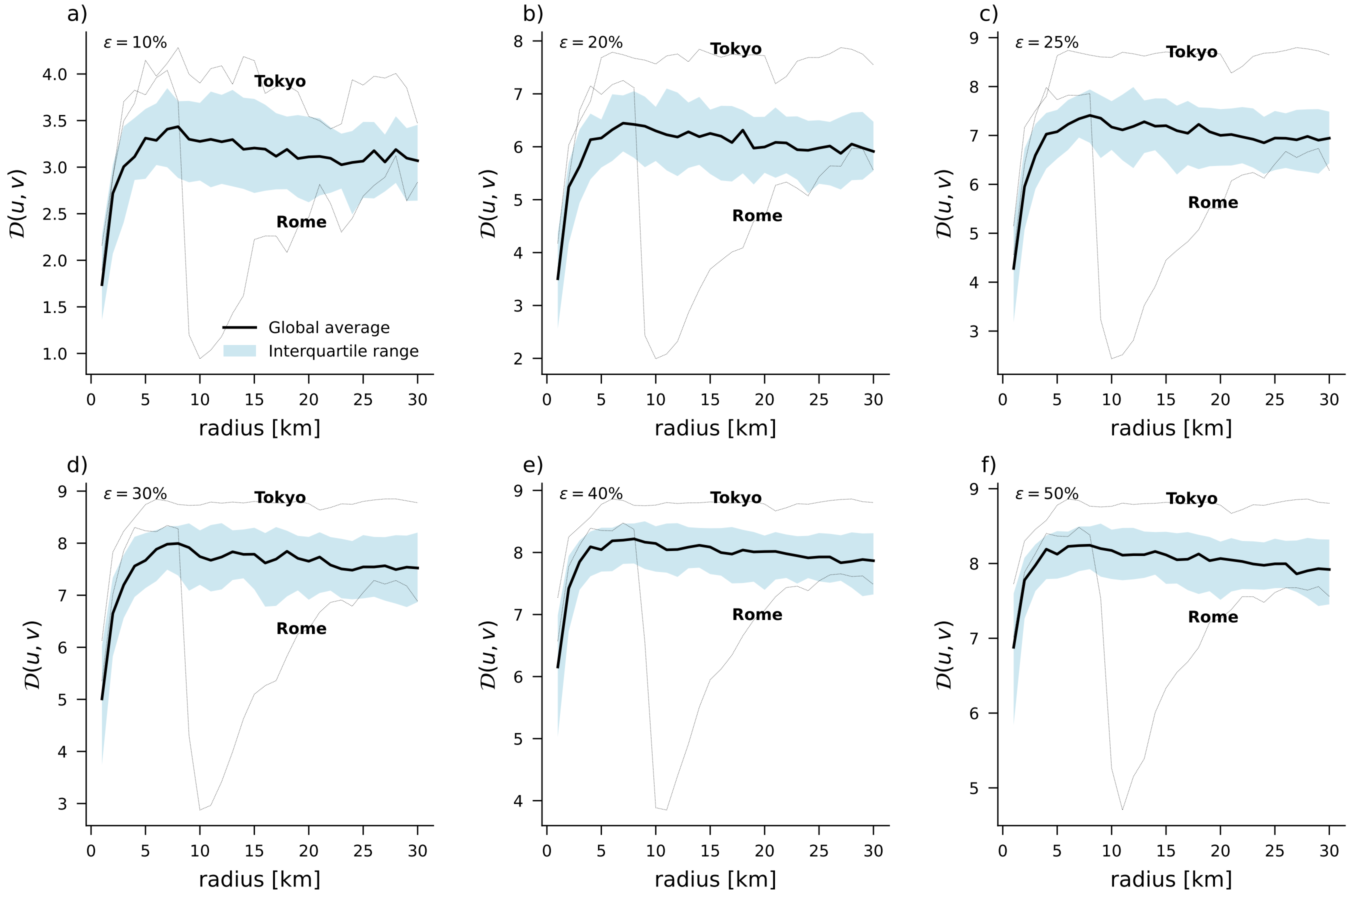


Figure S6: **DiverCity ($\mathcal{D}_C$) for trips at different radial distances for varying $\epsilon$.** The figure illustrates $\mathcal{D}_C$ as a function of radial distance for different $\epsilon$ values across all 56 cities. Default parameters: $k = 10$, $p = 0.1$.

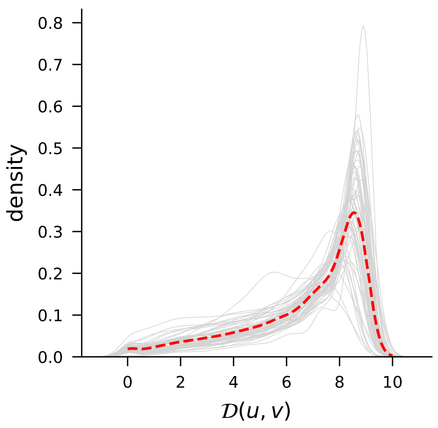


Figure S7: **Kernel density estimate (KDE) of DiverCity ($\mathcal{D}(u, v)$) across cities.** The distribution of $\mathcal{D}(u, v)$ for all cities (grey lines) and the global average (red dashed line).

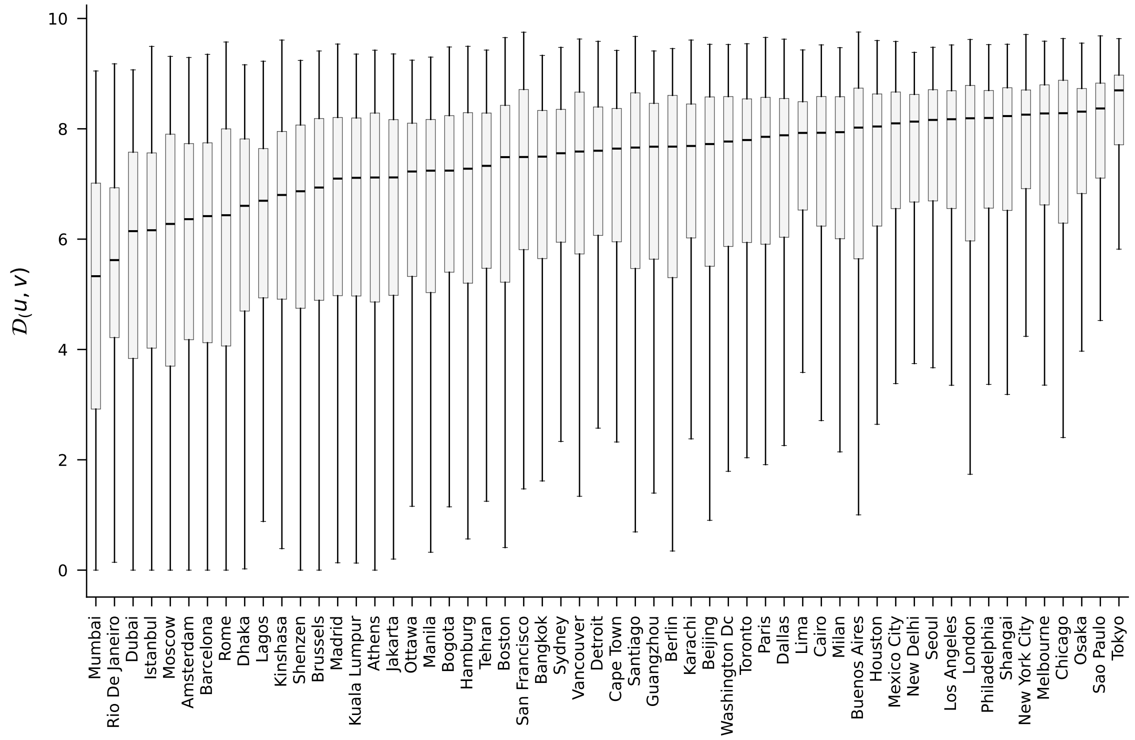


Figure S8: **Boxplots of DiverCity ($\mathcal{D}(u,v)$) for individual cities.** The boxplots illustrate the distribution of $\mathcal{D}(u,v)$ for each city. Cities such as Tokyo and Osaka exhibit high median $\mathcal{D}(u,v)$ values with low variance, while cities like Mumbai and Rio de Janeiro show lower medians and greater disparities.

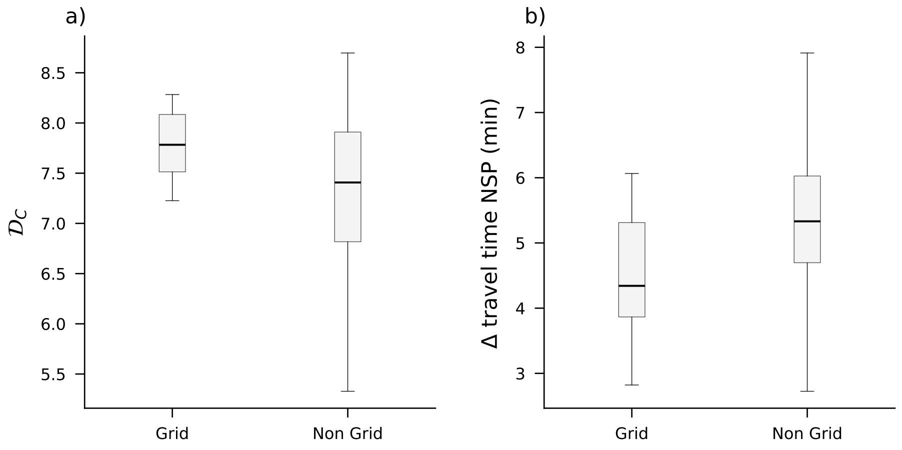


Figure S9: **DiverCity and Mobility Attractors.** (a) Distribution of $\mathcal{D}_C$ values for grid and non-grid cities. Grid cities exhibit higher and more stable $\mathcal{D}_C$ scores compared to non-grid cities, suggesting that grid-like networks support greater route diversification. (b) Time difference ($\Delta$ travel time) between the longest near-shortest route (NSR) and the optimal route for grid and non-grid cities. Grid cities show smaller average time differences, highlighting their efficiency in offering alternative routes that are competitive in cost.

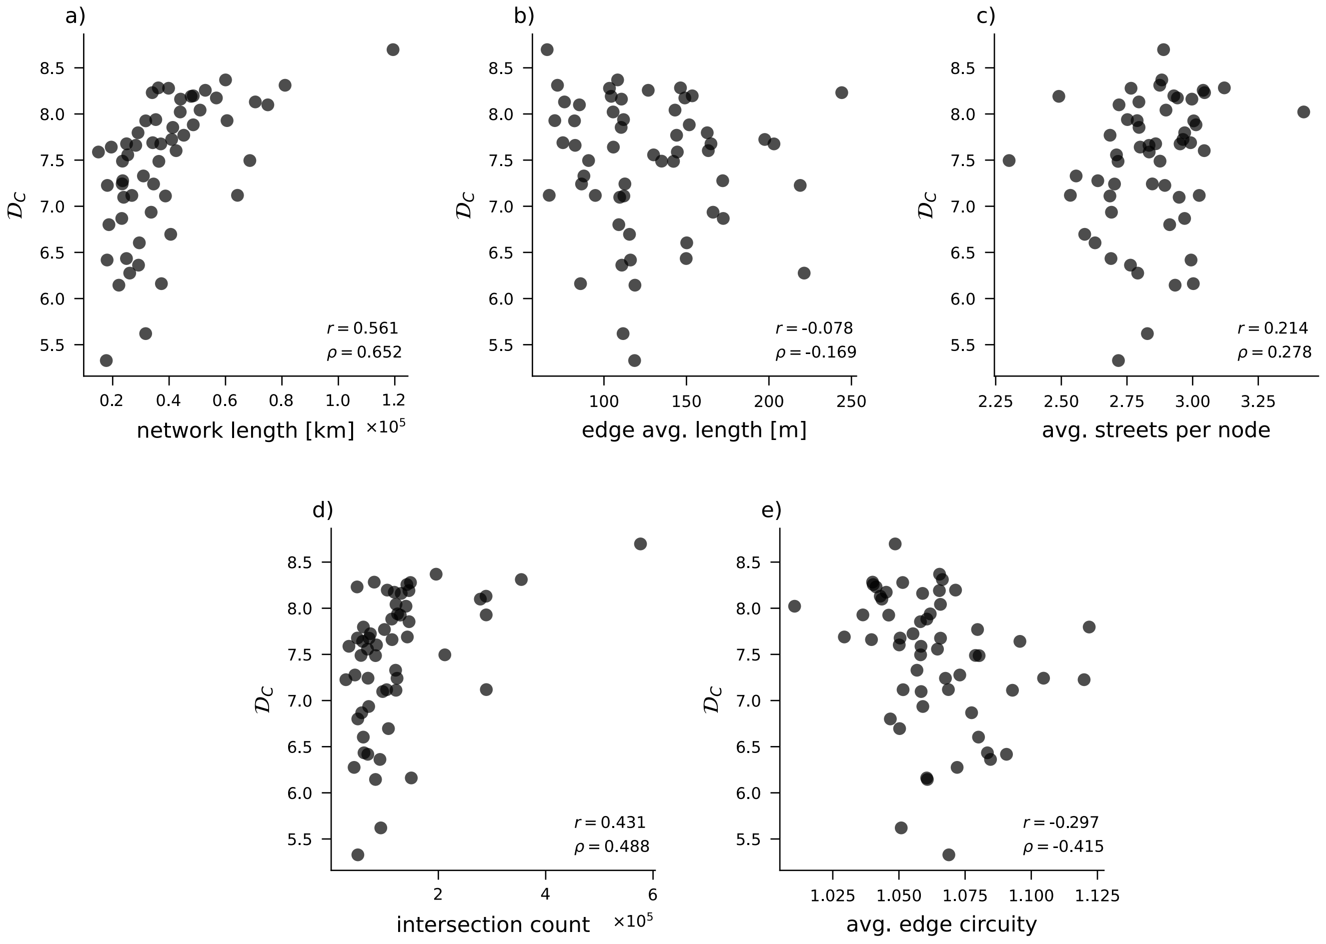


Figure S10: **Relationship between DiverCity ($\mathcal{D}_C$) and road network properties.** (a) $\mathcal{D}_C$ as a function of total network length. (b) $\mathcal{D}_C$ as a function of average street length. (c) $\mathcal{D}_C$ as a function of streets per node. (d) $\mathcal{D}_C$ as a function of intersection count. (e) $\mathcal{D}_C$ as a function of edge circuity.

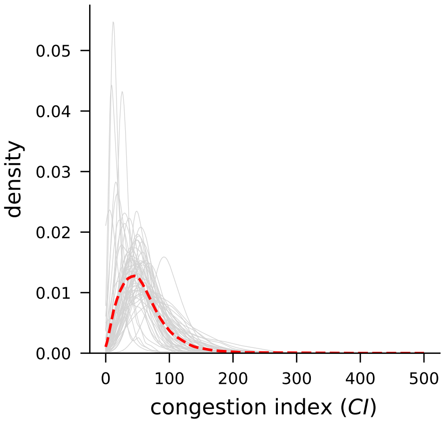


Figure S11: **Distribution of the Congestion Index ($CI$).** The distribution of $CI$ values for all cities (grey lines) and across all trips (red dashed line).

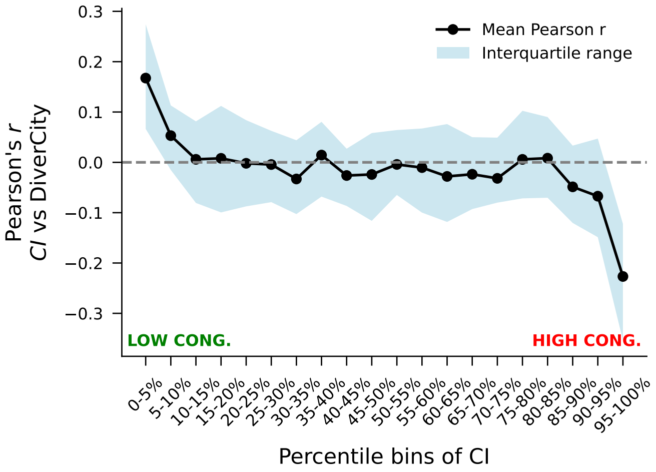


Figure S12: **Correlation between DiverCity and $CI$ across percentile bins of the $CI$ distribution.** Each point represents the average Pearson correlation ($r$) between DiverCity and $CI$ within non-overlapping 5-percentile bins. The shaded area denotes the interquartile range across cities.

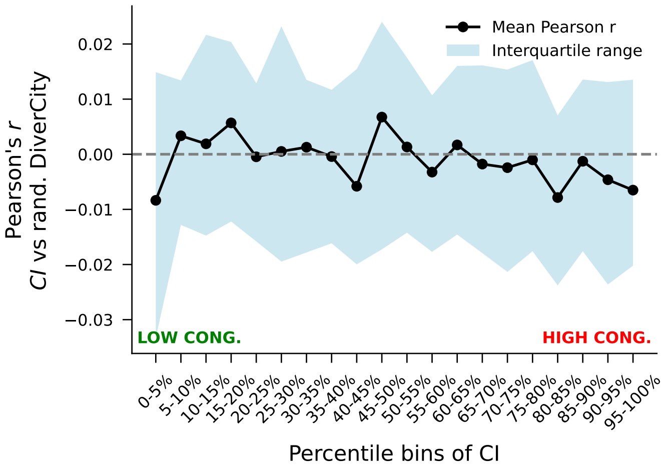


Figure S13: **Correlation between randomly shuffled DiverCity and $CI$ across percentile bins of the $CI$ distribution.** Each point represents the average Pearson correlation ($r$) between DiverCity and $CI$ within non-overlapping 5-percentile bins. The shaded area denotes the interquartile range across cities. As expected, no systematic trend is observed.

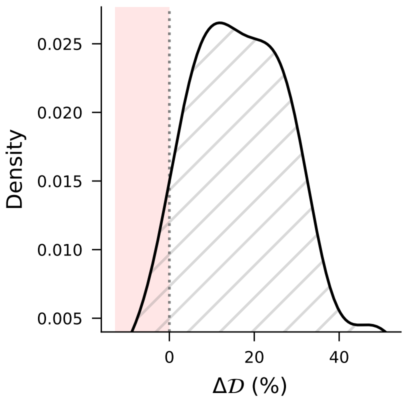


Figure S14: **Distribution of relative DiverCity differences ($\Delta\mathcal{D}$) between non-congested and congested trips across 56 cities.** The distribution of $\Delta\mathcal{D}$, representing the percentage increase in average DiverCity for non-congested trips relative to congested ones, across 56 cities. The red area highlights the region where $\Delta\mathcal{D}$ is negative.

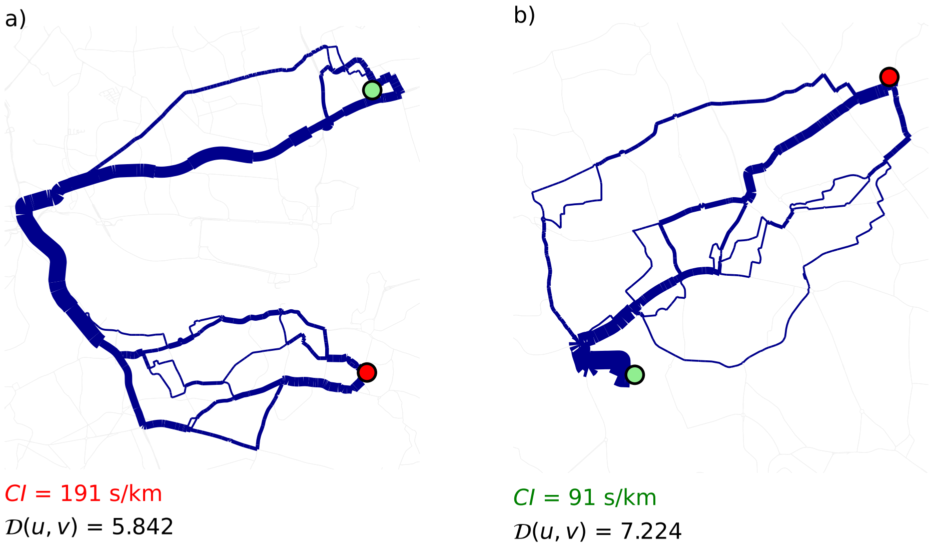


Figure S15: **Examples of trips with equal origin-destination (OD) distance but differing DiverCity and congestion.** Two OD pairs in London, each with a straight-line distance of ≈5 km. (a) A trip with low DiverCity ($D = 5.842$) exhibits high congestion ($CI = 191$ s/km). (b) A trip with higher DiverCity ($D = 7.224$) shows lower congestion ($CI = 91$ s/km).

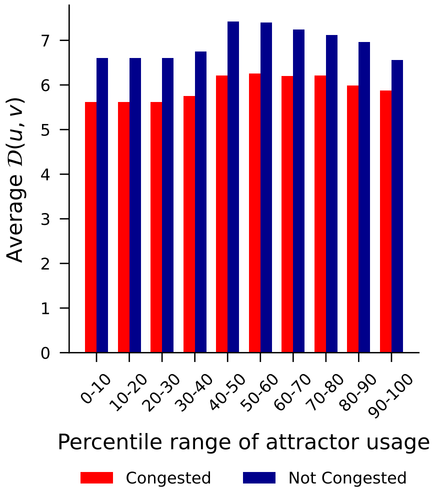


Figure S16: **Average DiverCity for congested and non-congested trips by attractor usage.** Average DiverCity for congested (red) and non-congested (blue) trips, stratified by percentile ranges of attractor usage (i.e., the share of the fastest path overlapping with attractor roads). Within each bin, non-congested trips consistently exhibit higher DiverCity. This trend holds across all levels of attractor reliance.

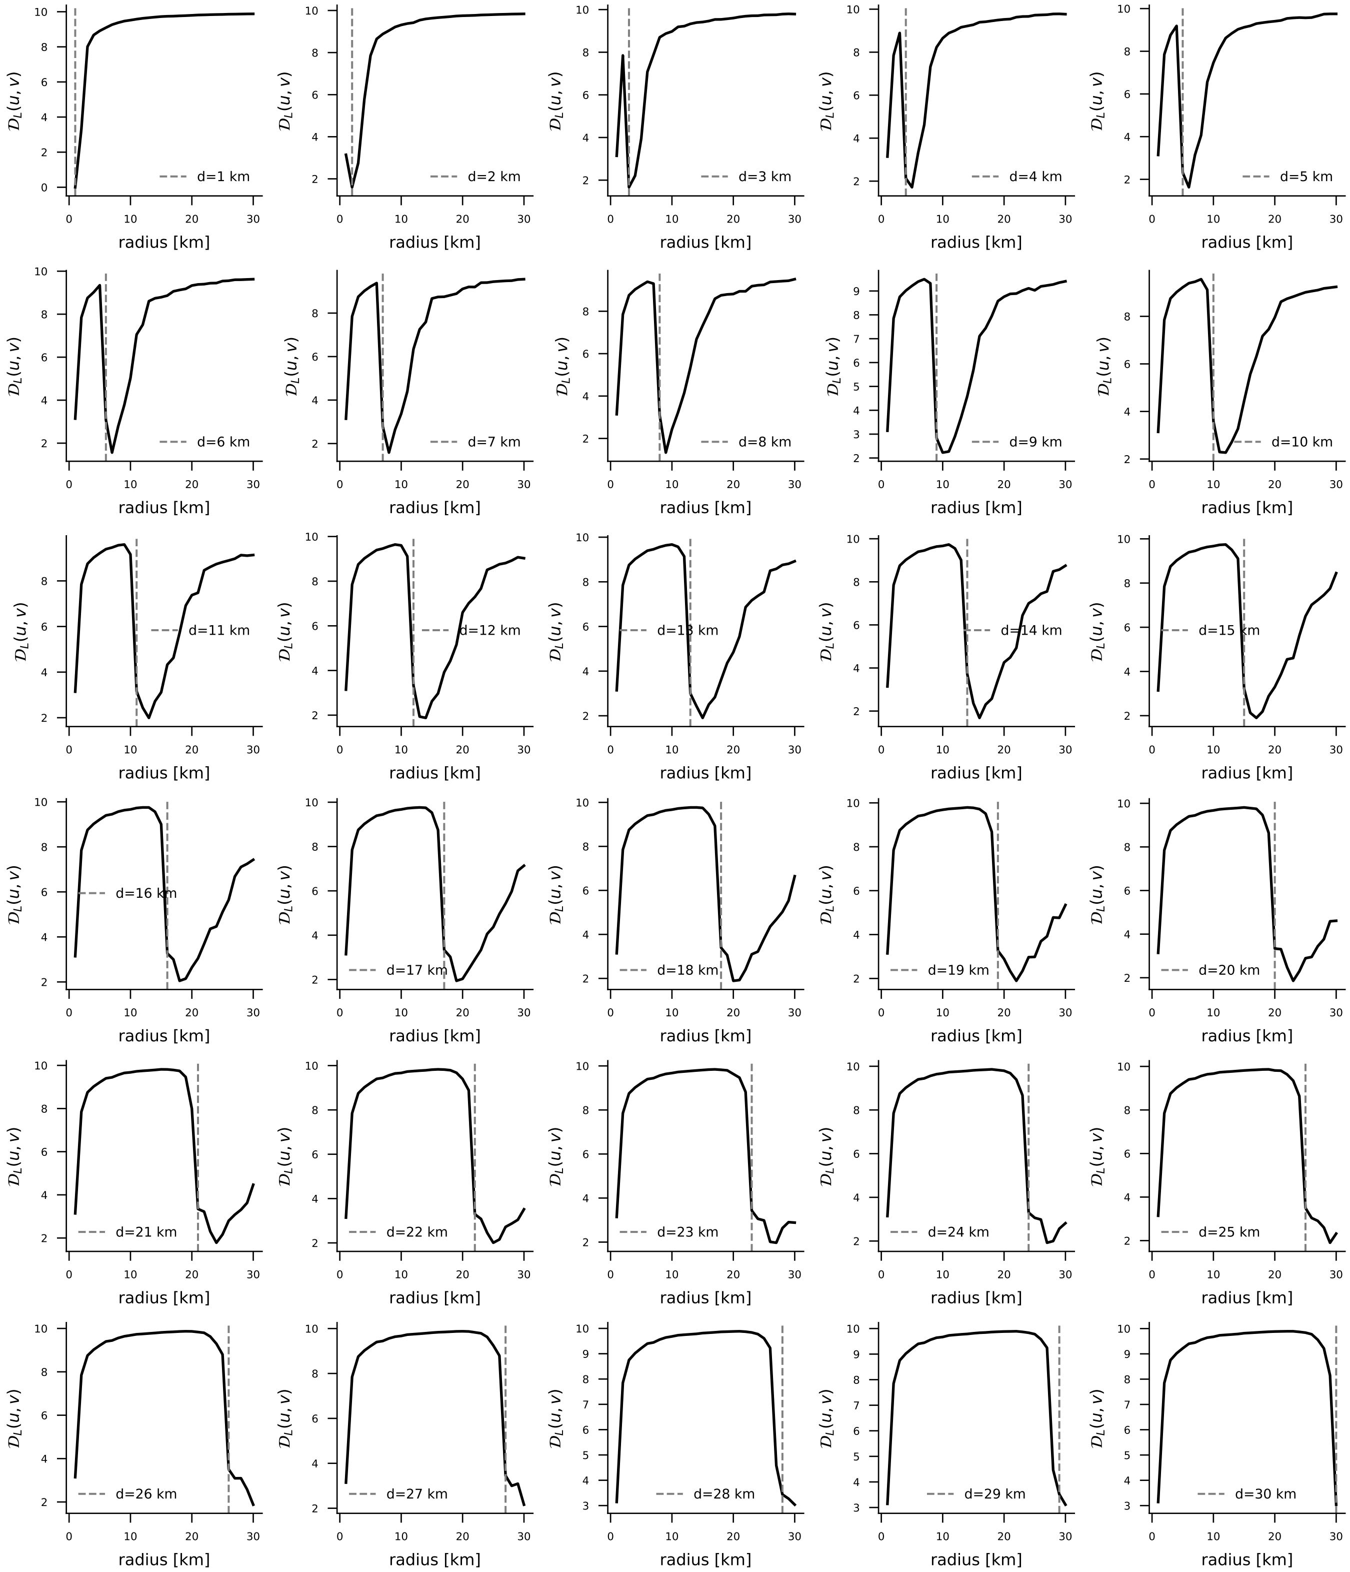


Figure S17: **Spatial distribution of $\mathcal{D}_L(u, v)$ with varying attractor distances ($d$).** DiverCity ($\mathcal{D}_L$) for attractors placed at varying distances $d$ from the grid center. The grey dashed line represents the attractor distance $d$ from the lattice's center. DiverCity consistently decreases near the attractor, demonstrating localized suppression effects.

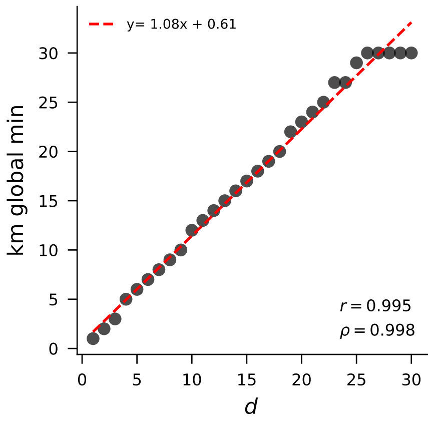


Figure S18: **Relationship between attractor distance ($d$) and the location of minimum DiverCity.** The plot shows a strong linear correlation ($r = 0.995$) between the attractor's distance from the center ($d$) and the location where DiverCity reaches its minimum. The red dashed line represents the best-fit model $y = 1.08x + 0.61$.

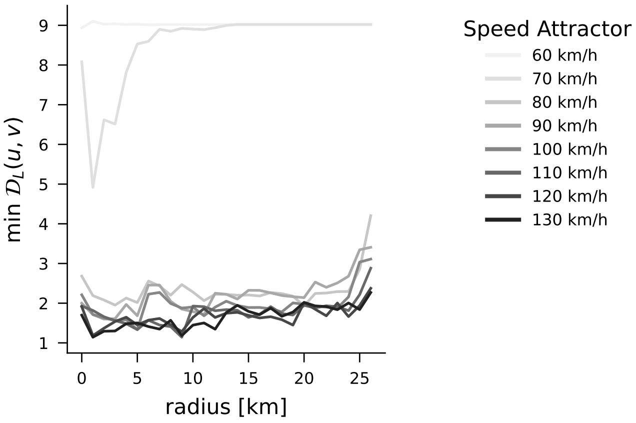


Figure S19: **Effect of attractor speed on the minimum $\mathcal{D}_L(u, v)$.** The minimum value of $\mathcal{D}_L$ (i.e., the extent of the suppression) as a function of attractor speed (60–130 km/h), encoded in different shades of grey. Higher attractor speeds result in lower minimum DiverCity values, confirming that increased speeds amplify suppression effects.

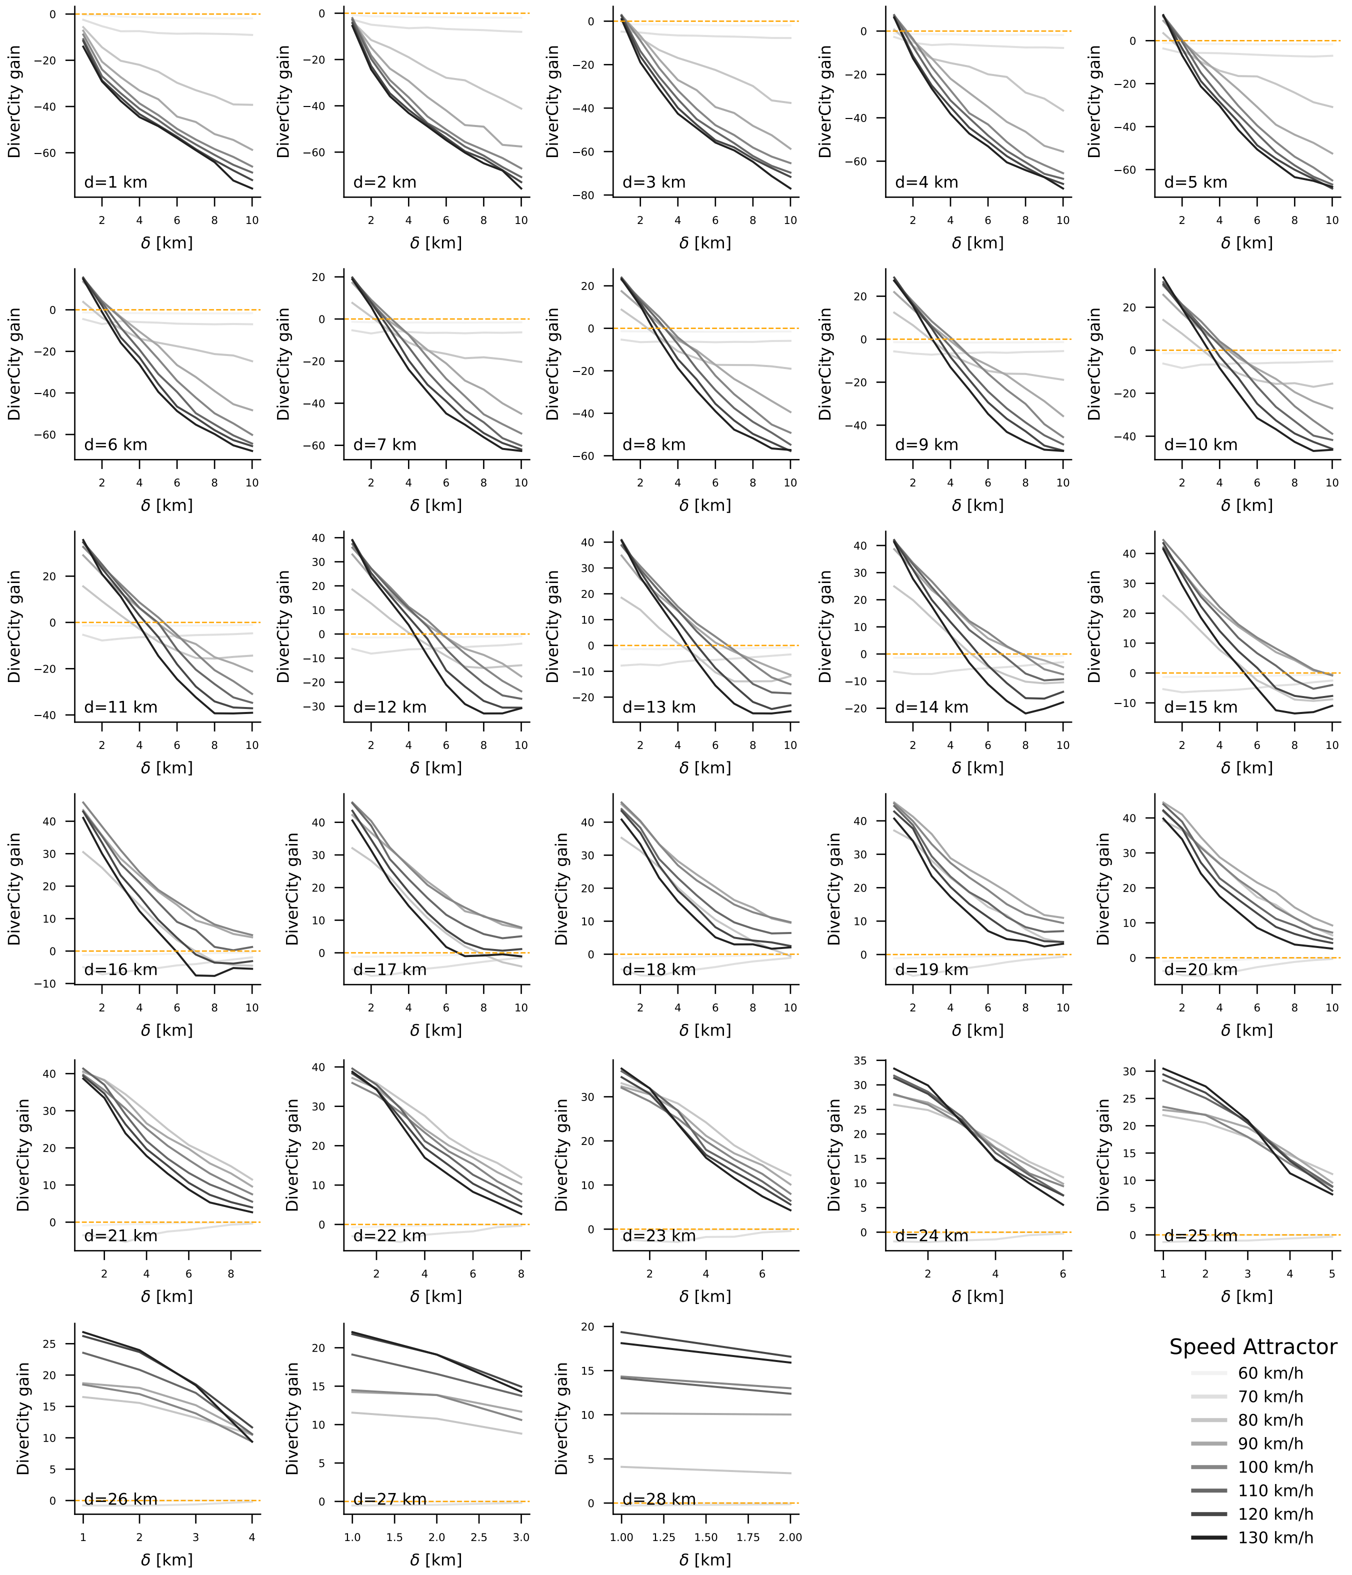


Figure S20: **Effect of offset $\delta$ between two attractors on DiverCity.** The plot shows DiverCity gains for two attractors with varying offsets $\delta$. The benefit of introducing a second attractor, measured by the Area Under the Curve (AUC) difference between $\mathcal{D}_L(u, v)$ with two and one attractors, decreases linearly as $\delta$ increases, with higher-speed attractors maintaining slightly greater benefits. The orange dashed line represents the baseline scenario (i.e., no difference).

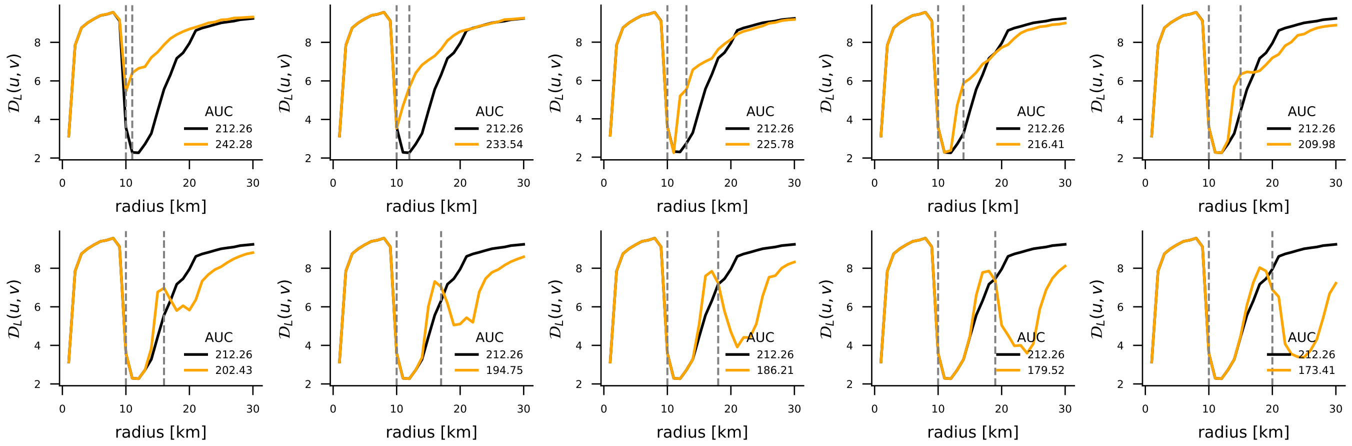


Figure S21: **Impact of a second attractor on DiverCity.** $\mathcal{D}_L$ for an attractor placed at 10 km and a second attractor at varying offsets from the first one. DiverCity increases significantly when the second attractor is close but exhibits two distinct reductions as the offset grows ($\delta$¿5), with the second reduction lagging behind the second attractor's position.

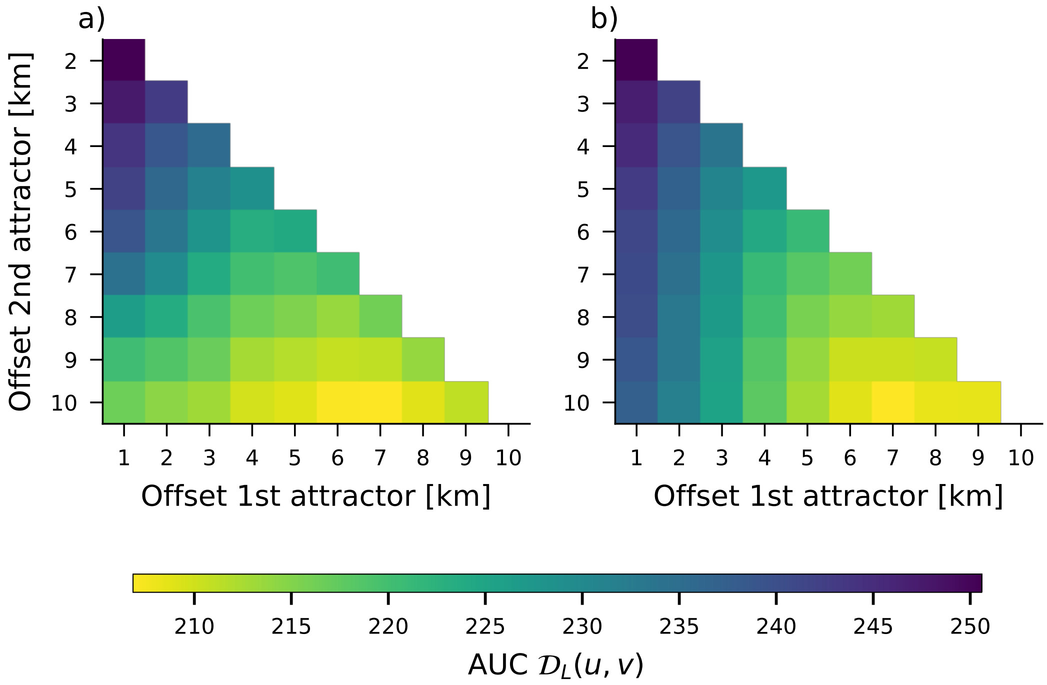


Figure S22: **Heatmatrix of AUC values for configurations with three attractors.** The heatmap shows the Area Under the Curve (AUC) of $\mathcal{D}_L(u,v)$ for different offsets of the second and third attractors relative to the first attractor. The offsets for the first and second attractors are measured in kilometers along the axes. Higher AUC values (lighter colors) correspond to greater route diversification. Closer placement of attractors results in higher AUC values, while increased offsets lead to lower AUC due to fragmented suppression zones.

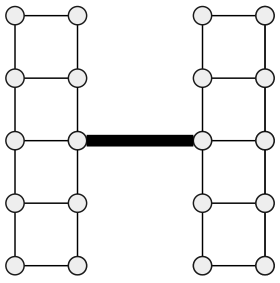

Figure S23: **Bottleneck Implementation in $L$.** Illustrative example of a bottleneck in the lattice $L$. The network is divided into two unconnected regions, linked only by a single mobility attractor (thick black edge), acting as a bridge. This configuration simulates the impact of a critical mobility bottleneck. While depicted here with a small grid for clarity, the actual lattice can be configured with any number of rows and columns.

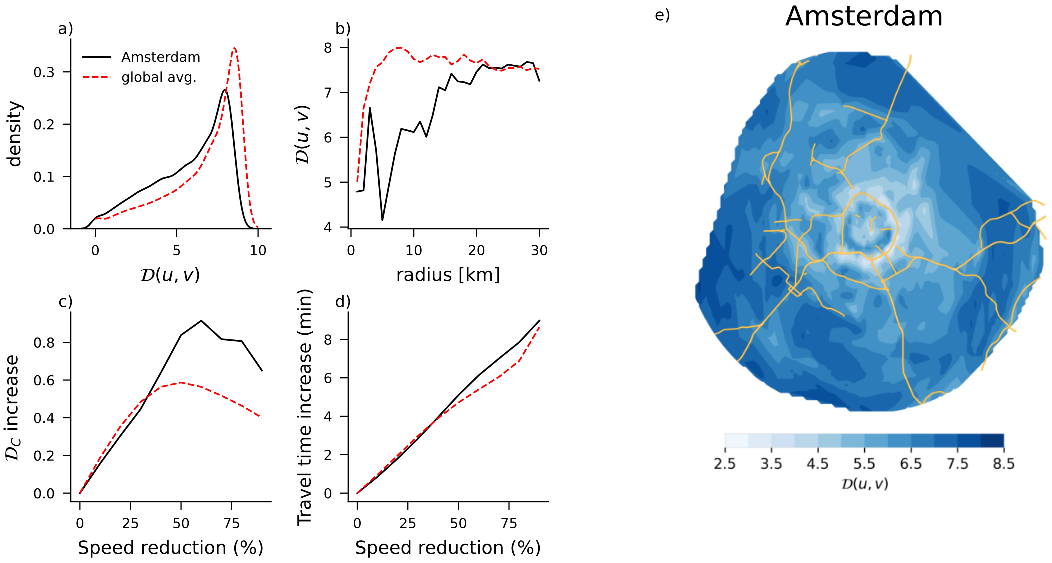


Figure S24: **Summary of DiverCity in Amsterdam.** DiverCity trends in Amsterdam (black solid line) compared to global averages (red dashed line) are shown for: (a) the distribution of $\mathcal{D}(u,v)$, highlighting intra-city variability; (b) $\mathcal{D}(u,v)$ as a function of radial distance from the city center; (c) the increase in DiverCity ($\mathcal{D}_C$) as a function of attractor speed reduction percentages; (d) the increase in travel time as a function of attractor speed reduction percentages; (e) The spatial distribution of $\mathcal{D}(u,v)$ across Amsterdam provides a geographical perspective on route diversification within the city, with mobility attractor roads shown in orange.

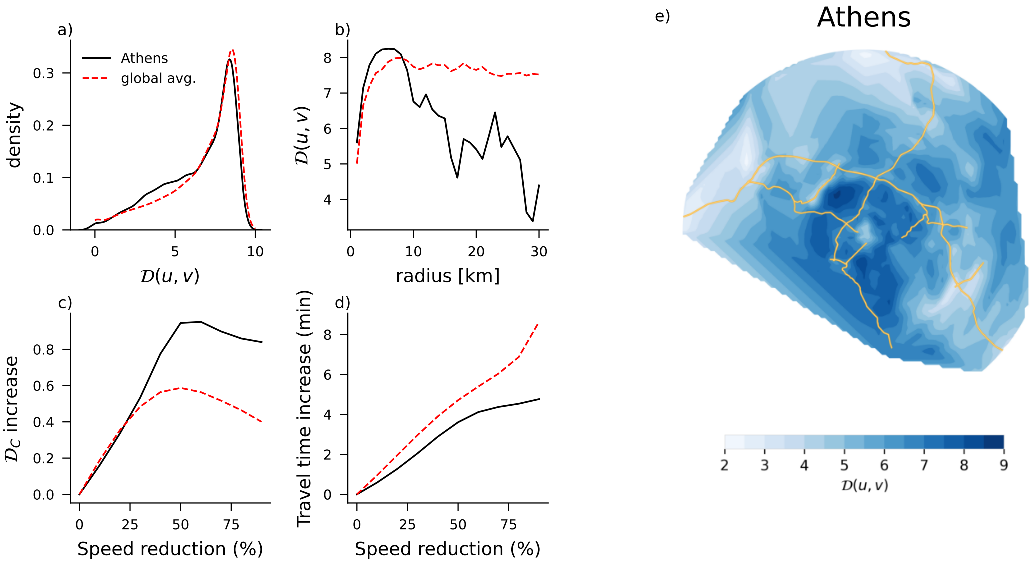


Figure S25: **Summary of DiverCity in Athens.** DiverCity trends in Athens (black solid line) compared to global averages (red dashed line) are shown for: (a) the distribution of $\mathcal{D}(u,v)$, highlighting intra-city variability; (b) $\mathcal{D}(u,v)$ as a function of radial distance from the city center; (c) the increase in DiverCity ($\mathcal{D}_C$) as a function of attractor speed reduction percentages; (d) the increase in travel time as a function of attractor speed reduction percentages; (e) The spatial distribution of $\mathcal{D}(u,v)$ across Athens provides a geographical perspective on route diversification within the city, with mobility attractor roads shown in orange.

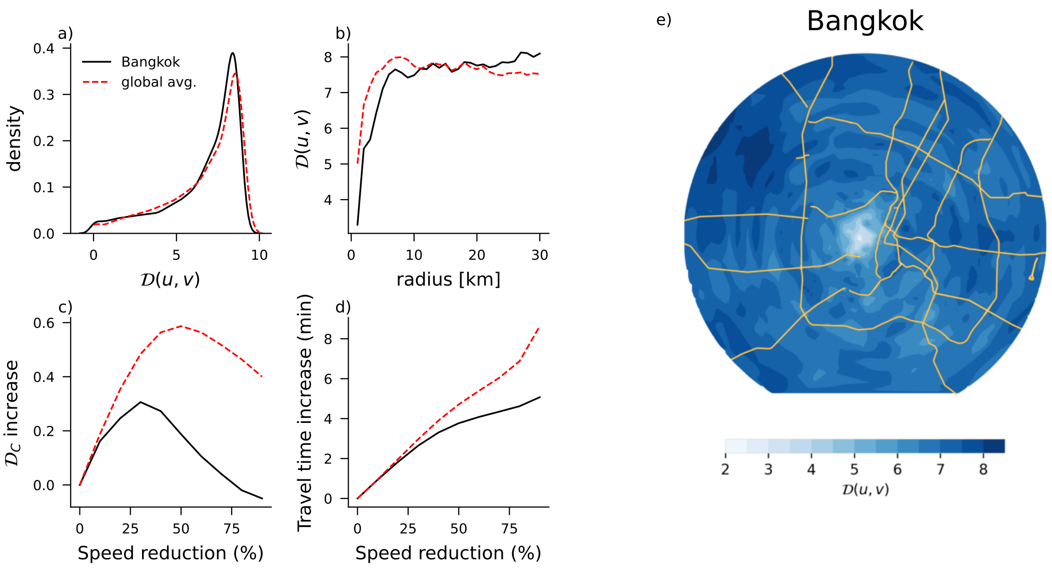


Figure S26: **Summary of DiverCity in Bangkok.** DiverCity trends in Bangkok (black solid line) compared to global averages (red dashed line) are shown for: (a) the distribution of $\mathcal{D}(u, v)$, highlighting intra-city variability; (b) $\mathcal{D}(u, v)$ as a function of radial distance from the city center; (c) the increase in DiverCity ($\mathcal{D}_C$) as a function of attractor speed reduction percentages; (d) the increase in travel time as a function of attractor speed reduction percentages; (e) The spatial distribution of $\mathcal{D}(u, v)$ across Bangkok provides a geographical perspective on route diversification within the city, with mobility attractor roads shown in orange.

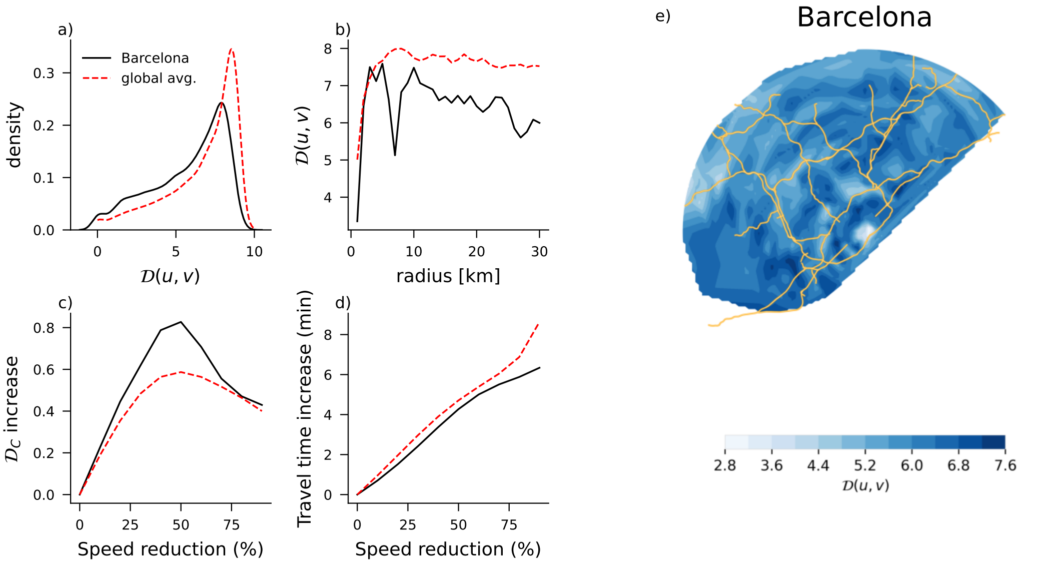


Figure S27: **Summary of DiverCity in Barcelona.** DiverCity trends in Barcelona (black solid line) compared to global averages (red dashed line) are shown for: (a) the distribution of $\mathcal{D}(u, v)$, highlighting intra-city variability; (b) $\mathcal{D}(u, v)$ as a function of radial distance from the city center; (c) the increase in DiverCity ($\mathcal{D}_C$) as a function of attractor speed reduction percentages; (d) the increase in travel time as a function of attractor speed reduction percentages; (e) The spatial distribution of $\mathcal{D}(u, v)$ across Barcelona provides a geographical perspective on route diversification within the city, with mobility attractor roads shown in orange.

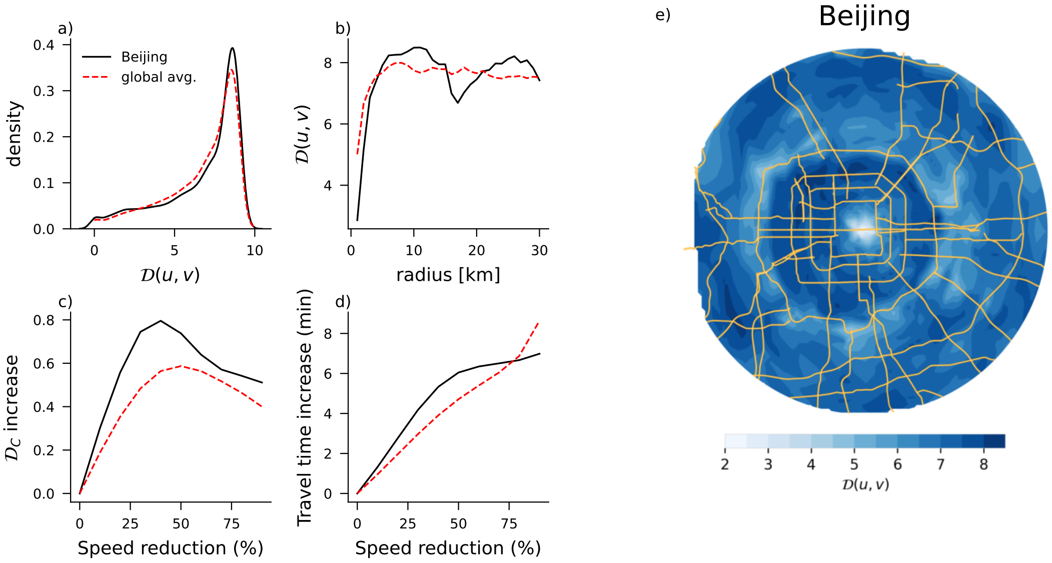


Figure S28: **Summary of DiverCity in Beijing.** DiverCity trends in Beijing (black solid line) compared to global averages (red dashed line) are shown for: (a) the distribution of $\mathcal{D}(u, v)$, highlighting intra-city variability; (b) $\mathcal{D}(u, v)$ as a function of radial distance from the city center; (c) the increase in DiverCity ($\mathcal{D}_C$) as a function of attractor speed reduction percentages; (d) the increase in travel time as a function of attractor speed reduction percentages; (e) The spatial distribution of $\mathcal{D}(u, v)$ across Beijing provides a geographical perspective on route diversification within the city, with mobility attractor roads shown in orange.

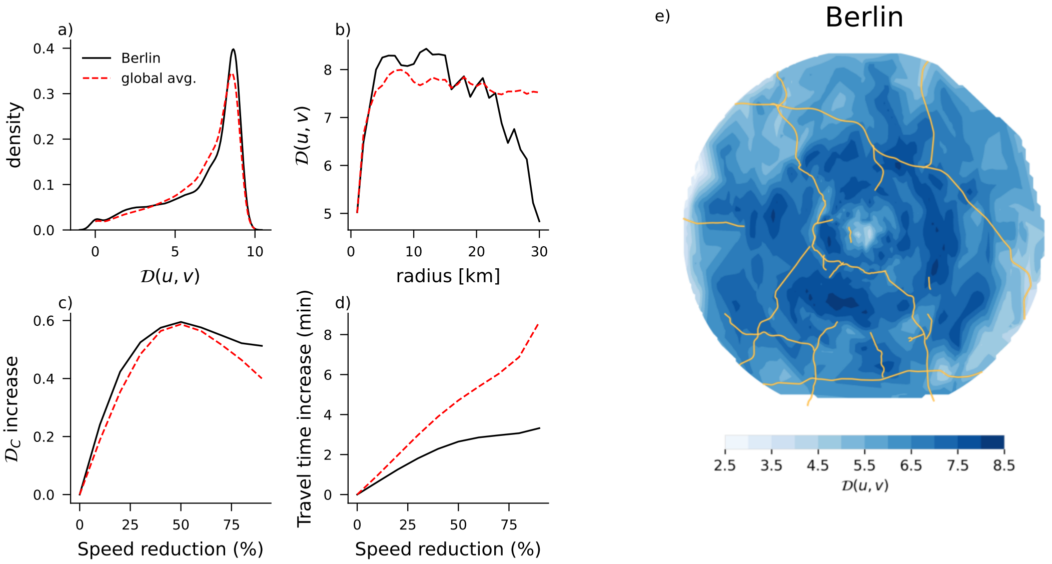


Figure S29: **Summary of DiverCity in Berlin.** DiverCity trends in Berlin (black solid line) compared to global averages (red dashed line) are shown for: (a) the distribution of $\mathcal{D}(u, v)$, highlighting intra-city variability; (b) $\mathcal{D}(u, v)$ as a function of radial distance from the city center; (c) the increase in DiverCity ($\mathcal{D}_C$) as a function of attractor speed reduction percentages; (d) the increase in travel time as a function of attractor speed reduction percentages; (e) The spatial distribution of $\mathcal{D}(u, v)$ across Berlin provides a geographical perspective on route diversification within the city, with mobility attractor roads shown in orange.

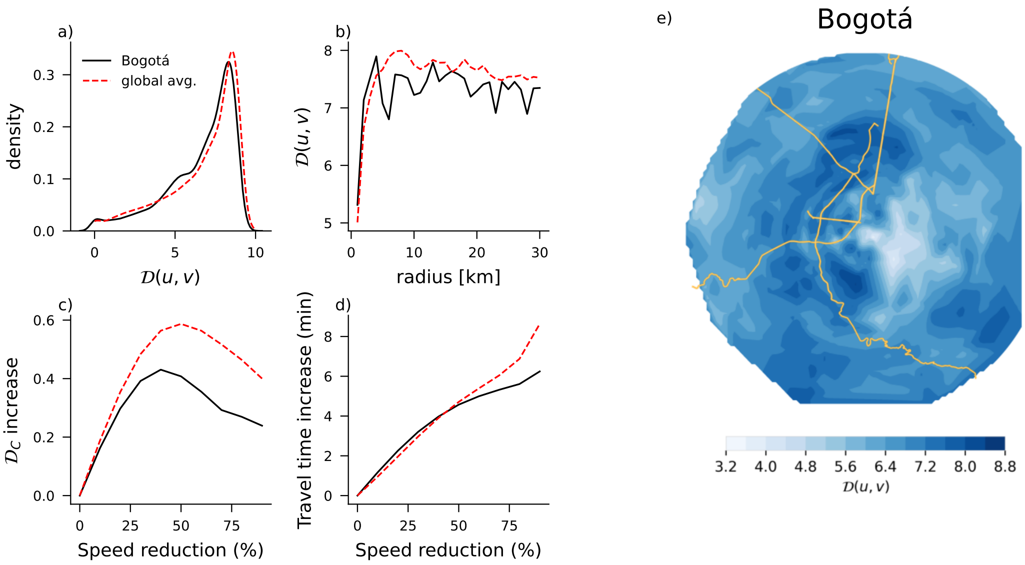


Figure S30: **Summary of DiverCity in Bogotá.** DiverCity trends in Bogotá (black solid line) compared to global averages (red dashed line) are shown for: (a) the distribution of $\mathcal{D}(u, v)$, highlighting intra-city variability; (b) $\mathcal{D}(u, v)$ as a function of radial distance from the city center; (c) the increase in DiverCity ($\mathcal{D}_C$) as a function of attractor speed reduction percentages; (d) the increase in travel time as a function of attractor speed reduction percentages; (e) The spatial distribution of $\mathcal{D}(u, v)$ across Bogotá provides a geographical perspective on route diversification within the city, with mobility attractor roads shown in orange.

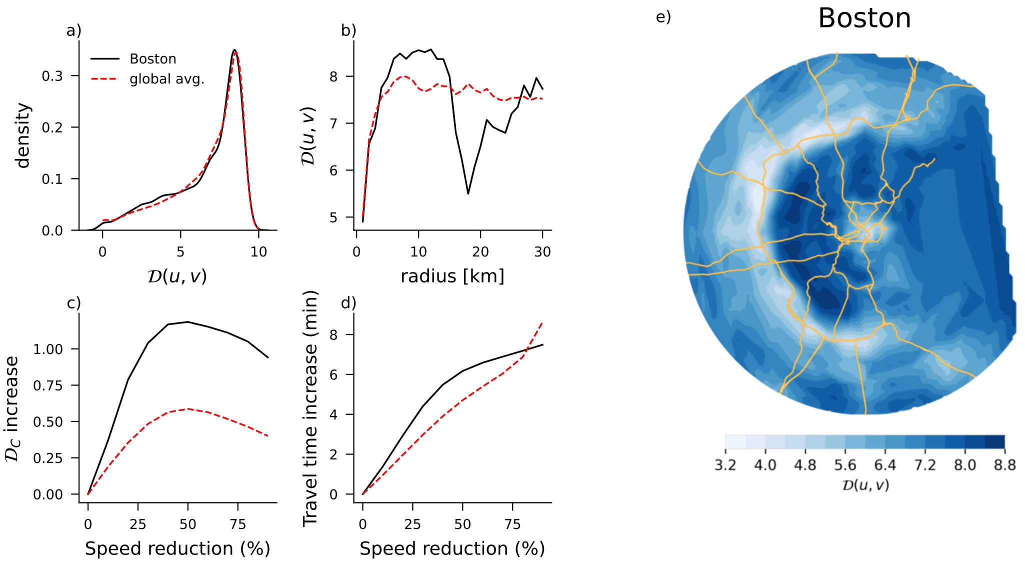


Figure S31: **Summary of DiverCity in Boston.** DiverCity trends in Boston (black solid line) compared to global averages (red dashed line) are shown for: (a) the distribution of $\mathcal{D}(u, v)$, highlighting intra-city variability; (b) $\mathcal{D}(u, v)$ as a function of radial distance from the city center; (c) the increase in DiverCity ($\mathcal{D}_C$) as a function of attractor speed reduction percentages; (d) the increase in travel time as a function of attractor speed reduction percentages; (e) The spatial distribution of $\mathcal{D}(u, v)$ across Boston provides a geographical perspective on route diversification within the city, with mobility attractor roads shown in orange.

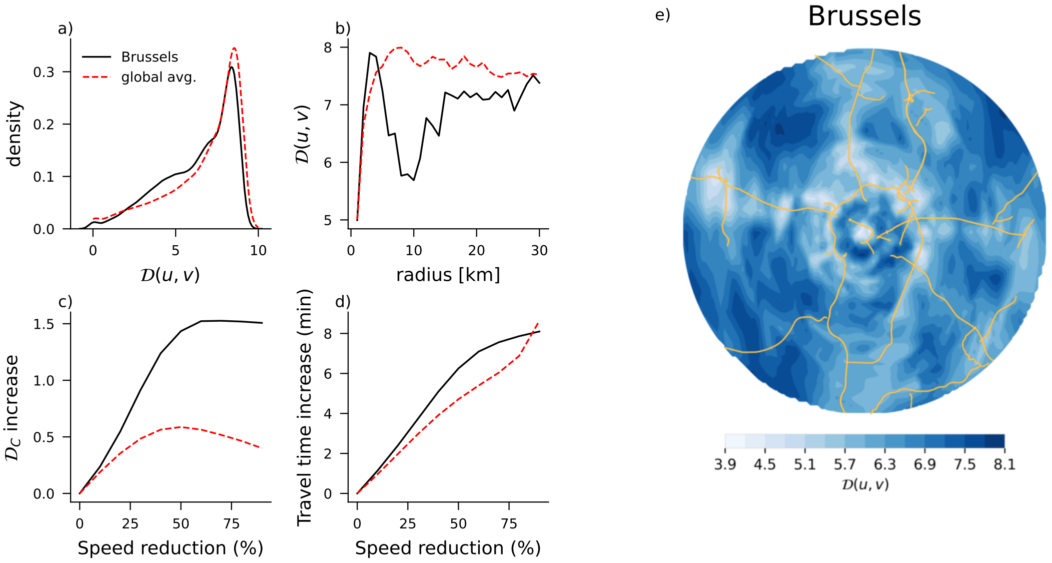


Figure S32: **Summary of DiverCity in Bruxelles.** DiverCity trends in Bruxelles (black solid line) compared to global averages (red dashed line) are shown for: (a) the distribution of $\mathcal{D}(u,v)$, highlighting intra-city variability; (b) $\mathcal{D}(u,v)$ as a function of radial distance from the city center; (c) the increase in DiverCity ($\mathcal{D}_C$) as a function of attractor speed reduction percentages; (d) the increase in travel time as a function of attractor speed reduction percentages; (e) The spatial distribution of $\mathcal{D}(u,v)$ across Bruxelles provides a geographical perspective on route diversification within the city, with mobility attractor roads shown in orange.

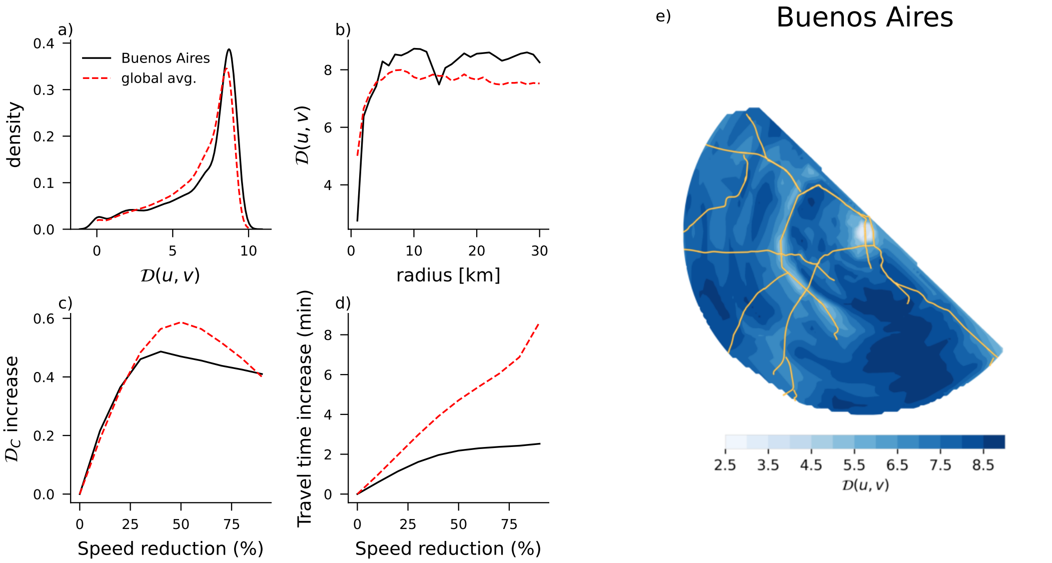


Figure S33: **Summary of DiverCity in Buenos Aires.** DiverCity trends in Buenos Aires (black solid line) compared to global averages (red dashed line) are shown for: (a) the distribution of $\mathcal{D}(u,v)$, highlighting intra-city variability; (b) $\mathcal{D}(u,v)$ as a function of radial distance from the city center; (c) the increase in DiverCity ($\mathcal{D}_C$) as a function of attractor speed reduction percentages; (d) the increase in travel time as a function of attractor speed reduction percentages; (e) The spatial distribution of $\mathcal{D}(u,v)$ across Buenos Aires provides a geographical perspective on route diversification within the city, with mobility attractor roads shown in orange.

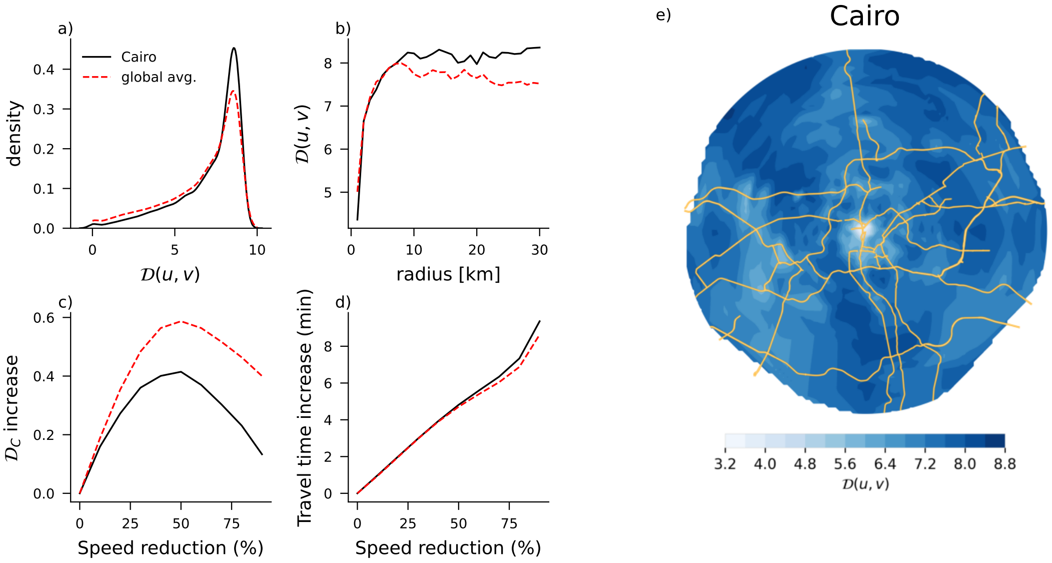


Figure S34: **Summary of DiverCity in Cairo.** DiverCity trends in Cairo (black solid line) compared to global averages (red dashed line) are shown for: (a) the distribution of $\mathcal{D}(u, v)$, highlighting intra-city variability; (b) $\mathcal{D}(u, v)$ as a function of radial distance from the city center; (c) the increase in DiverCity ($\mathcal{D}_C$) as a function of attractor speed reduction percentages; (d) the increase in travel time as a function of attractor speed reduction percentages; (e) The spatial distribution of $\mathcal{D}(u, v)$ across Cairo provides a geographical perspective on route diversification within the city, with mobility attractor roads shown in orange.

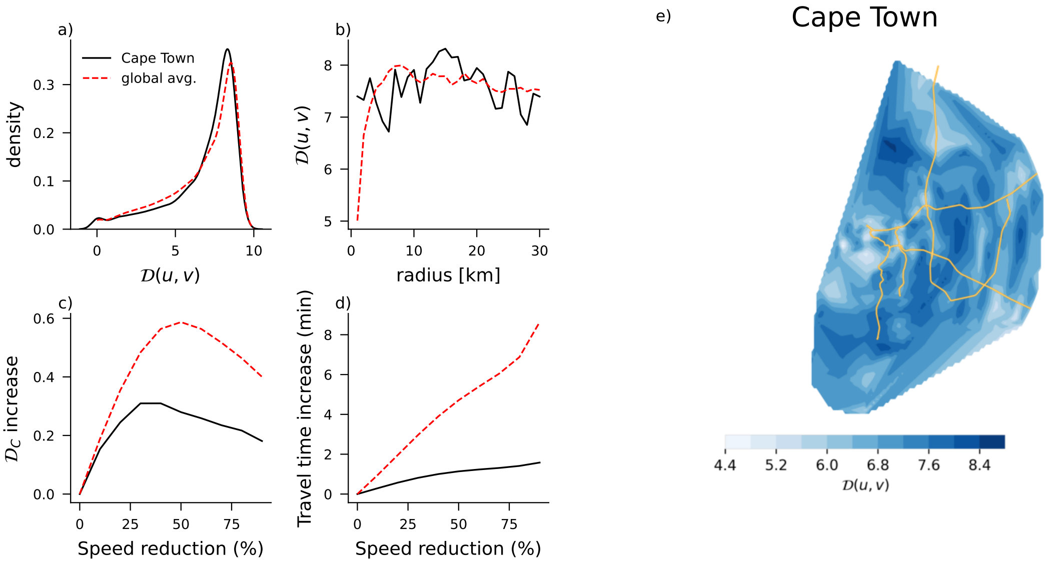


Figure S35: **Summary of DiverCity in Cape Town.** DiverCity trends in Cape Town (black solid line) compared to global averages (red dashed line) are shown for: (a) the distribution of $\mathcal{D}(u, v)$, highlighting intra-city variability; (b) $\mathcal{D}(u, v)$ as a function of radial distance from the city center; (c) the increase in DiverCity ($\mathcal{D}_C$) as a function of attractor speed reduction percentages; (d) the increase in travel time as a function of attractor speed reduction percentages; (e) The spatial distribution of $\mathcal{D}(u, v)$ across Cape Town provides a geographical perspective on route diversification within the city, with mobility attractor roads shown in orange.

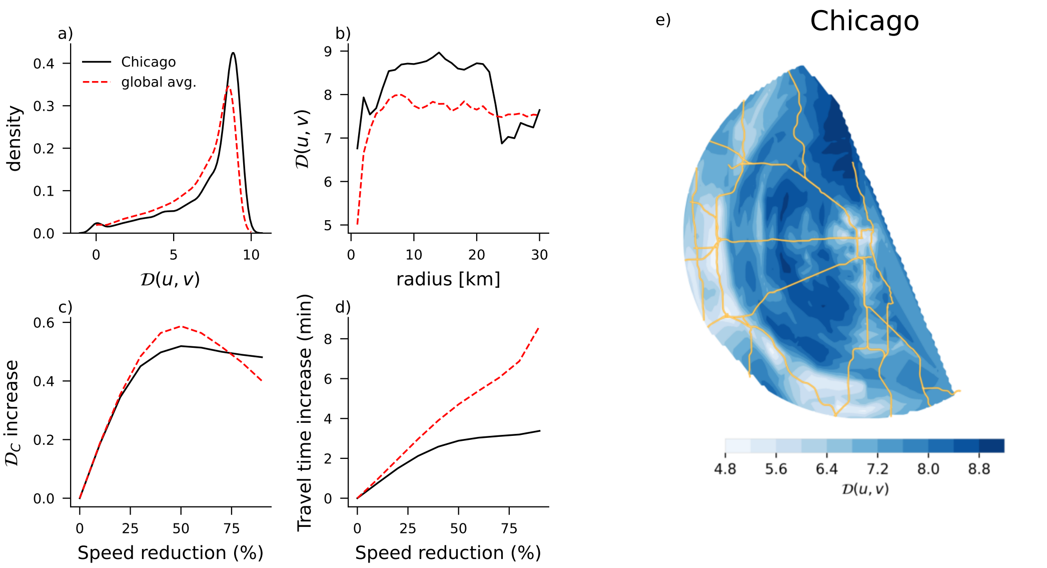


Figure S36: **Summary of DiverCity in Chicago.** DiverCity trends in Chicago (black solid line) compared to global averages (red dashed line) are shown for: (a) the distribution of $\mathcal{D}(u,v)$, highlighting intra-city variability; (b) $\mathcal{D}(u,v)$ as a function of radial distance from the city center; (c) the increase in DiverCity ($\mathcal{D}_C$) as a function of attractor speed reduction percentages; (d) the increase in travel time as a function of attractor speed reduction percentages; (e) The spatial distribution of $\mathcal{D}(u,v)$ across Chicago provides a geographical perspective on route diversification within the city, with mobility attractor roads shown in orange.

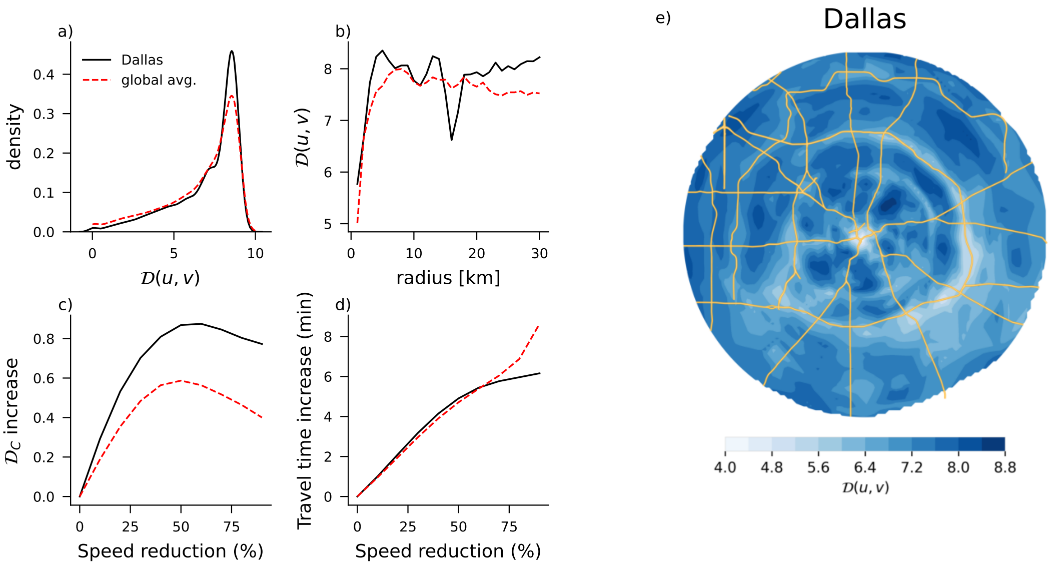


Figure S37: **Summary of DiverCity in Dallas.** DiverCity trends in Dallas (black solid line) compared to global averages (red dashed line) are shown for: (a) the distribution of $\mathcal{D}(u,v)$, highlighting intra-city variability; (b) $\mathcal{D}(u,v)$ as a function of radial distance from the city center; (c) the increase in DiverCity ($\mathcal{D}_C$) as a function of attractor speed reduction percentages; (d) the increase in travel time as a function of attractor speed reduction percentages; (e) The spatial distribution of $\mathcal{D}(u,v)$ across Dallas provides a geographical perspective on route diversification within the city, with mobility attractor roads shown in orange.

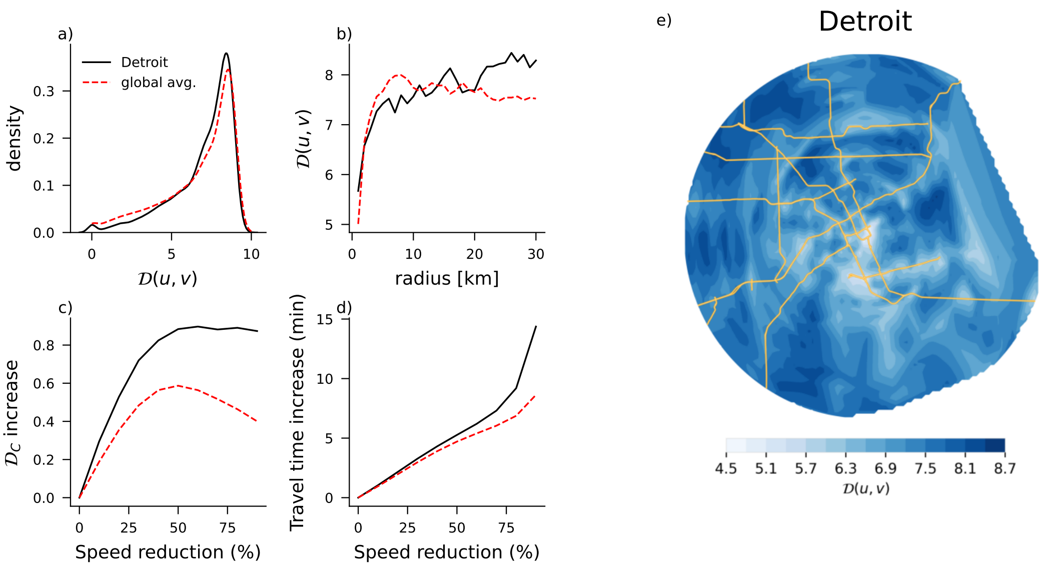


Figure S38: **Summary of DiverCity in Detroit.** DiverCity trends in Detroit (black solid line) compared to global averages (red dashed line) are shown for: (a) the distribution of $\mathcal{D}(u, v)$, highlighting intra-city variability; (b) $\mathcal{D}(u, v)$ as a function of radial distance from the city center; (c) the increase in DiverCity ($\mathcal{D}_C$) as a function of attractor speed reduction percentages; (d) the increase in travel time as a function of attractor speed reduction percentages; (e) The spatial distribution of $\mathcal{D}(u, v)$ across Detroit provides a geographical perspective on route diversification within the city, with mobility attractor roads shown in orange.

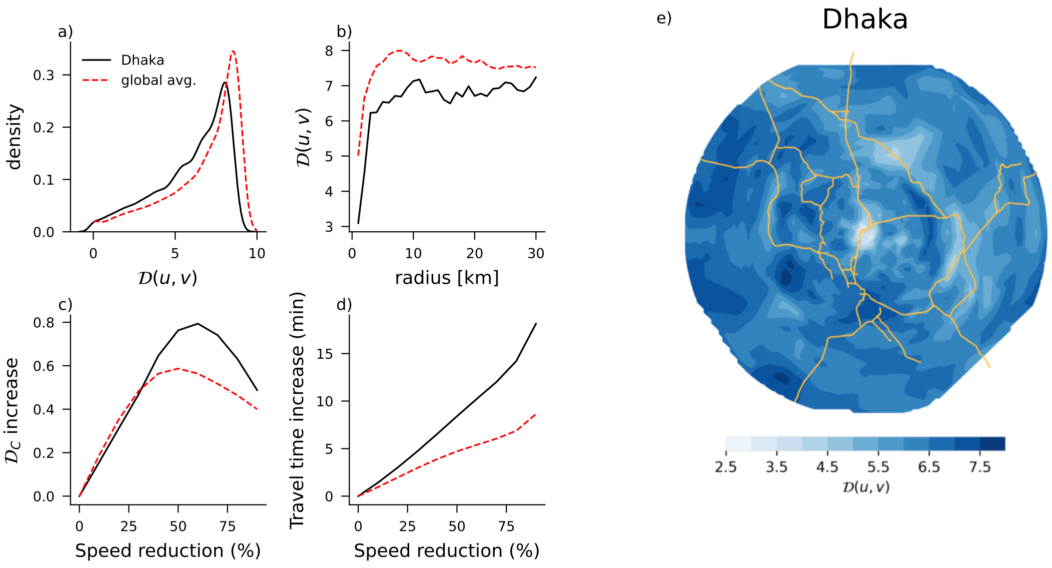


Figure S39: **Summary of DiverCity in Dhaka.** DiverCity trends in Dhaka (black solid line) compared to global averages (red dashed line) are shown for: (a) the distribution of $\mathcal{D}(u, v)$, highlighting intra-city variability; (b) $\mathcal{D}(u, v)$ as a function of radial distance from the city center; (c) the increase in DiverCity ($\mathcal{D}_C$) as a function of attractor speed reduction percentages; (d) the increase in travel time as a function of attractor speed reduction percentages; (e) The spatial distribution of $\mathcal{D}(u, v)$ across Detroit provides a geographical perspective on route diversification within the city, with mobility attractor roads shown in orange.

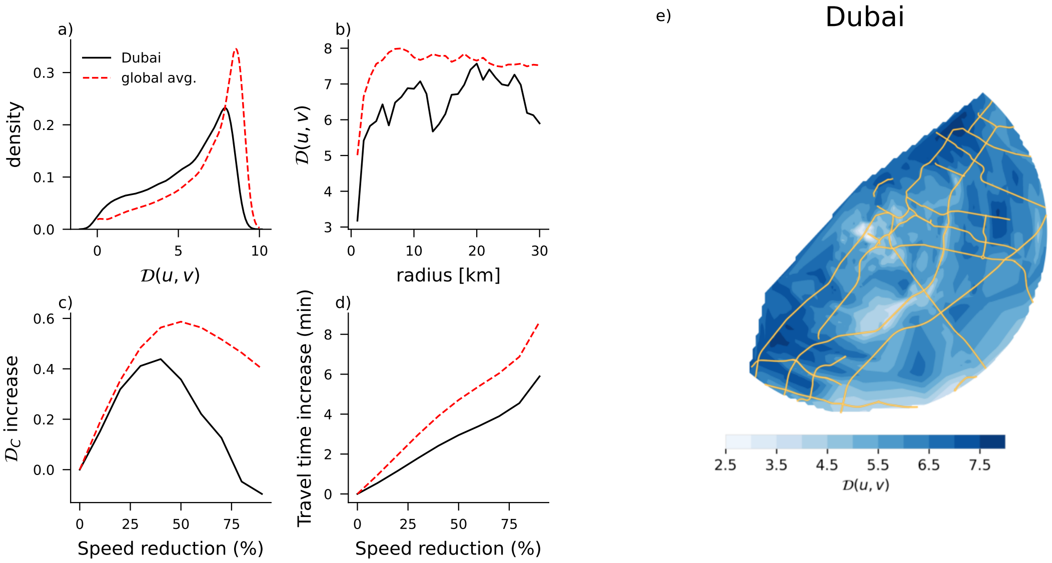


Figure S40: **Summary of DiverCity in Dubai.** DiverCity trends in Dubai (black solid line) compared to global averages (red dashed line) are shown for: (a) the distribution of $\mathcal{D}(u, v)$, highlighting intra-city variability; (b) $\mathcal{D}(u, v)$ as a function of radial distance from the city center; (c) the increase in DiverCity ($\mathcal{D}_C$) as a function of attractor speed reduction percentages; (d) the increase in travel time as a function of attractor speed reduction percentages; (e) The spatial distribution of $\mathcal{D}(u, v)$ across Dubai provides a geographical perspective on route diversification within the city, with mobility attractor roads shown in orange.

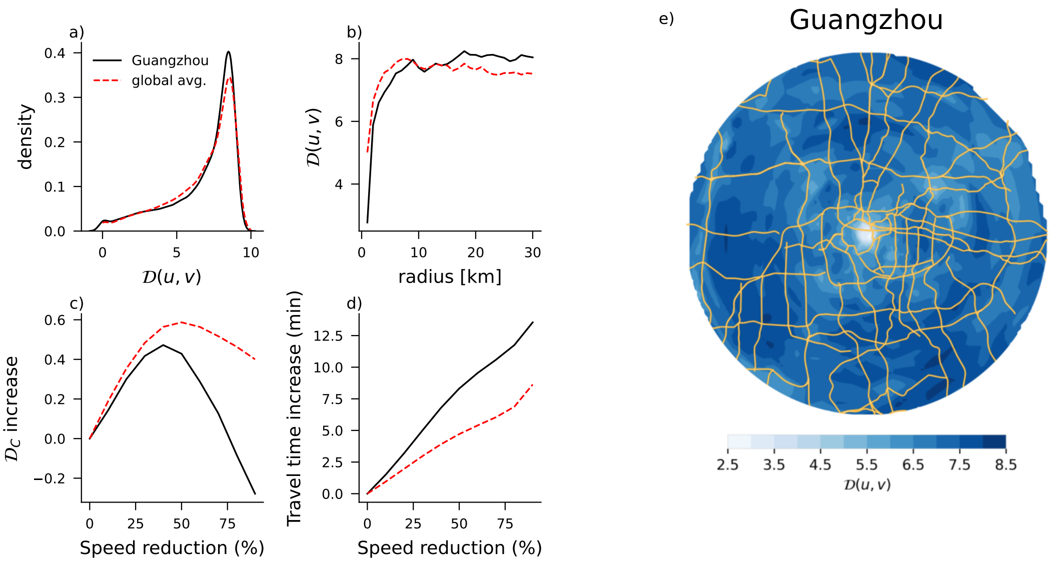


Figure S41: **Summary of DiverCity in Guangzhou.** DiverCity trends in Guangzhou (black solid line) compared to global averages (red dashed line) are shown for: (a) the distribution of $\mathcal{D}(u, v)$, highlighting intra-city variability; (b) $\mathcal{D}(u, v)$ as a function of radial distance from the city center; (c) the increase in DiverCity ($\mathcal{D}_C$) as a function of attractor speed reduction percentages; (d) the increase in travel time as a function of attractor speed reduction percentages; (e) The spatial distribution of $\mathcal{D}(u, v)$ across Guangzhou provides a geographical perspective on route diversification within the city, with mobility attractor roads shown in orange.

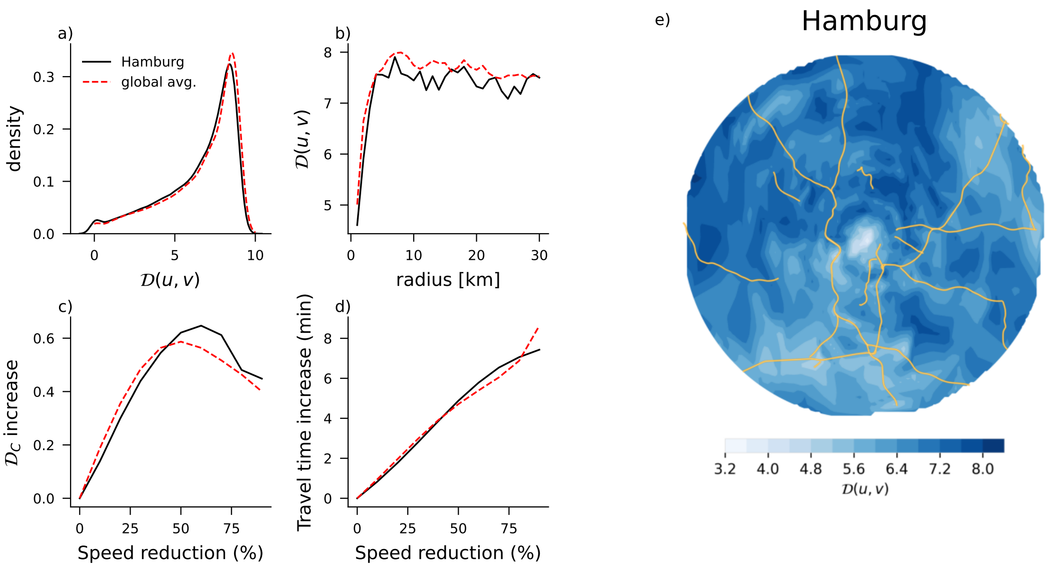


Figure S42: **Summary of DiverCity in Hamburg.** DiverCity trends in Hamburg (black solid line) compared to global averages (red dashed line) are shown for: (a) the distribution of $\mathcal{D}(u, v)$, highlighting intra-city variability; (b) $\mathcal{D}(u, v)$ as a function of radial distance from the city center; (c) the increase in DiverCity ($\mathcal{D}_C$) as a function of attractor speed reduction percentages; (d) the increase in travel time as a function of attractor speed reduction percentages; (e) The spatial distribution of $\mathcal{D}(u, v)$ across Hamburg provides a geographical perspective on route diversification within the city, with mobility attractor roads shown in orange.

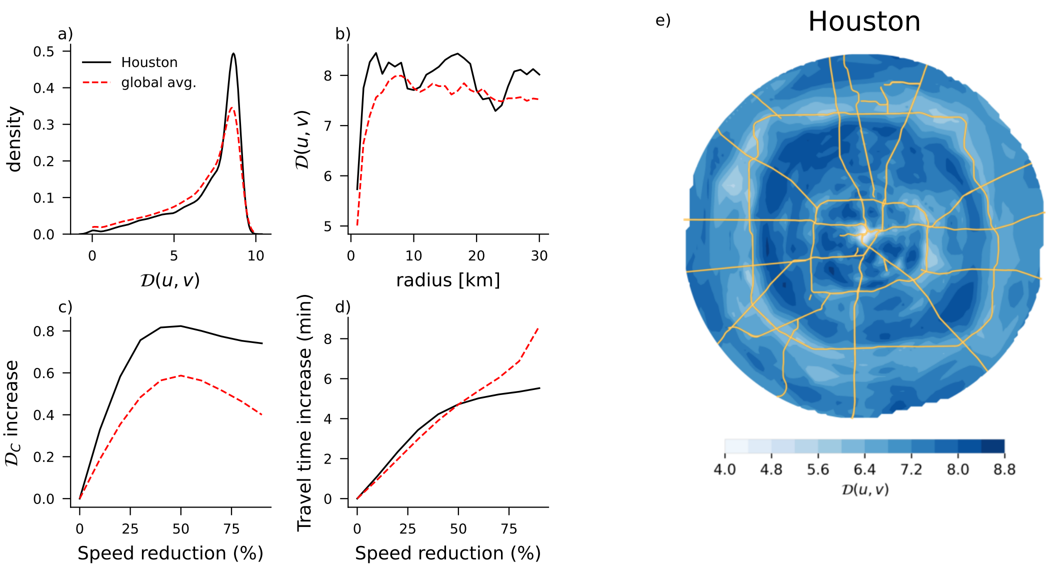


Figure S43: **Summary of DiverCity in Houston.** DiverCity trends in Houston (black solid line) compared to global averages (red dashed line) are shown for: (a) the distribution of $\mathcal{D}(u, v)$, highlighting intra-city variability; (b) $\mathcal{D}(u, v)$ as a function of radial distance from the city center; (c) the increase in DiverCity ($\mathcal{D}_C$) as a function of attractor speed reduction percentages; (d) the increase in travel time as a function of attractor speed reduction percentages; (e) The spatial distribution of $\mathcal{D}(u, v)$ across Houston provides a geographical perspective on route diversification within the city, with mobility attractor roads shown in orange.

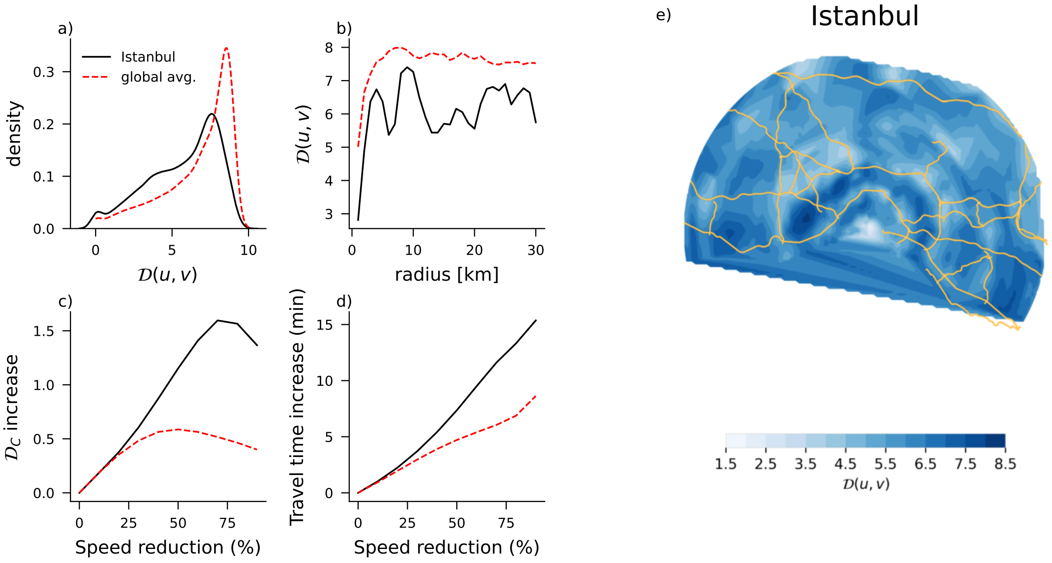


Figure S44: **Summary of DiverCity in Istanbul.** DiverCity trends in Istanbul (black solid line) compared to global averages (red dashed line) are shown for: (a) the distribution of $\mathcal{D}(u, v)$, highlighting intra-city variability; (b) $\mathcal{D}(u, v)$ as a function of radial distance from the city center; (c) the increase in DiverCity ($\mathcal{D}_C$) as a function of attractor speed reduction percentages; (d) the increase in travel time as a function of attractor speed reduction percentages; (e) The spatial distribution of $\mathcal{D}(u, v)$ across Istanbul provides a geographical perspective on route diversification within the city, with mobility attractor roads shown in orange.

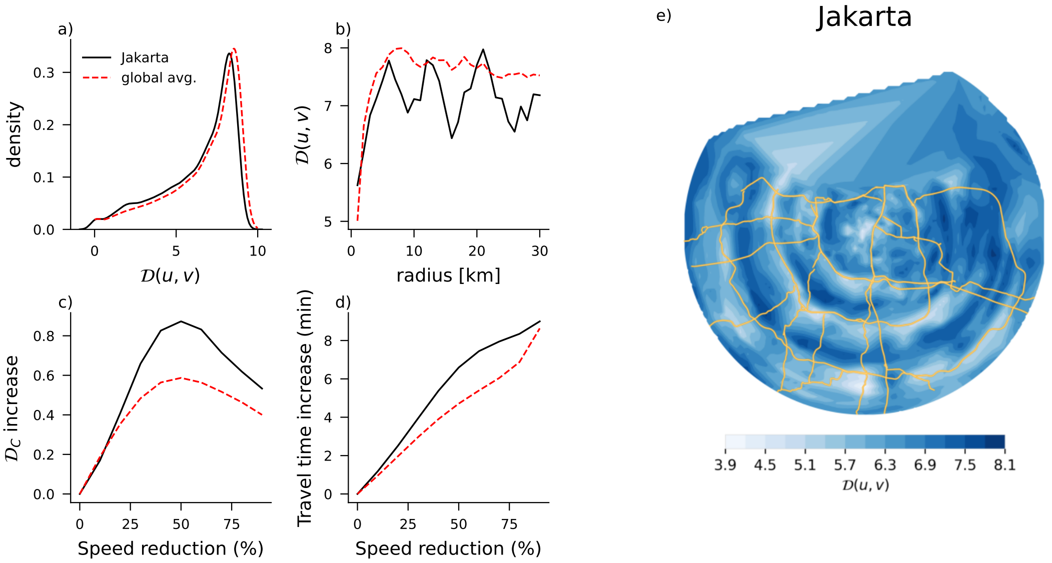


Figure S45: **Summary of DiverCity in Jakarta.** DiverCity trends in Jakarta (black solid line) compared to global averages (red dashed line) are shown for: (a) the distribution of $\mathcal{D}(u, v)$, highlighting intra-city variability; (b) $\mathcal{D}(u, v)$ as a function of radial distance from the city center; (c) the increase in DiverCity ($\mathcal{D}_C$) as a function of attractor speed reduction percentages; (d) the increase in travel time as a function of attractor speed reduction percentages; (e) The spatial distribution of $\mathcal{D}(u, v)$ across Jakarta provides a geographical perspective on route diversification within the city, with mobility attractor roads shown in orange.

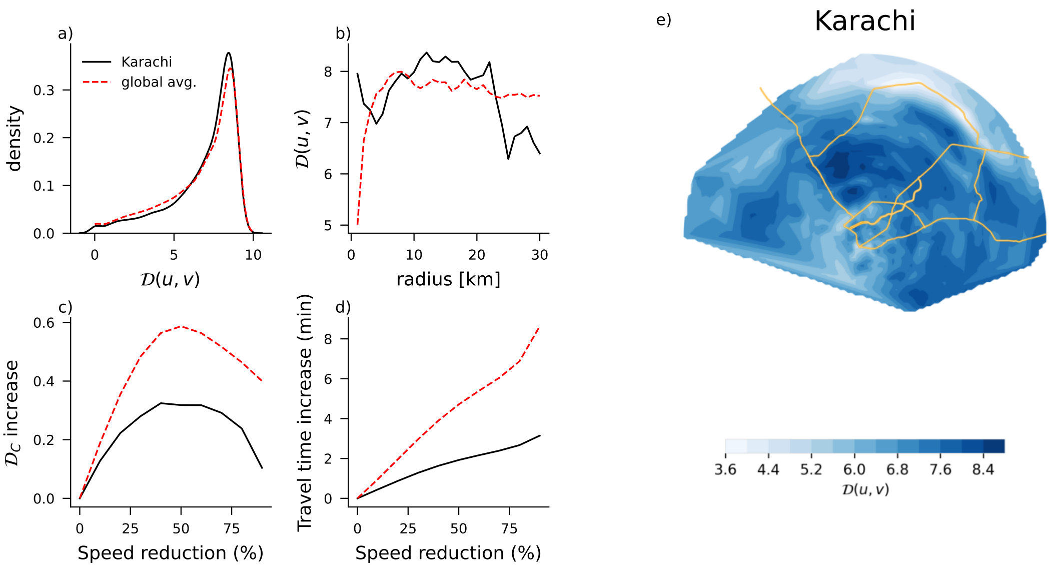


Figure S46: **Summary of DiverCity in Karachi.** DiverCity trends in Karachi (black solid line) compared to global averages (red dashed line) are shown for: (a) the distribution of $\mathcal{D}(u, v)$, highlighting intra-city variability; (b) $\mathcal{D}(u, v)$ as a function of radial distance from the city center; (c) the increase in DiverCity ($\mathcal{D}_C$) as a function of attractor speed reduction percentages; (d) the increase in travel time as a function of attractor speed reduction percentages; (e) The spatial distribution of $\mathcal{D}(u, v)$ across Karachi provides a geographical perspective on route diversification within the city, with mobility attractor roads shown in orange.

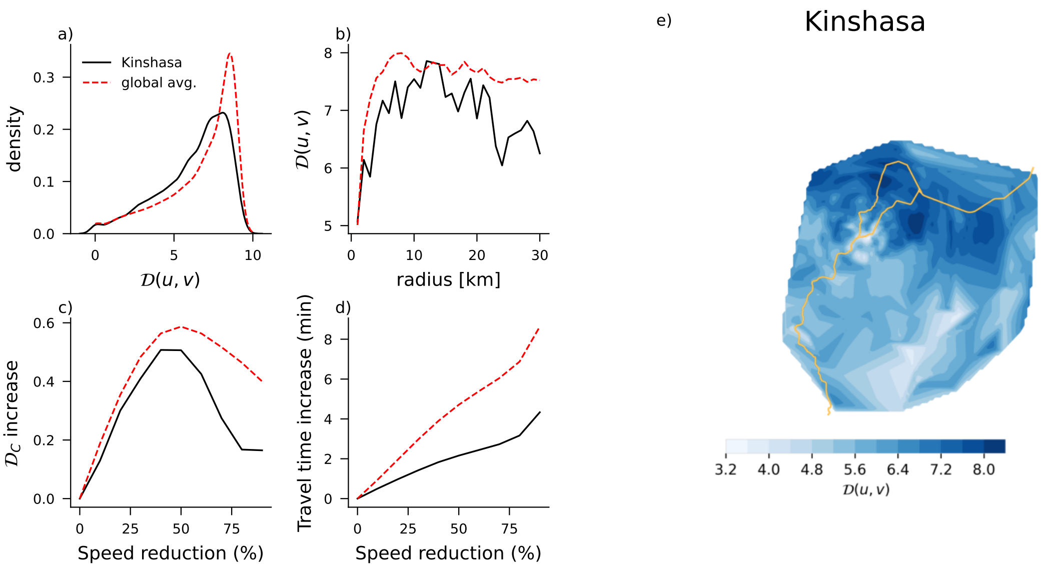


Figure S47: **Summary of DiverCity in Kinshasa.** DiverCity trends in Kinshasa (black solid line) compared to global averages (red dashed line) are shown for: (a) the distribution of $\mathcal{D}(u, v)$, highlighting intra-city variability; (b) $\mathcal{D}(u, v)$ as a function of radial distance from the city center; (c) the increase in DiverCity ($\mathcal{D}_C$) as a function of attractor speed reduction percentages; (d) the increase in travel time as a function of attractor speed reduction percentages; (e) The spatial distribution of $\mathcal{D}(u, v)$ across Kinshasa provides a geographical perspective on route diversification within the city, with mobility attractor roads shown in orange.

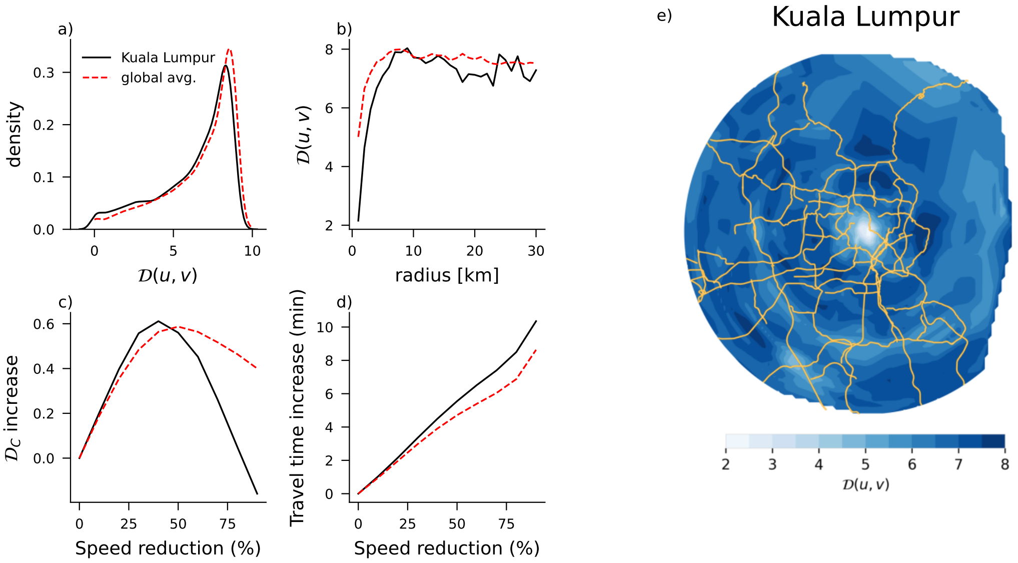


Figure S48: **Summary of DiverCity in Kuala Lumpur.** DiverCity trends in Kuala Lumpur (black solid line) compared to global averages (red dashed line) are shown for: (a) the distribution of $\mathcal{D}(u, v)$, highlighting intra-city variability; (b) $\mathcal{D}(u, v)$ as a function of radial distance from the city center; (c) the increase in DiverCity ($\mathcal{D}_C$) as a function of attractor speed reduction percentages; (d) the increase in travel time as a function of attractor speed reduction percentages; (e) The spatial distribution of $\mathcal{D}(u, v)$ across Kuala Lumpur provides a geographical perspective on route diversification within the city, with mobility attractor roads shown in orange.

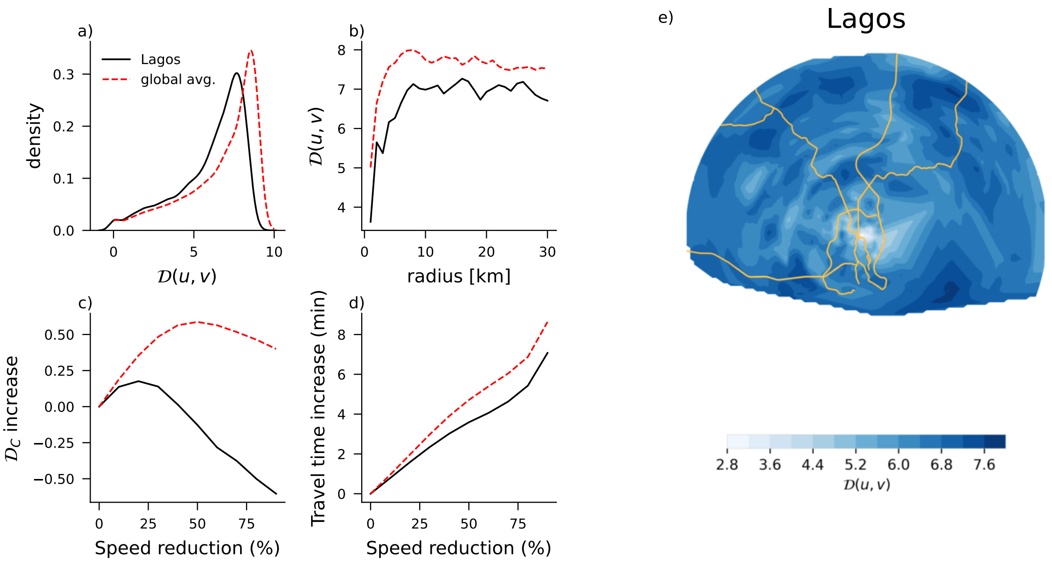


Figure S49: **Summary of DiverCity in Lagos.** DiverCity trends in Lagos (black solid line) compared to global averages (red dashed line) are shown for: (a) the distribution of $\mathcal{D}(u, v)$, highlighting intra-city variability; (b) $\mathcal{D}(u, v)$ as a function of radial distance from the city center; (c) the increase in DiverCity ($\mathcal{D}_C$) as a function of attractor speed reduction percentages; (d) the increase in travel time as a function of attractor speed reduction percentages; (e) The spatial distribution of $\mathcal{D}(u, v)$ across Lagos provides a geographical perspective on route diversification within the city, with mobility attractor roads shown in orange.

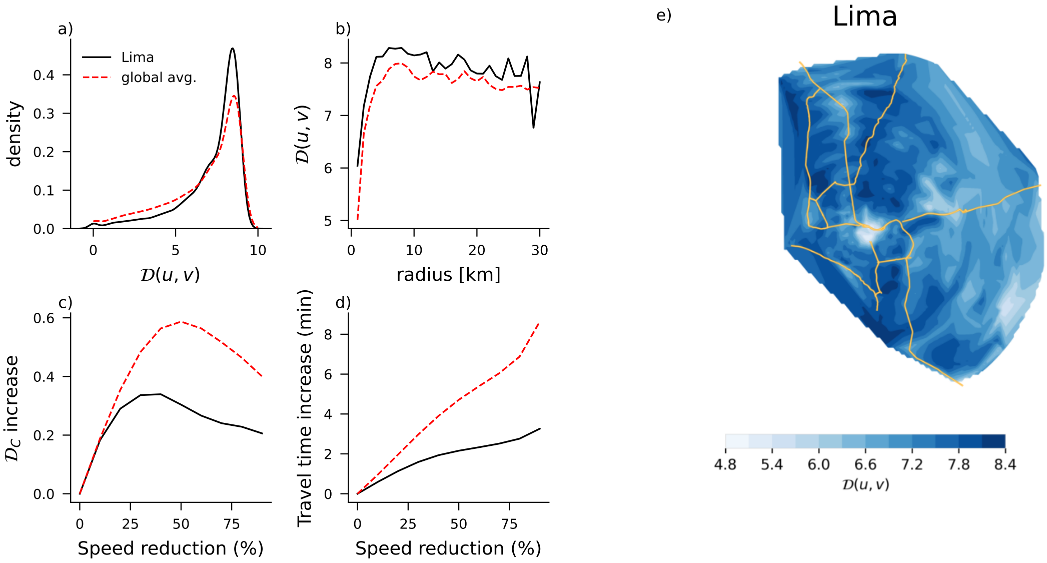


Figure S50: **Summary of DiverCity in Lima.** DiverCity trends in Lima (black solid line) compared to global averages (red dashed line) are shown for: (a) the distribution of $\mathcal{D}(u, v)$, highlighting intra-city variability; (b) $\mathcal{D}(u, v)$ as a function of radial distance from the city center; (c) the increase in DiverCity ($\mathcal{D}_C$) as a function of attractor speed reduction percentages; (d) the increase in travel time as a function of attractor speed reduction percentages; (e) The spatial distribution of $\mathcal{D}(u, v)$ across Lima provides a geographical perspective on route diversification within the city, with mobility attractor roads shown in orange.

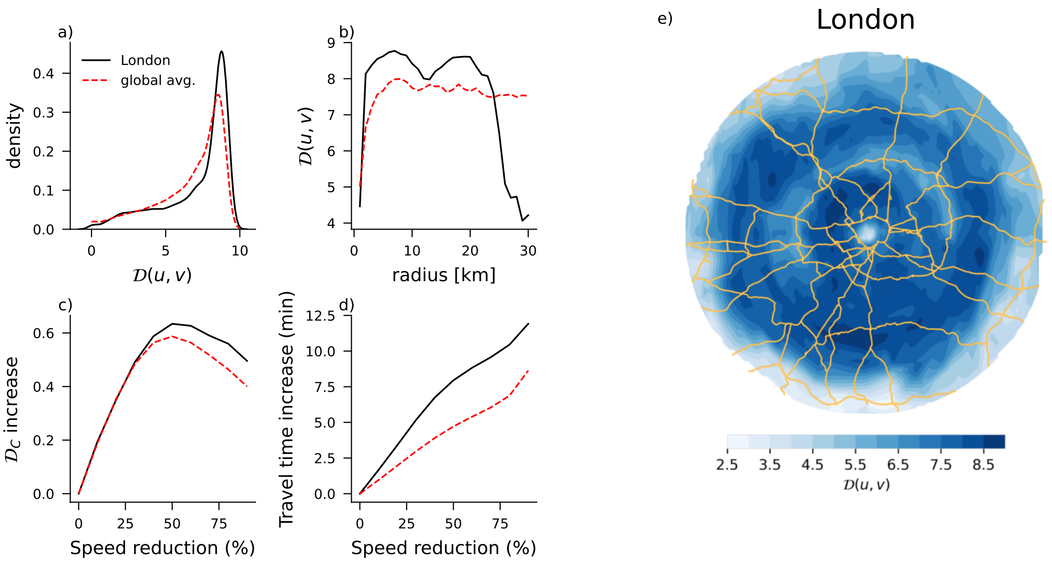


Figure S51: **Summary of DiverCity in London.** DiverCity trends in London (black solid line) compared to global averages (red dashed line) are shown for: (a) the distribution of $\mathcal{D}(u, v)$, highlighting intra-city variability; (b) $\mathcal{D}(u, v)$ as a function of radial distance from the city center; (c) the increase in DiverCity ($\mathcal{D}_C$) as a function of attractor speed reduction percentages; (d) the increase in travel time as a function of attractor speed reduction percentages; (e) The spatial distribution of $\mathcal{D}(u, v)$ across London provides a geographical perspective on route diversification within the city, with mobility attractor roads shown in orange.

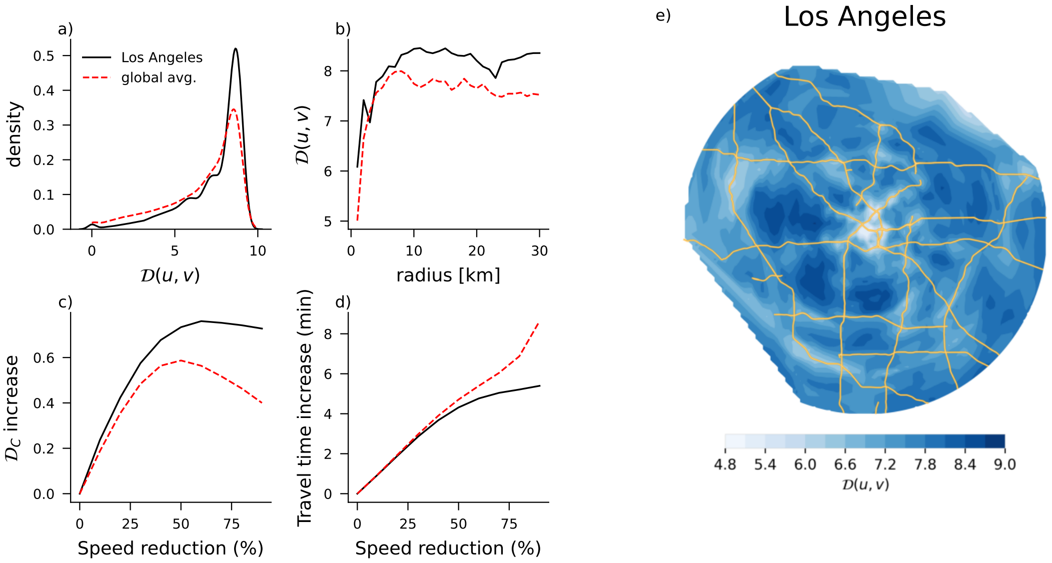


Figure S52: **Summary of DiverCity in Los Angeles.** DiverCity trends in Los Angeles (black solid line) compared to global averages (red dashed line) are shown for: (a) the distribution of $\mathcal{D}(u,v)$, highlighting intra-city variability; (b) $\mathcal{D}(u,v)$ as a function of radial distance from the city center; (c) the increase in DiverCity ($\mathcal{D}_C$) as a function of attractor speed reduction percentages; (d) the increase in travel time as a function of attractor speed reduction percentages; (e) The spatial distribution of $\mathcal{D}(u,v)$ across Los Angeles provides a geographical perspective on route diversification within the city, with mobility attractor roads shown in orange.

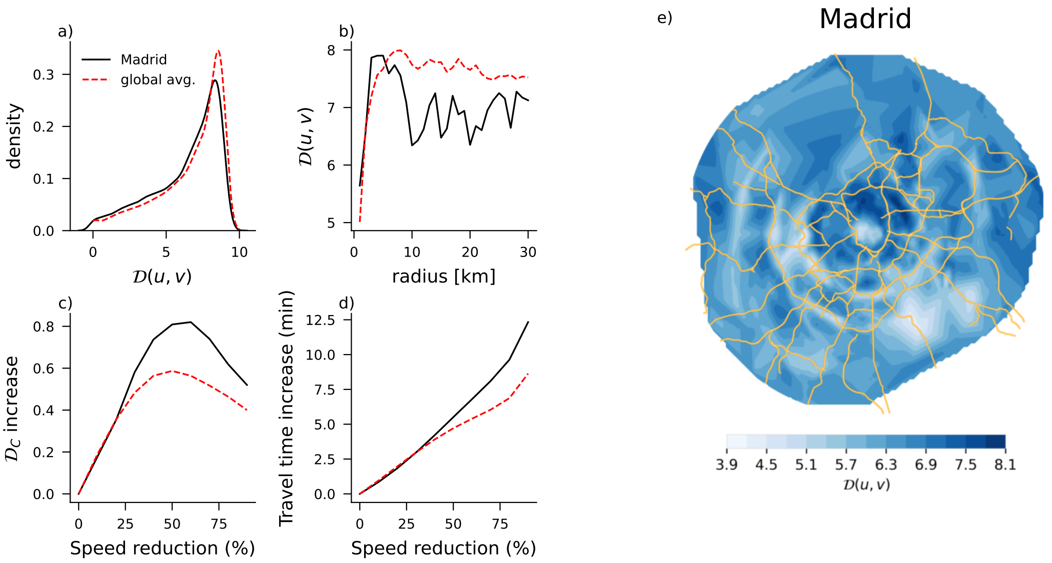


Figure S53: **Summary of DiverCity in Madrid.** DiverCity trends in Madrid (black solid line) compared to global averages (red dashed line) are shown for: (a) the distribution of $\mathcal{D}(u,v)$, highlighting intra-city variability; (b) $\mathcal{D}(u,v)$ as a function of radial distance from the city center; (c) the increase in DiverCity ($\mathcal{D}_C$) as a function of attractor speed reduction percentages; (d) the increase in travel time as a function of attractor speed reduction percentages; (e) The spatial distribution of $\mathcal{D}(u,v)$ across Madrid provides a geographical perspective on route diversification within the city, with mobility attractor roads shown in orange.

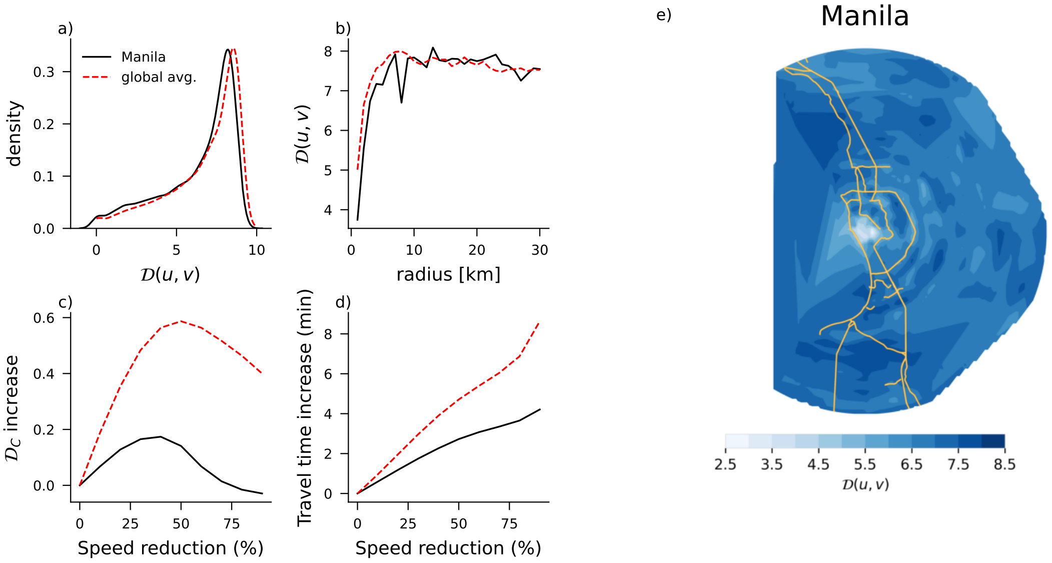


Figure S54: **Summary of DiverCity in Manila.** DiverCity trends in Manila (black solid line) compared to global averages (red dashed line) are shown for: (a) the distribution of $\mathcal{D}(u, v)$, highlighting intra-city variability; (b) $\mathcal{D}(u, v)$ as a function of radial distance from the city center; (c) the increase in DiverCity ($\mathcal{D}_C$) as a function of attractor speed reduction percentages; (d) the increase in travel time as a function of attractor speed reduction percentages; (e) The spatial distribution of $\mathcal{D}(u, v)$ across Manila provides a geographical perspective on route diversification within the city, with mobility attractor roads shown in orange.

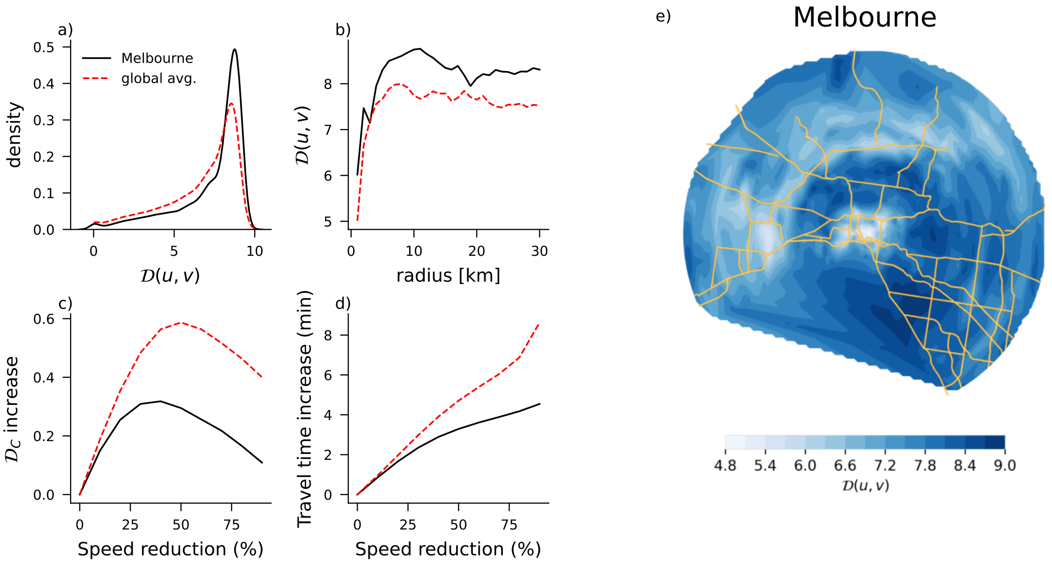


Figure S55: **Summary of DiverCity in Melbourne.** DiverCity trends in Melbourne (black solid line) compared to global averages (red dashed line) are shown for: (a) the distribution of $\mathcal{D}(u, v)$, highlighting intra-city variability; (b) $\mathcal{D}(u, v)$ as a function of radial distance from the city center; (c) the increase in DiverCity ($\mathcal{D}_C$) as a function of attractor speed reduction percentages; (d) the increase in travel time as a function of attractor speed reduction percentages; (e) The spatial distribution of $\mathcal{D}(u, v)$ across Melbourne provides a geographical perspective on route diversification within the city, with mobility attractor roads shown in orange.

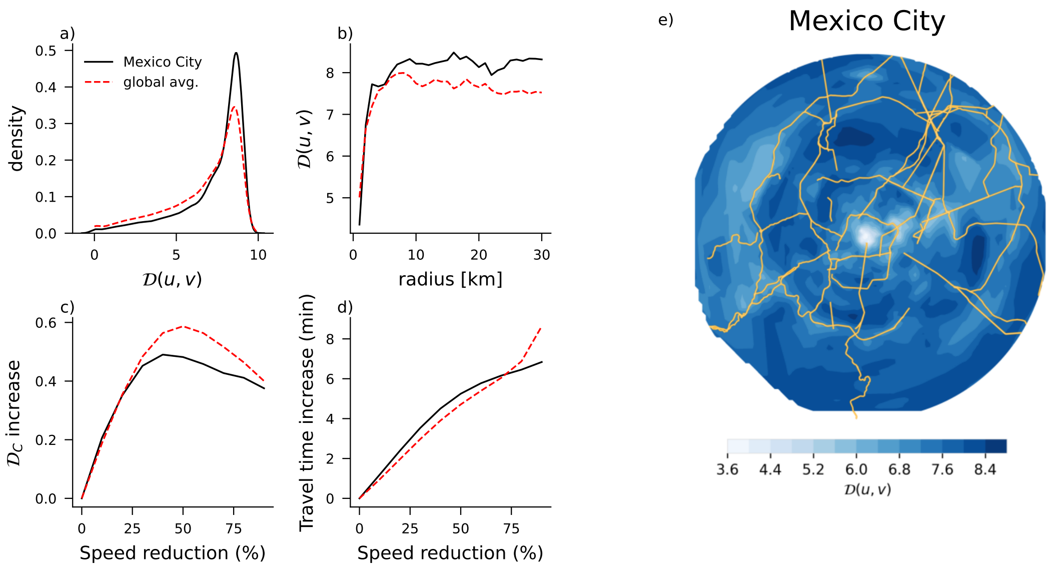


Figure S56: **Summary of DiverCity in Mexico City.** DiverCity trends in Mexico City (black solid line) compared to global averages (red dashed line) are shown for: (a) the distribution of $\mathcal{D}(u, v)$, highlighting intra-city variability; (b) $\mathcal{D}(u, v)$ as a function of radial distance from the city center; (c) the increase in DiverCity ($\mathcal{D}_C$) as a function of attractor speed reduction percentages; (d) the increase in travel time as a function of attractor speed reduction percentages; (e) The spatial distribution of $\mathcal{D}(u, v)$ across Mexico City provides a geographical perspective on route diversification within the city, with mobility attractor roads shown in orange.

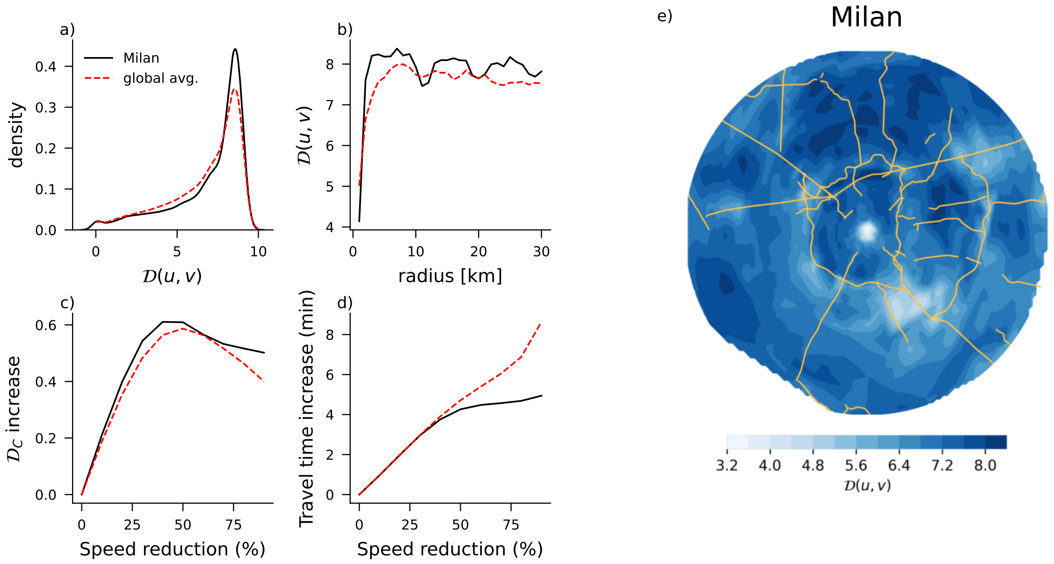


Figure S57: **Summary of DiverCity in Milan.** DiverCity trends in Milan (black solid line) compared to global averages (red dashed line) are shown for: (a) the distribution of $\mathcal{D}(u, v)$, highlighting intra-city variability; (b) $\mathcal{D}(u, v)$ as a function of radial distance from the city center; (c) the increase in DiverCity ($\mathcal{D}_C$) as a function of attractor speed reduction percentages; (d) the increase in travel time as a function of attractor speed reduction percentages; (e) The spatial distribution of $\mathcal{D}(u, v)$ across Milan provides a geographical perspective on route diversification within the city, with mobility attractor roads shown in orange.

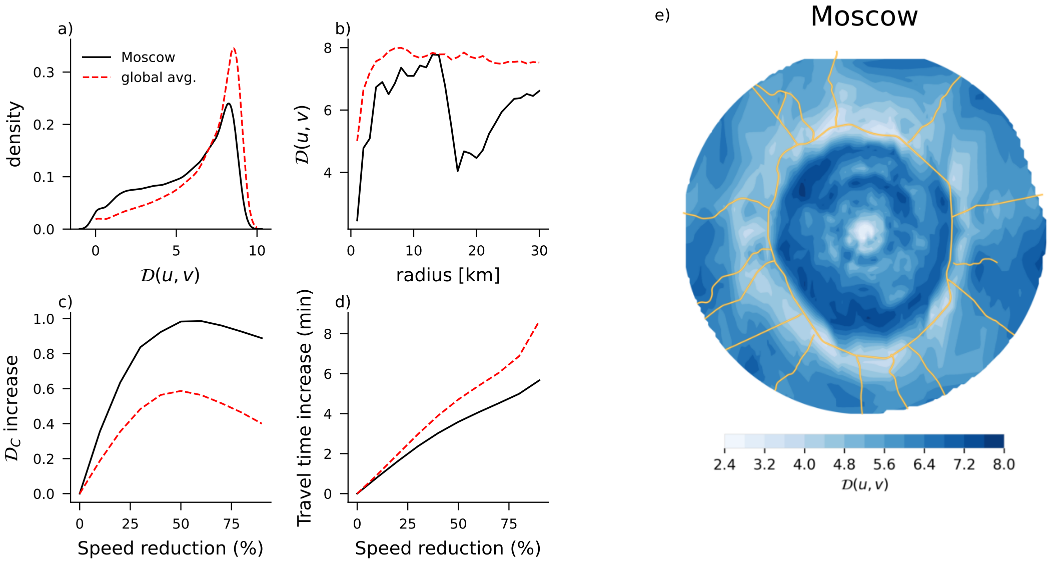


Figure S58: **Summary of DiverCity in Moscow.** DiverCity trends in Moscow (black solid line) compared to global averages (red dashed line) are shown for: (a) the distribution of $\mathcal{D}(u, v)$, highlighting intra-city variability; (b) $\mathcal{D}(u, v)$ as a function of radial distance from the city center; (c) the increase in DiverCity ($\mathcal{D}_C$) as a function of attractor speed reduction percentages; (d) the increase in travel time as a function of attractor speed reduction percentages; (e) The spatial distribution of $\mathcal{D}(u, v)$ across Moscow provides a geographical perspective on route diversification within the city, with mobility attractor roads shown in orange.

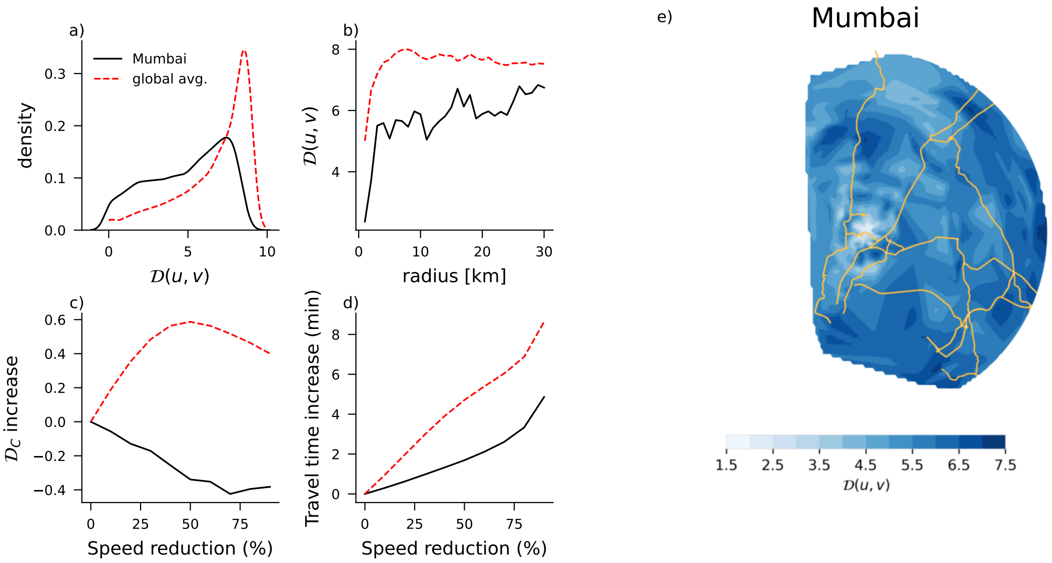


Figure S59: **Summary of DiverCity in Mumbai.** DiverCity trends in Mumbai (black solid line) compared to global averages (red dashed line) are shown for: (a) the distribution of $\mathcal{D}(u, v)$, highlighting intra-city variability; (b) $\mathcal{D}(u, v)$ as a function of radial distance from the city center; (c) the increase in DiverCity ($\mathcal{D}_C$) as a function of attractor speed reduction percentages; (d) the increase in travel time as a function of attractor speed reduction percentages; (e) The spatial distribution of $\mathcal{D}(u, v)$ across Mumbai provides a geographical perspective on route diversification within the city, with mobility attractor roads shown in orange.

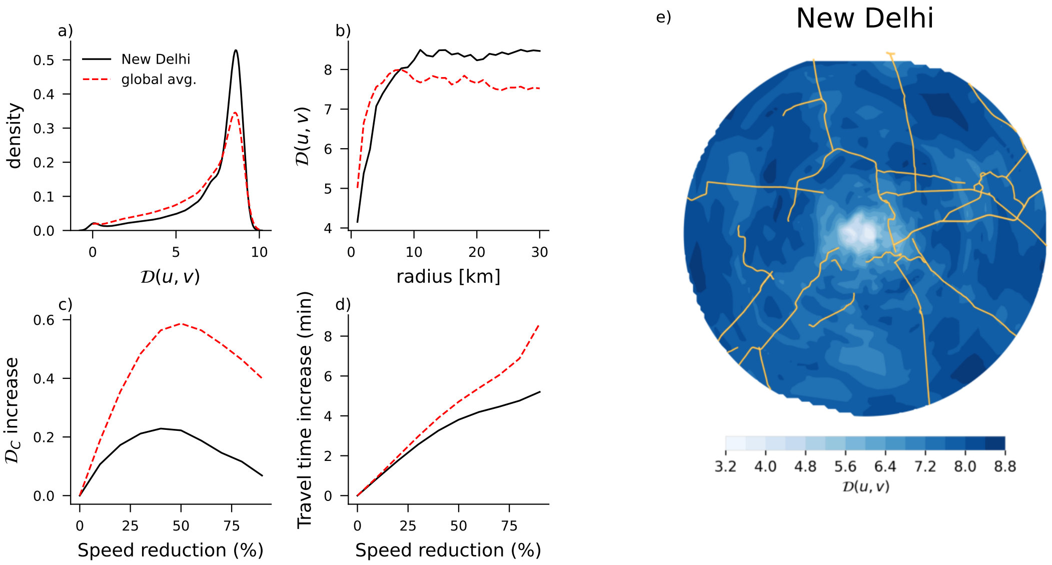


Figure S60: **Summary of DiverCity in New Delhi.** DiverCity trends in New Delhi (black solid line) compared to global averages (red dashed line) are shown for: (a) the distribution of $\mathcal{D}(u, v)$, highlighting intra-city variability; (b) $\mathcal{D}(u, v)$ as a function of radial distance from the city center; (c) the increase in DiverCity ($\mathcal{D}_C$) as a function of attractor speed reduction percentages; (d) the increase in travel time as a function of attractor speed reduction percentages; (e) The spatial distribution of $\mathcal{D}(u, v)$ across New Delhi provides a geographical perspective on route diversification within the city, with mobility attractor roads shown in orange.

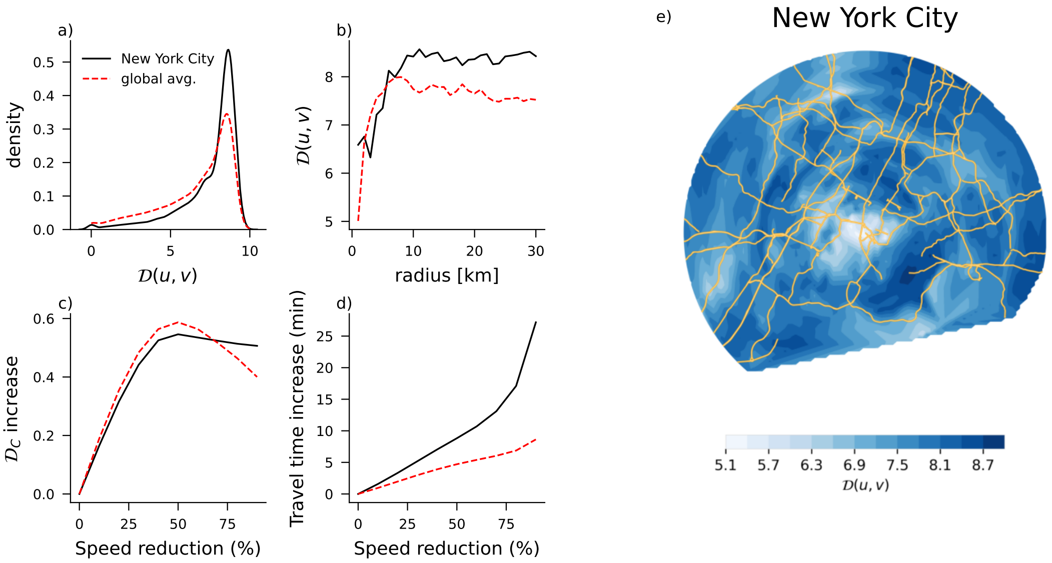


Figure S61: **Summary of DiverCity in New York City.** DiverCity trends in New York City (black solid line) compared to global averages (red dashed line) are shown for: (a) the distribution of $\mathcal{D}(u, v)$, highlighting intra-city variability; (b) $\mathcal{D}(u, v)$ as a function of radial distance from the city center; (c) the increase in DiverCity ($\mathcal{D}_C$) as a function of attractor speed reduction percentages; (d) the increase in travel time as a function of attractor speed reduction percentages; (e) The spatial distribution of $\mathcal{D}(u, v)$ across New York City provides a geographical perspective on route diversification within the city, with mobility attractor roads shown in orange.

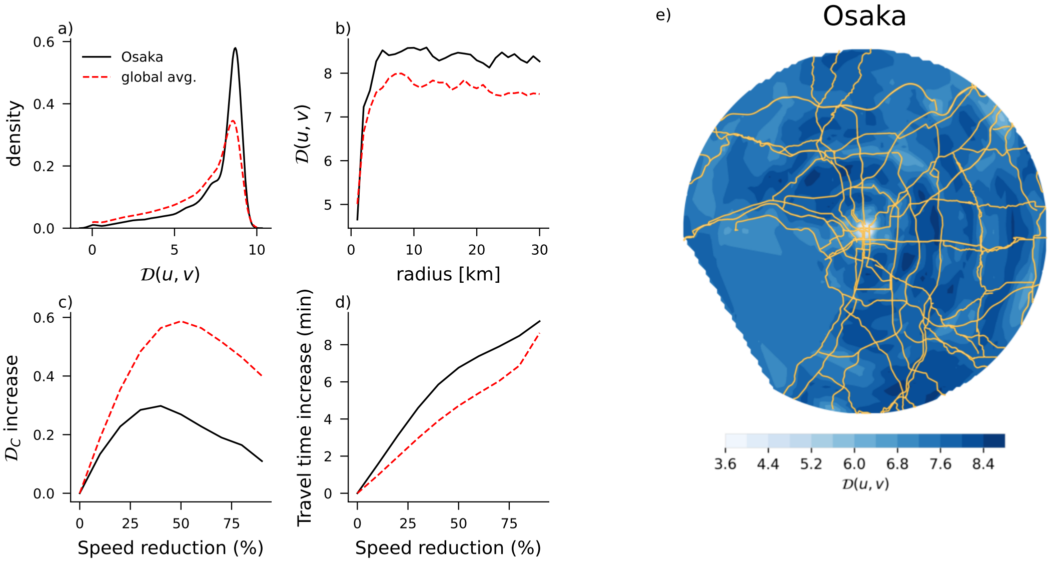


Figure S62: **Summary of DiverCity in Osaka.** DiverCity trends in Osaka (black solid line) compared to global averages (red dashed line) are shown for: (a) the distribution of $\mathcal{D}(u,v)$, highlighting intra-city variability; (b) $\mathcal{D}(u,v)$ as a function of radial distance from the city center; (c) the increase in DiverCity ($\mathcal{D}_C$) as a function of attractor speed reduction percentages; (d) the increase in travel time as a function of attractor speed reduction percentages; (e) The spatial distribution of $\mathcal{D}(u,v)$ across Osaka provides a geographical perspective on route diversification within the city, with mobility attractor roads shown in orange.

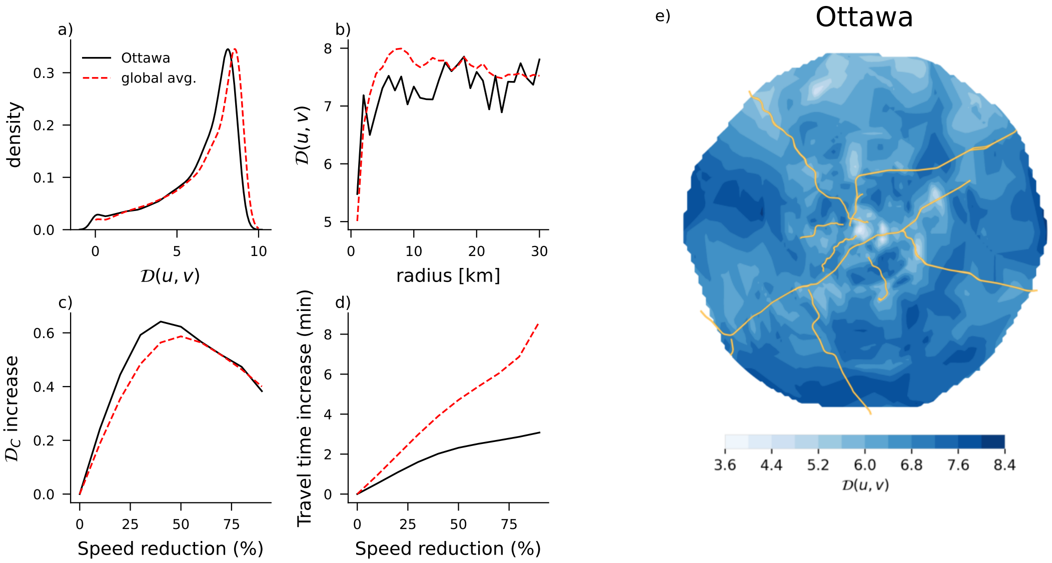


Figure S63: **Summary of DiverCity in Ottawa.** DiverCity trends in Ottawa (black solid line) compared to global averages (red dashed line) are shown for: (a) the distribution of $\mathcal{D}(u,v)$, highlighting intra-city variability; (b) $\mathcal{D}(u,v)$ as a function of radial distance from the city center; (c) the increase in DiverCity ($\mathcal{D}_C$) as a function of attractor speed reduction percentages; (d) the increase in travel time as a function of attractor speed reduction percentages; (e) The spatial distribution of $\mathcal{D}(u,v)$ across Ottawa provides a geographical perspective on route diversification within the city, with mobility attractor roads shown in orange.

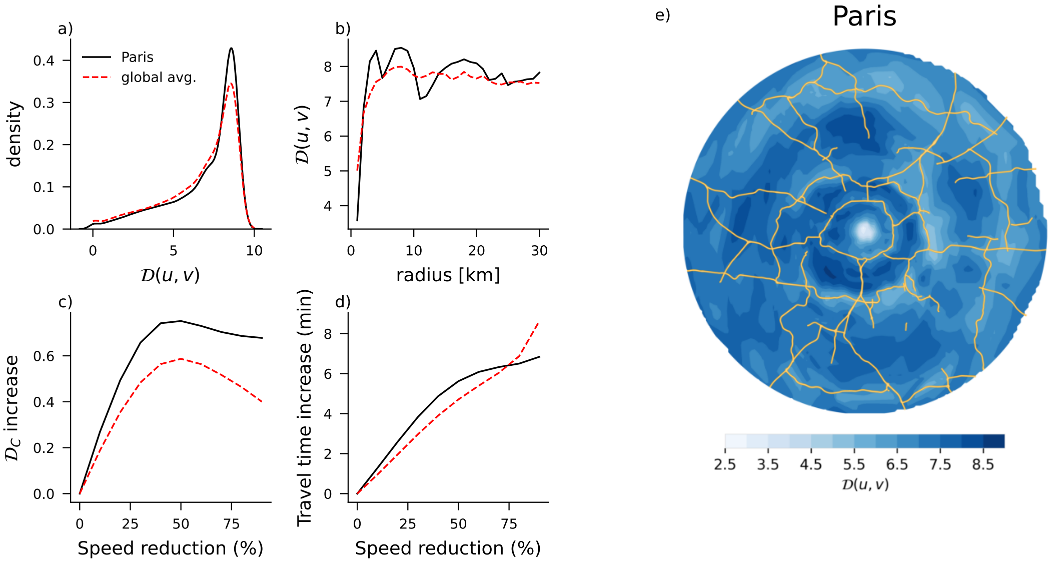


Figure S64: **Summary of DiverCity in Paris.** DiverCity trends in Paris (black solid line) compared to global averages (red dashed line) are shown for: (a) the distribution of $\mathcal{D}(u, v)$, highlighting intra-city variability; (b) $\mathcal{D}(u, v)$ as a function of radial distance from the city center; (c) the increase in DiverCity ($\mathcal{D}_C$) as a function of attractor speed reduction percentages; (d) the increase in travel time as a function of attractor speed reduction percentages; (e) The spatial distribution of $\mathcal{D}(u, v)$ across Paris provides a geographical perspective on route diversification within the city, with mobility attractor roads shown in orange.

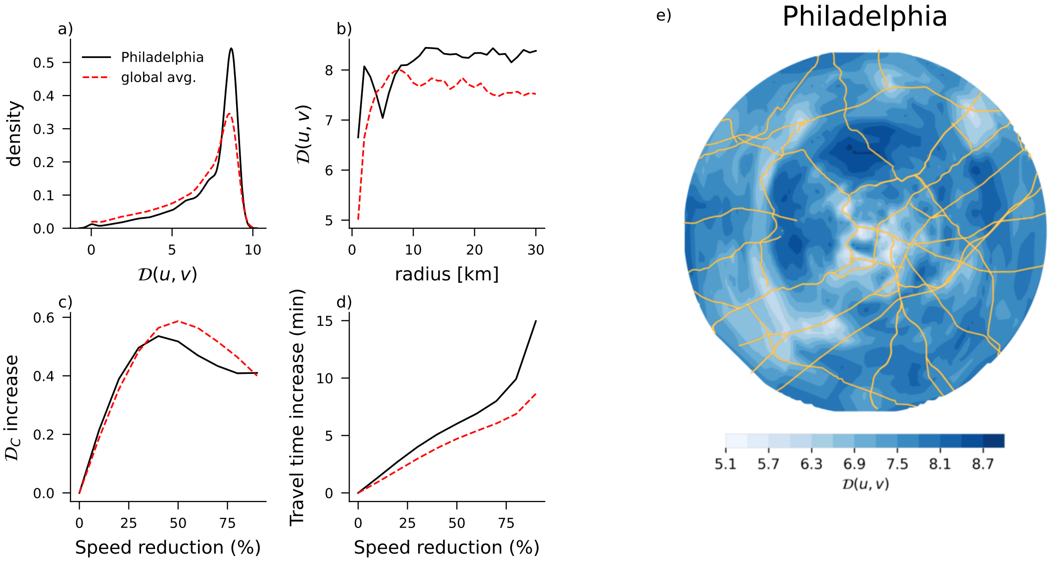


Figure S65: **Summary of DiverCity in Philadelphia.** DiverCity trends in Philadelphia (black solid line) compared to global averages (red dashed line) are shown for: (a) the distribution of $\mathcal{D}(u, v)$, highlighting intra-city variability; (b) $\mathcal{D}(u, v)$ as a function of radial distance from the city center; (c) the increase in DiverCity ($\mathcal{D}_C$) as a function of attractor speed reduction percentages; (d) the increase in travel time as a function of attractor speed reduction percentages; (e) The spatial distribution of $\mathcal{D}(u, v)$ across Philadelphia provides a geographical perspective on route diversification within the city, with mobility attractor roads shown in orange.

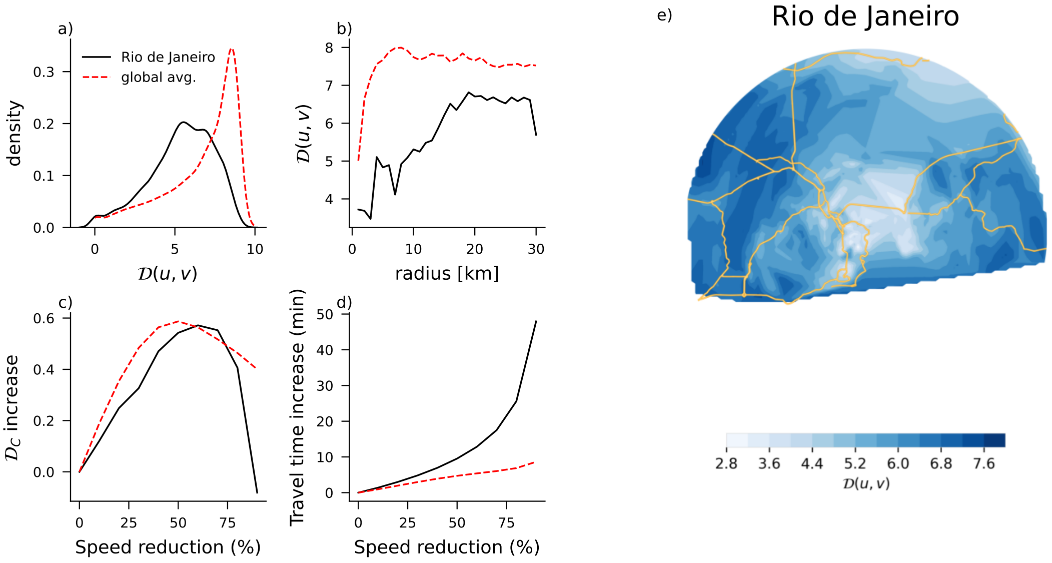


Figure S66: **Summary of DiverCity in Rio de Janeiro.** DiverCity trends in Rio de Janeiro (black solid line) compared to global averages (red dashed line) are shown for: (a) the distribution of $\mathcal{D}(u, v)$, highlighting intra-city variability; (b) $\mathcal{D}(u, v)$ as a function of radial distance from the city center; (c) the increase in DiverCity ($\mathcal{D}_C$) as a function of attractor speed reduction percentages; (d) the increase in travel time as a function of attractor speed reduction percentages; (e) The spatial distribution of $\mathcal{D}(u, v)$ across Rio de Janeiro provides a geographical perspective on route diversification within the city, with mobility attractor roads shown in orange.

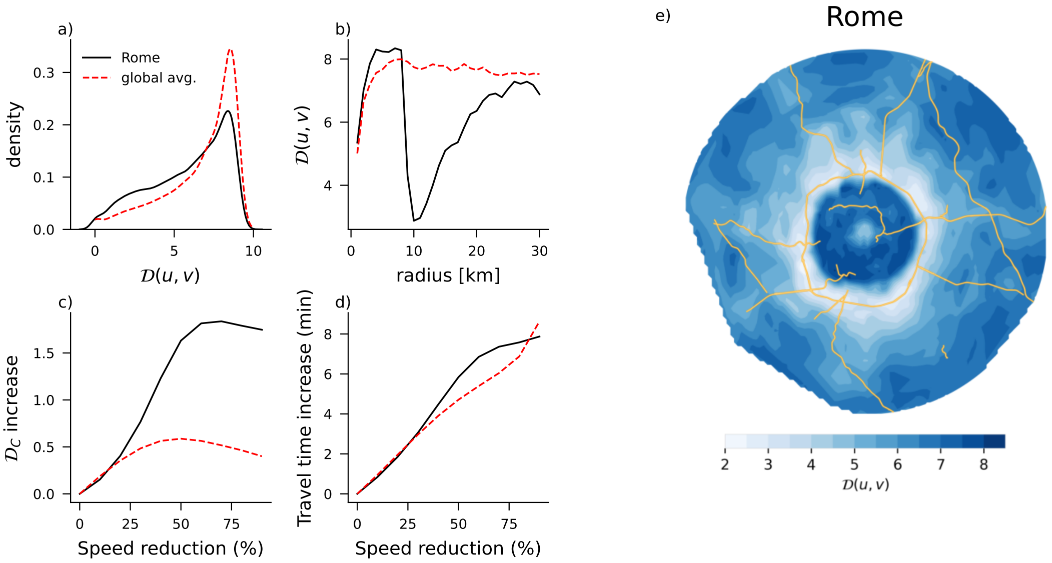


Figure S67: **Summary of DiverCity in Rome.** DiverCity trends in Rome (black solid line) compared to global averages (red dashed line) are shown for: (a) the distribution of $\mathcal{D}(u, v)$, highlighting intra-city variability; (b) $\mathcal{D}(u, v)$ as a function of radial distance from the city center; (c) the increase in DiverCity ($\mathcal{D}_C$) as a function of attractor speed reduction percentages; (d) the increase in travel time as a function of attractor speed reduction percentages; (e) The spatial distribution of $\mathcal{D}(u, v)$ across Rome provides a geographical perspective on route diversification within the city, with mobility attractor roads shown in orange.

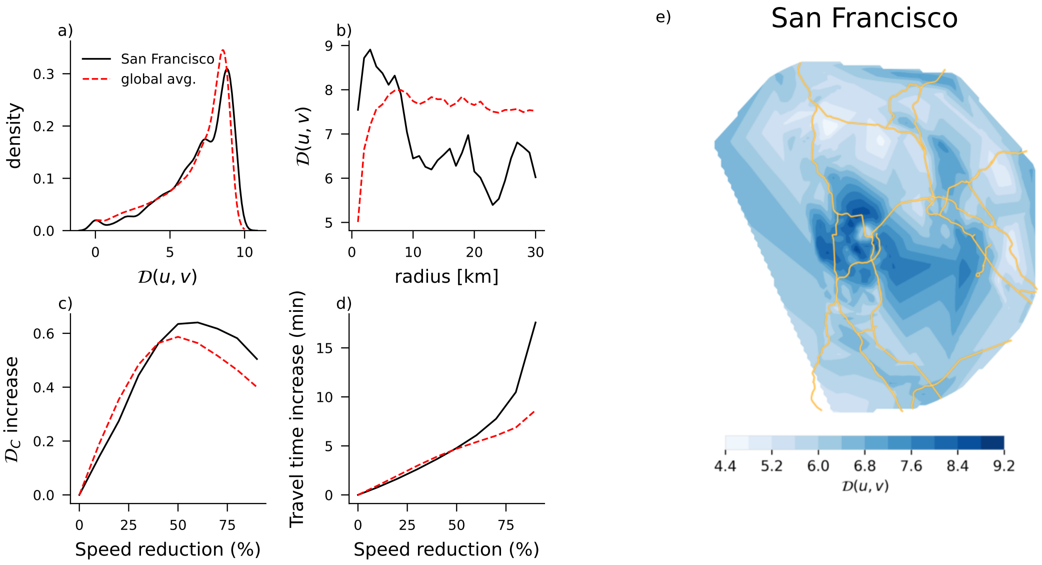


Figure S68: **Summary of DiverCity in San Francisco.** DiverCity trends in San Francisco (black solid line) compared to global averages (red dashed line) are shown for: (a) the distribution of $\mathcal{D}(u, v)$, highlighting intra-city variability; (b) $\mathcal{D}(u, v)$ as a function of radial distance from the city center; (c) the increase in DiverCity ($\mathcal{D}_C$) as a function of attractor speed reduction percentages; (d) the increase in travel time as a function of attractor speed reduction percentages; (e) The spatial distribution of $\mathcal{D}(u, v)$ across San Francisco provides a geographical perspective on route diversification within the city, with mobility attractor roads shown in orange.

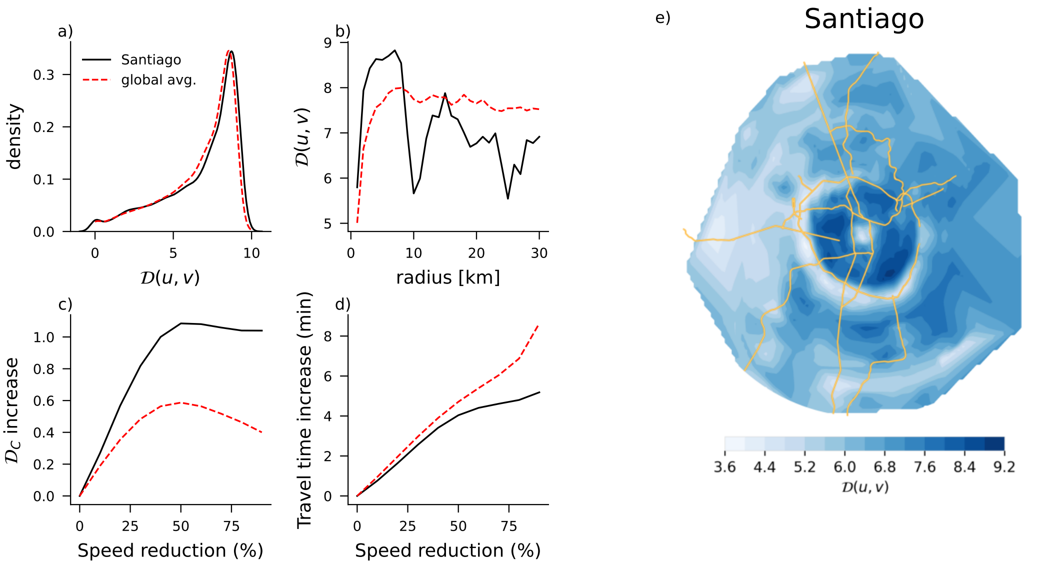


Figure S69: **Summary of DiverCity in Santiago.** DiverCity trends in Santiago (black solid line) compared to global averages (red dashed line) are shown for: (a) the distribution of $\mathcal{D}(u, v)$, highlighting intra-city variability; (b) $\mathcal{D}(u, v)$ as a function of radial distance from the city center; (c) the increase in DiverCity ($\mathcal{D}_C$) as a function of attractor speed reduction percentages; (d) the increase in travel time as a function of attractor speed reduction percentages; (e) The spatial distribution of $\mathcal{D}(u, v)$ across Santiago provides a geographical perspective on route diversification within the city, with mobility attractor roads shown in orange.

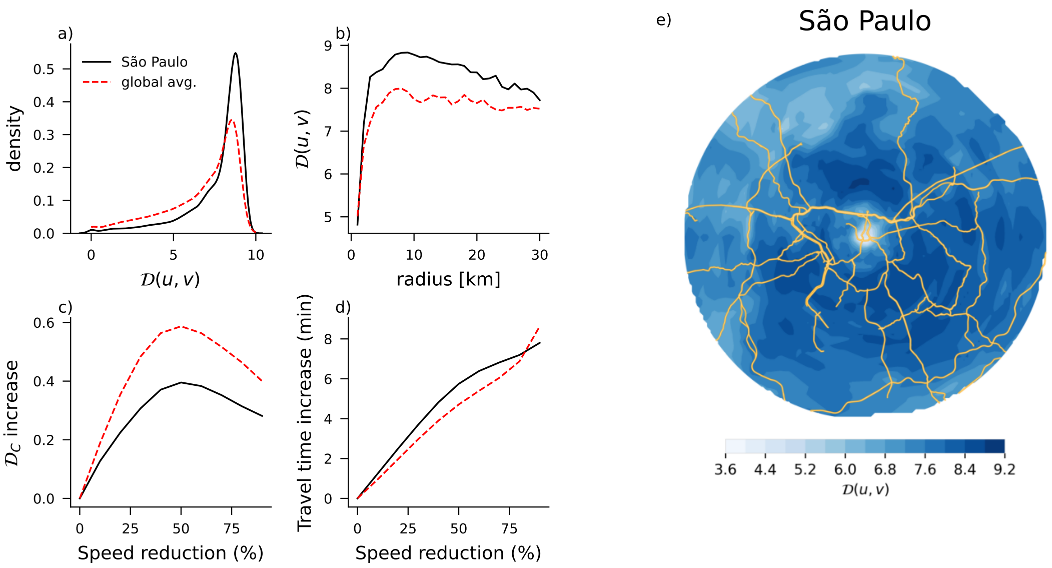


Figure S70: **Summary of DiverCity in São Paulo.** DiverCity trends in São Paulo (black solid line) compared to global averages (red dashed line) are shown for: (a) the distribution of $\mathcal{D}(u,v)$, highlighting intra-city variability; (b) $\mathcal{D}(u,v)$ as a function of radial distance from the city center; (c) the increase in DiverCity ($\mathcal{D}_C$) as a function of attractor speed reduction percentages; (d) the increase in travel time as a function of attractor speed reduction percentages; (e) The spatial distribution of $\mathcal{D}(u,v)$ across São Paulo provides a geographical perspective on route diversification within the city, with mobility attractor roads shown in orange.

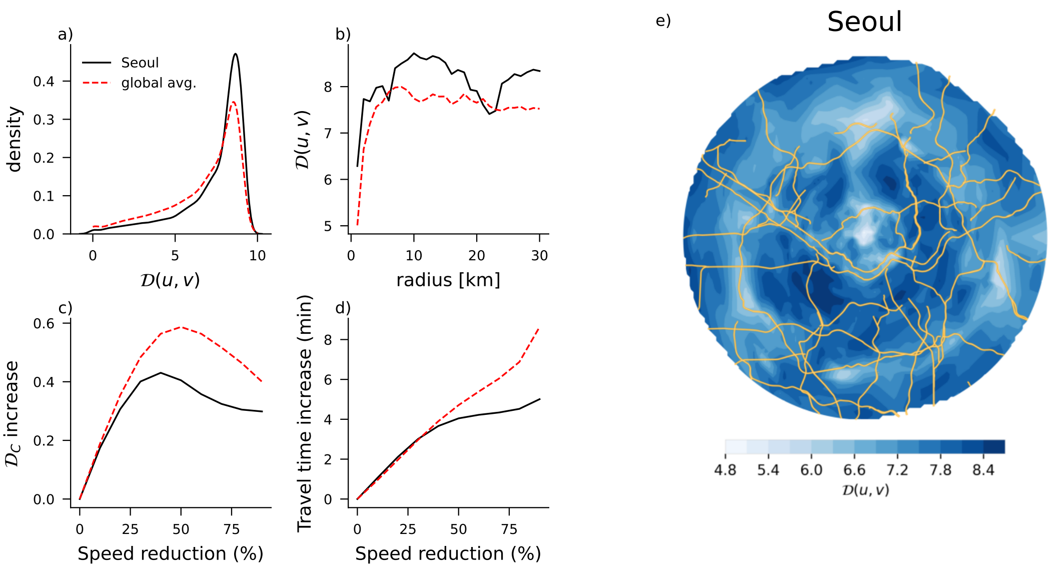


Figure S71: **Summary of DiverCity in Seoul.** DiverCity trends in Seoul (black solid line) compared to global averages (red dashed line) are shown for: (a) the distribution of $\mathcal{D}(u,v)$, highlighting intra-city variability; (b) $\mathcal{D}(u,v)$ as a function of radial distance from the city center; (c) the increase in DiverCity ($\mathcal{D}_C$) as a function of attractor speed reduction percentages; (d) the increase in travel time as a function of attractor speed reduction percentages; (e) The spatial distribution of $\mathcal{D}(u,v)$ across Seoul provides a geographical perspective on route diversification within the city, with mobility attractor roads shown in orange.

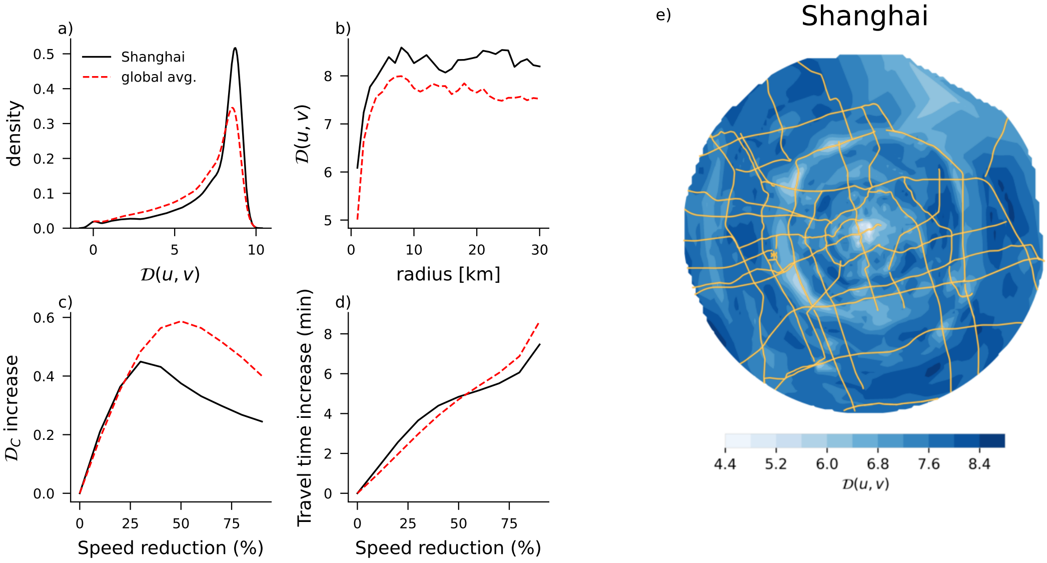


Figure S72: **Summary of DiverCity in Shanghai.** DiverCity trends in Shanghai (black solid line) compared to global averages (red dashed line) are shown for: (a) the distribution of $\mathcal{D}(u, v)$, highlighting intra-city variability; (b) $\mathcal{D}(u, v)$ as a function of radial distance from the city center; (c) the increase in DiverCity ($\mathcal{D}_C$) as a function of attractor speed reduction percentages; (d) the increase in travel time as a function of attractor speed reduction percentages; (e) The spatial distribution of $\mathcal{D}(u, v)$ across Shanghai provides a geographical perspective on route diversification within the city, with mobility attractor roads shown in orange.

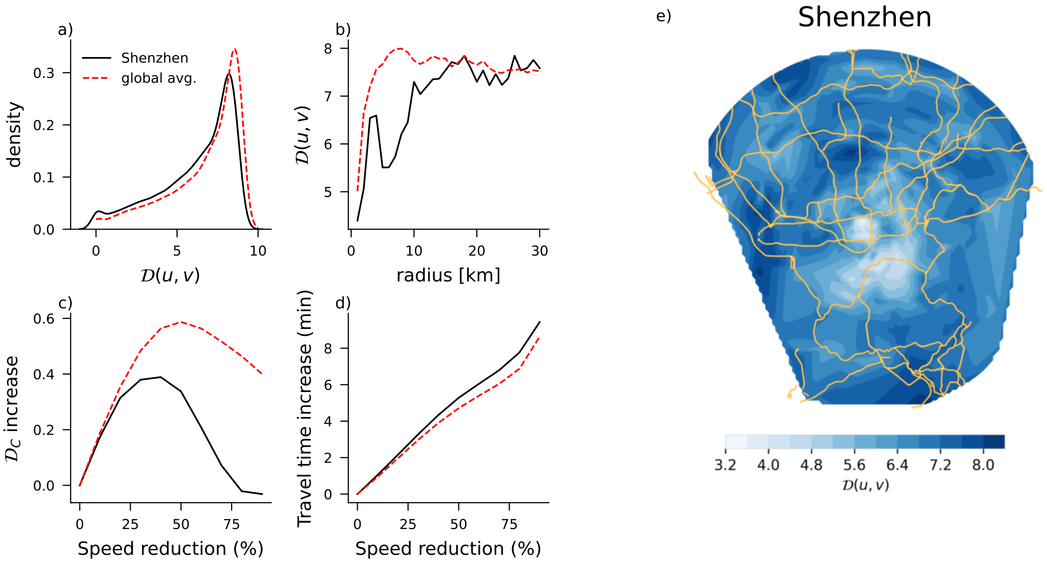


Figure S73: **Summary of DiverCity in Shenzhen.** DiverCity trends in Shenzhen (black solid line) compared to global averages (red dashed line) are shown for: (a) the distribution of $\mathcal{D}(u, v)$, highlighting intra-city variability; (b) $\mathcal{D}(u, v)$ as a function of radial distance from the city center; (c) the increase in DiverCity ($\mathcal{D}_C$) as a function of attractor speed reduction percentages; (d) the increase in travel time as a function of attractor speed reduction percentages; (e) The spatial distribution of $\mathcal{D}(u, v)$ across Shenzhen provides a geographical perspective on route diversification within the city, with mobility attractor roads shown in orange.

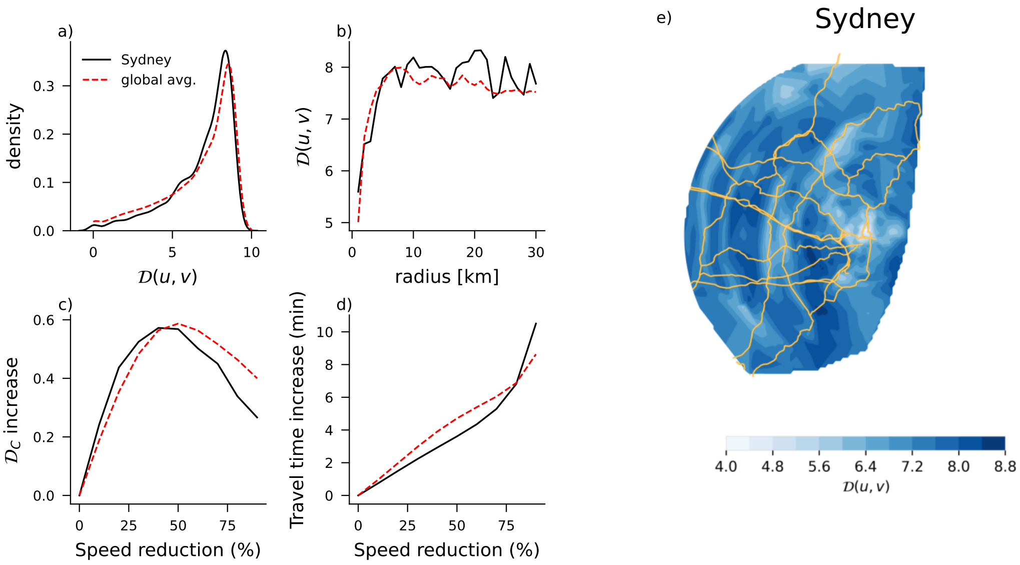


Figure S74: **Summary of DiverCity in Sydney.** DiverCity trends in Sydney (black solid line) compared to global averages (red dashed line) are shown for: (a) the distribution of $\mathcal{D}(u, v)$, highlighting intra-city variability; (b) $\mathcal{D}(u, v)$ as a function of radial distance from the city center; (c) the increase in DiverCity ($\mathcal{D}_C$) as a function of attractor speed reduction percentages; (d) the increase in travel time as a function of attractor speed reduction percentages; (e) The spatial distribution of $\mathcal{D}(u, v)$ across Sydney provides a geographical perspective on route diversification within the city, with mobility attractor roads shown in orange.

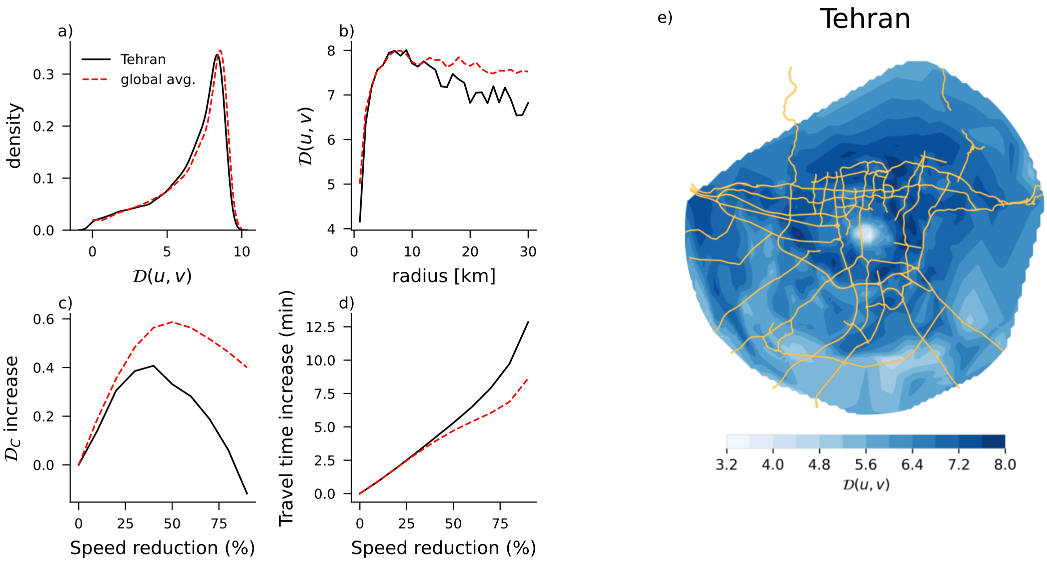


Figure S75: **Summary of DiverCity in Tehran.** DiverCity trends in Tehran (black solid line) compared to global averages (red dashed line) are shown for: (a) the distribution of $\mathcal{D}(u, v)$, highlighting intra-city variability; (b) $\mathcal{D}(u, v)$ as a function of radial distance from the city center; (c) the increase in DiverCity ($\mathcal{D}_C$) as a function of attractor speed reduction percentages; (d) the increase in travel time as a function of attractor speed reduction percentages; (e) The spatial distribution of $\mathcal{D}(u, v)$ across Tehran provides a geographical perspective on route diversification within the city, with mobility attractor roads shown in orange.

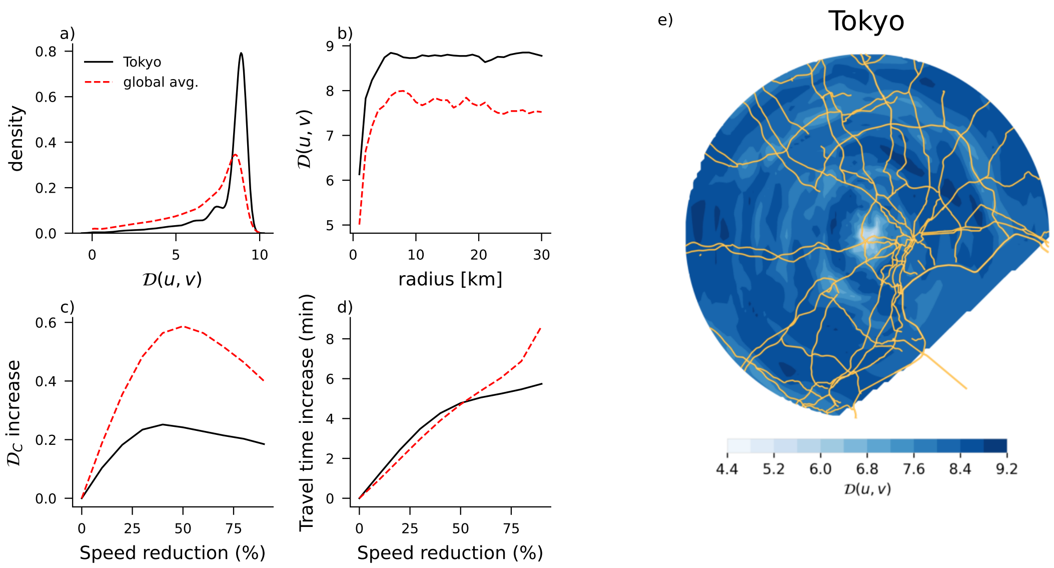


Figure S76: **Summary of DiverCity in Tokyo.** DiverCity trends in Tokyo (black solid line) compared to global averages (red dashed line) are shown for: (a) the distribution of $\mathcal{D}(u, v)$, highlighting intra-city variability; (b) $\mathcal{D}(u, v)$ as a function of radial distance from the city center; (c) the increase in DiverCity ($\mathcal{D}_C$) as a function of attractor speed reduction percentages; (d) the increase in travel time as a function of attractor speed reduction percentages; (e) The spatial distribution of $\mathcal{D}(u, v)$ across Tokyo provides a geographical perspective on route diversification within the city, with mobility attractor roads shown in orange.

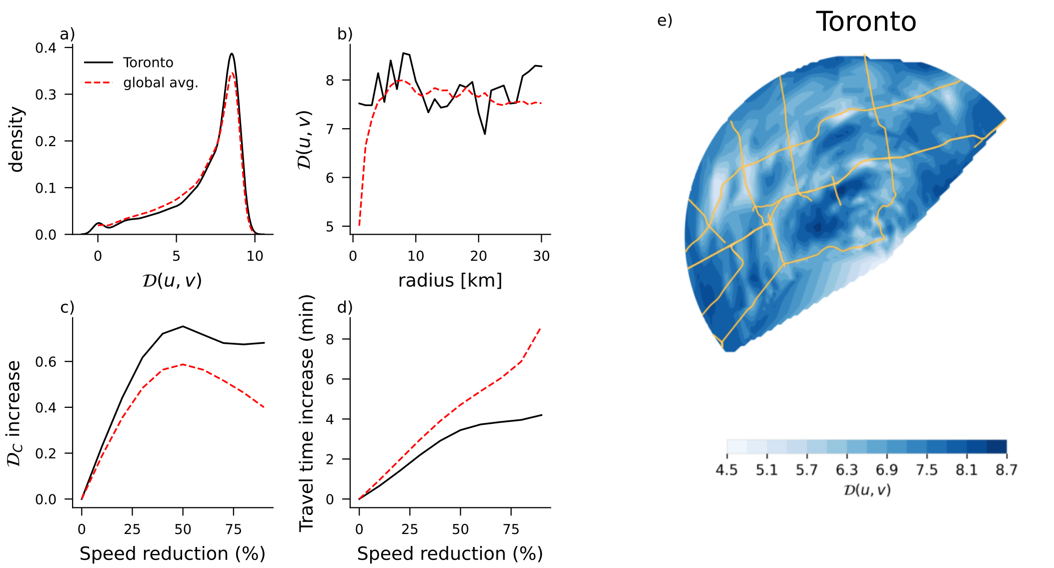


Figure S77: **Summary of DiverCity in Toronto.** DiverCity trends in Toronto (black solid line) compared to global averages (red dashed line) are shown for: (a) the distribution of $\mathcal{D}(u, v)$, highlighting intra-city variability; (b) $\mathcal{D}(u, v)$ as a function of radial distance from the city center; (c) the increase in DiverCity ($\mathcal{D}_C$) as a function of attractor speed reduction percentages; (d) the increase in travel time as a function of attractor speed reduction percentages; (e) The spatial distribution of $\mathcal{D}(u, v)$ across Toronto provides a geographical perspective on route diversification within the city, with mobility attractor roads shown in orange.

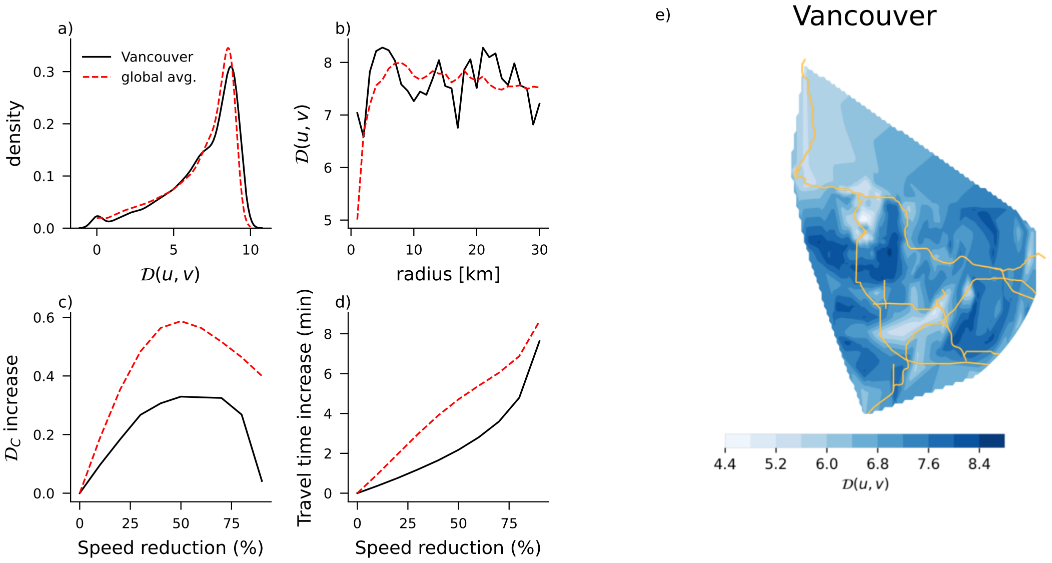


Figure S78: **Summary of DiverCity in Vancouver.** DiverCity trends in Vancouver (black solid line) compared to global averages (red dashed line) are shown for: (a) the distribution of $\mathcal{D}(u, v)$, highlighting intra-city variability; (b) $\mathcal{D}(u, v)$ as a function of radial distance from the city center; (c) the increase in DiverCity ($\mathcal{D}_C$) as a function of attractor speed reduction percentages; (d) the increase in travel time as a function of attractor speed reduction percentages; (e) The spatial distribution of $\mathcal{D}(u, v)$ across Vancouver provides a geographical perspective on route diversification within the city, with mobility attractor roads shown in orange.

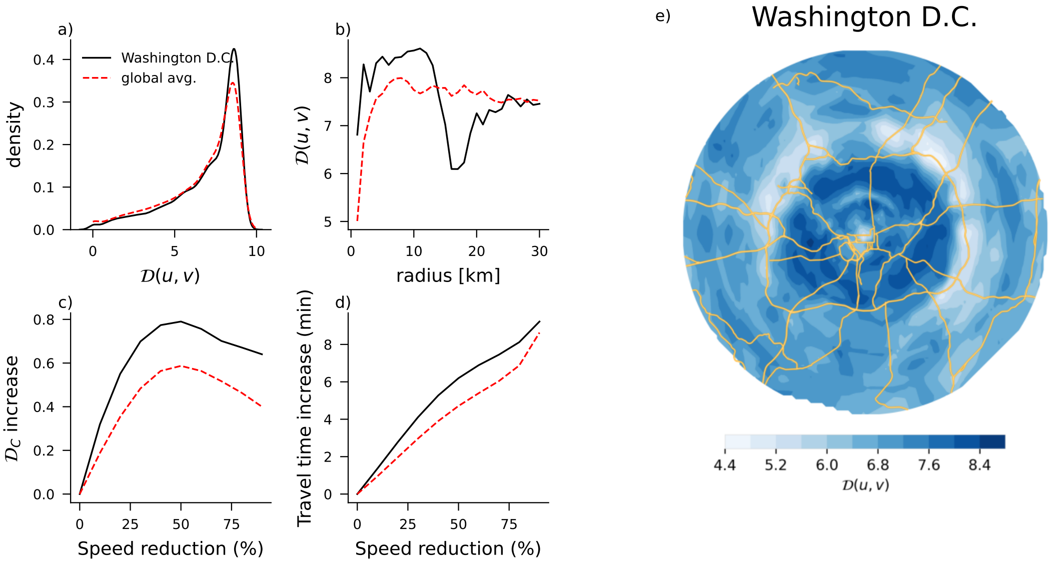


Figure S79: **Summary of DiverCity in Washington D.C..** DiverCity trends in Washington D.C. (black solid line) compared to global averages (red dashed line) are shown for: (a) the distribution of $\mathcal{D}(u, v)$, highlighting intra-city variability; (b) $\mathcal{D}(u, v)$ as a function of radial distance from the city center; (c) the increase in DiverCity ($\mathcal{D}_C$) as a function of attractor speed reduction percentages; (d) the increase in travel time as a function of attractor speed reduction percentages; (e) The spatial distribution of $\mathcal{D}(u, v)$ across Washington D.C. provides a geographical perspective on route diversification within the city, with mobility attractor roads shown in orange.

# 3 Supplementary Tables

| Rank | City | $\mathcal{D}_C$ | IQR | attractors length [km] | attractor density | H | road network length [km] | Land % | avg. Edge Load ($10^{-3}$) | avg. edge length [m] | avg. streets/node | intersections | avg. circuity |
|---|---|---|---|---|---|---|---|---|---|---|---|---|---|
| 1 | Tokyo | 8.697 | 1.264 | 2,534 | 0.910 | 1.339 | 119,383 | 86.569 | 0.441 | 65.555 | 2.889 | 576,634 | 1.049 |
| 2 | São Paulo | 8.369 | 1.722 | 1,652 | 0.532 | 2.215 | 60,014 | 96.660 | 0.746 | 108.267 | 2.883 | 195,880 | 1.065 |
| 3 | Osaka | 8.311 | 1.905 | 2,808 | 0.992 | 1.064 | 81,108 | 88.064 | 0.561 | 71.819 | 2.875 | 354,586 | 1.066 |
| 4 | Chicago ⊞ | 8.283 | 2.591 | 799 | 0.440 | 1.769 | 36,184 | 56.466 | 0.935 | 146.370 | 3.121 | 80,565 | 1.040 |
| 5 | Melbourne ⊞ | 8.279 | 2.177 | 1,282 | 0.508 | 2.249 | 39,818 | 78.430 | 0.972 | 103.337 | 2.765 | 148,114 | 1.051 |
| 6 | New York City ⊞ | 8.257 | 1.790 | 2,128 | 0.811 | 1.381 | 52,837 | 81.591 | 0.612 | 126.825 | 3.040 | 141,379 | 1.040 |
| 7 | Shanghai | 8.231 | 2.224 | 2,012 | 0.697 | 1.422 | 34,017 | 89.777 | 0.961 | 244.134 | 3.045 | 48,669 | 1.041 |
| 8 | Philadelphia ⊞ | 8.197 | 2.134 | 1,680 | 0.528 | 1.602 | 48,573 | 98.983 | 0.943 | 153.503 | 2.929 | 104,834 | 1.071 |
| 9 | London | 8.191 | 2.820 | 2,012 | 0.632 | 1.363 | 47,797 | 99.056 | 1.092 | 104.382 | 2.491 | 145,219 | 1.065 |
| 10 | Los Angeles ⊞ | 8.174 | 2.136 | 1,278 | 0.486 | 1.762 | 56,758 | 81.802 | 0.669 | 149.014 | 2.942 | 117,979 | 1.045 |
| 11 | Seoul | 8.161 | 2.016 | 2,068 | 0.664 | 1.563 | 44,062 | 96.881 | 0.819 | 110.584 | 2.997 | 130,839 | 1.059 |
| 12 | New Delhi | 8.130 | 1.952 | 960 | 0.306 | 2.836 | 70,560 | 97.593 | 0.718 | 76.064 | 2.795 | 288,914 | 1.043 |
| 13 | Mexico City ⊞ | 8.099 | 2.115 | 1,580 | 0.533 | 2.520 | 75,000 | 92.262 | 0.697 | 85.111 | 2.720 | 278,255 | 1.044 |
| 14 | Houston ⊞ | 8.042 | 2.396 | 1,574 | 0.502 | 2.110 | 50,981 | 97.573 | 0.701 | 143.068 | 2.899 | 121,145 | 1.066 |
| 15 | Buenos Aires ⊞ | 8.022 | 3.095 | 510 | 0.291 | 3.044 | 43,942 | 54.582 | 0.689 | 105.537 | 3.423 | 139,752 | 1.011 |
| 16 | Milan | 7.939 | 2.576 | 932 | 0.299 | 2.941 | 35,285 | 96.872 | 0.980 | 111.846 | 2.752 | 124,081 | 1.062 |
| 17 | Cairo | 7.928 | 2.351 | 1,499 | 0.528 | 2.636 | 60,542 | 88.263 | 0.605 | 70.200 | 2.789 | 289,172 | 1.036 |
| 18 | Lima ⊞ | 7.926 | 1.964 | 432 | 0.272 | 3.756 | 31,714 | 49.420 | 0.967 | 82.134 | 3.004 | 129,052 | 1.046 |
| 19 | Dallas ⊞ | 7.883 | 2.517 | 1,622 | 0.518 | 1.832 | 48,563 | 97.449 | 0.702 | 151.697 | 3.013 | 113,153 | 1.061 |
| 20 | Paris | 7.854 | 2.664 | 1,341 | 0.430 | 1.906 | 41,311 | 97.057 | 0.780 | 110.415 | 2.796 | 145,462 | 1.058 |
| 21 | Toronto ⊞ | 7.796 | 2.604 | 740 | 0.417 | 2.009 | 28,988 | 55.233 | 0.969 | 162.590 | 2.970 | 60,388 | 1.122 |
| 22 | Washington D.C. ⊞ | 7.769 | 2.717 | 1,620 | 0.512 | 1.976 | 45,202 | 98.332 | 1.011 | 144.023 | 2.686 | 99,542 | 1.080 |
| 23 | Beijing ⊞ | 7.724 | 3.071 | 2,218 | 0.696 | 1.273 | 40,910 | 99.120 | 1.028 | 197.468 | 2.963 | 73,414 | 1.055 |
| 24 | Karachi | 7.689 | 2.428 | 416 | 0.240 | 4.733 | 34,193 | 53.978 | 0.765 | 75.103 | 2.992 | 142,244 | 1.029 |
| 25 | Berlin | 7.677 | 3.305 | 722 | 0.253 | 3.063 | 24,924 | 88.711 | 1.426 | 164.857 | 2.859 | 49,241 | 1.050 |
| 26 | Guangzhou | 7.676 | 2.827 | 2,749 | 0.862 | 1.035 | 37,051 | 99.152 | 1.067 | 203.049 | 2.952 | 70,909 | 1.066 |
| 27 | Santiago ⊞ | 7.660 | 3.185 | 679 | 0.323 | 3.271 | 28,182 | 65.289 | 0.748 | 82.519 | 2.834 | 113,773 | 1.040 |
| 28 | Cape Town | 7.641 | 2.419 | 322 | 0.238 | 3.842 | 19,505 | 42.121 | 1.232 | 105.695 | 2.800 | 58,955 | 1.096 |
| 29 | Detroit ⊞ | 7.603 | 2.329 | 844 | 0.309 | 3.761 | 42,481 | 84.982 | 0.938 | 163.240 | 3.044 | 84,778 | 1.050 |
| 30 | Vancouver ⊞ | 7.588 | 2.934 | 481 | 0.389 | 2.383 | 14,955 | 38.452 | 1.574 | 144.460 | 2.835 | 33,404 | 1.058 |
| 31 | Sydney | 7.557 | 2.409 | 1,042 | 0.587 | 2.097 | 25,343 | 55.223 | 1.155 | 130.071 | 2.710 | 68,031 | 1.065 |
| 32 | Bangkok | 7.495 | 2.687 | 1,155 | 0.378 | 2.642 | 68,623 | 94.975 | 1.310 | 90.662 | 2.301 | 212,114 | 1.058 |
| 33 | San Francisco ⊞ | 7.489 | 2.904 | 753 | 0.474 | 2.154 | 23,471 | 49.414 | 1.088 | 134.944 | 2.876 | 55,946 | 1.079 |
| 34 | Boston | 7.487 | 3.207 | 950 | 0.364 | 2.784 | 36,370 | 81.069 | 1.115 | 142.139 | 2.716 | 82,966 | 1.080 |
| 35 | Tehran | 7.328 | 2.815 | 1,578 | 0.714 | 1.617 | 30,889 | 68.692 | 1.128 | 87.835 | 2.556 | 120,389 | 1.057 |
| 36 | Hamburg | 7.277 | 3.091 | 683 | 0.226 | 3.380 | 23,544 | 93.775 | 1.861 | 171.978 | 2.639 | 44,649 | 1.073 |
| 37 | Bogota ⊞ | 7.242 | 2.839 | 441 | 0.172 | 6.510 | 23,364 | 79.907 | 1.644 | 112.684 | 2.846 | 69,001 | 1.105 |
| 38 | Manila ⊞ | 7.241 | 3.139 | 553 | 0.288 | 7.162 | 34,497 | 59.789 | 1.798 | 86.407 | 2.703 | 123,099 | 1.068 |
| 39 | Ottawa ⊞ | 7.226 | 2.779 | 428 | 0.158 | 5.414 | 18,115 | 84.441 | 2.114 | 218.951 | 2.894 | 27,787 | 1.120 |
| 40 | Jakarta | 7.119 | 3.187 | 1,225 | 0.499 | 2.634 | 64,246 | 76.387 | 0.835 | 66.800 | 2.534 | 289,414 | 1.069 |
| 41 | Athens | 7.117 | 3.426 | 425 | 0.225 | 3.854 | 26,795 | 58.664 | 0.911 | 94.760 | 3.025 | 103,722 | 1.052 |
| 42 | Kuala Lumpur | 7.111 | 3.228 | 1,620 | 0.655 | 2.100 | 38,709 | 76.862 | 1.143 | 112.062 | 2.685 | 121,112 | 1.093 |
| 43 | Madrid | 7.097 | 3.231 | 1,833 | 0.816 | 1.359 | 23,899 | 69.853 | 0.877 | 109.540 | 2.949 | 96,307 | 1.058 |
| 44 | Brussels | 6.935 | 3.296 | 800 | 0.250 | 3.016 | 33,635 | 99.388 | 1.073 | 166.121 | 2.691 | 70,238 | 1.059 |
| 45 | Shenzhen | 6.868 | 3.322 | 1,798 | 0.777 | 1.244 | 23,228 | 71.971 | 1.546 | 172.305 | 2.969 | 57,318 | 1.077 |
| 46 | Kinshasa | 6.801 | 3.041 | 209 | 0.157 | 7.749 | 18,671 | 41.430 | 1.573 | 108.991 | 2.913 | 49,944 | 1.047 |
| 47 | Lagos | 6.696 | 2.708 | 439 | 0.212 | 5.108 | 40,577 | 64.431 | 1.538 | 115.473 | 2.589 | 107,039 | 1.050 |
| 48 | Dhaka | 6.604 | 3.121 | 780 | 0.260 | 4.226 | 29,445 | 93.380 | 1.788 | 150.168 | 2.628 | 60,194 | 1.080 |
| 49 | Rome | 6.434 | 3.937 | 741 | 0.261 | 3.309 | 24,886 | 88.435 | 1.244 | 149.841 | 2.689 | 61,535 | 1.083 |
| 50 | Barcelona ⊞ | 6.417 | 3.624 | 870 | 0.564 | 1.812 | 18,023 | 48.040 | 1.257 | 116.050 | 2.994 | 68,626 | 1.091 |
| 51 | Amsterdam | 6.362 | 3.555 | 898 | 0.361 | 2.642 | 29,170 | 77.353 | 1.101 | 110.819 | 2.763 | 91,230 | 1.085 |
| 52 | Moscow | 6.276 | 4.205 | 688 | 0.224 | 3.654 | 26,040 | 95.382 | 1.624 | 221.352 | 2.791 | 43,108 | 1.072 |
| 53 | Istanbul | 6.161 | 3.540 | 996 | 0.520 | 1.649 | 37,276 | 59.591 | 0.563 | 85.783 | 3.003 | 149,594 | 1.060 |
| 54 | Dubai ⊞ | 6.145 | 3.740 | 939 | 0.583 | 1.294 | 22,202 | 50.047 | 1.246 | 118.775 | 2.933 | 82,965 | 1.061 |
| 55 | Rio de Janeiro | 5.620 | 2.716 | 796 | 0.445 | 2.314 | 31,695 | 55.671 | 1.780 | 111.584 | 2.828 | 92,819 | 1.051 |
| 56 | Mumbai | 5.328 | 4.096 | 739 | 0.448 | 2.652 | 17,745 | 51.318 | 2.316 | 118.573 | 2.717 | 50,066 | 1.069 |

Table S1: **Complete City-level DiverCity Ranking.** The table presents all 56 cities ranked by their city-level DiverCity ($\mathcal{D}_C$). Metrics include interquartile range (IQR), total attractors length, attractors density, spatial homogeneity ($H$), total road network length, percentage of land area covered by roads (Land %), edge load, average edge length, average number of streets per node, total intersection count, and average circuity. A ⊞ symbol indicates a gridded road network structure.
